# Supplementary material for: Guidelines and Evaluation of Clinical Explainable AI in Medical Image Analysis
Source: arXiv:2202.10553 source file (2022-12-08)
Supplement: Supplementary file 2 [file S2.tex]

\documentclass{article}
\topmargin=-0.45in
\evensidemargin=0in
\oddsidemargin=0in
\textwidth=6.5in
\textheight=9.0in
\headsep=0.25in
\setlength{\parskip}{2pt}
\usepackage{indentfirst}
\date{}
\usepackage{color}
\usepackage{xcolor}
\usepackage[normalem]{ulem} %

\usepackage{fancyhdr}
\pagestyle{fancy}
\fancyhf{}
\lhead{}
\rfoot{}
\rhead{\thepage}

\definecolor{blue}{RGB}{17, 85, 204}

\renewcommand{\sout}[1]{\unskip}
\renewcommand{\redsout}[1]{\unskip}

\usepackage{float}
\usepackage[section]{placeins}

\usepackage{algorithm}
\usepackage[noend]{algpseudocode}
\usepackage{booktabs} %
\usepackage[colorlinks=true,linkcolor=blue]{hyperref}%
\usepackage{bbm}
\usepackage{amsmath,amsthm,amsfonts,amssymb,amscd}
\usepackage{csvsimple}
\usepackage{xcolor}
\usepackage[normalem]{ulem} %
\usepackage{array}
\usepackage{makecell} 
\newcommand{\PreserveBackslash}[1]{\let\temp=\\#1\let\\=\temp}
\newcolumntype{C}[1]{>{\PreserveBackslash\centering}p{#1}}
\newcolumntype{R}[1]{>{\PreserveBackslash\raggedleft}p{#1}}
\newcolumntype{L}[1]{>{\PreserveBackslash\raggedright}p{#1}}
\usepackage{rotating} %
\title{\textbf{Guidelines and Evaluation of Clinical Explainable AI in Medical Image Analysis}\\
\vspace{0.5em}
Supplementary Material S2: \\
Additional Literature Review, Method Details, Results, and Heatmap Visualizations
}
\author{Weina Jin\\
\and
Xiaoxiao Li\\
\and
Mostafa Fatehi\\
\and
Ghassan Hamarneh\\
}

\begin{document}

\maketitle
\footnotetext[1]{\copyright 2022. This manuscript version is made available under the CC-BY-NC-ND 4.0 license https://creativecommons.org/licenses/by-nc-nd/4.0/}

{
  \hypersetup{linkcolor=black}
  \tableofcontents
}

\section{Literature Review on Evaluation Objectives of Explanation}

To develop the Clinical XAI Guidelines, we reviewed technical literature on computational and human user study evaluations for explainable AI (XAI). The literature covers both AI and human-computer interaction (HCI) domains. We extracted non-overlapping evaluation objectives from technical literature, and summarized them in Table~\ref{tab:obj}.

The guidelines selected and prioritized the evaluation objectives based on clinical requirements from our user study. In Table~\ref{tab:obj}, although consistency and simulatability are important technical evaluation objectives, we did not include them in the guidelines, because they were not the main concerns to clinical users in our user study. Whenever necessary, the consistency objective can be used as an additional technical evaluation objective in addition to the Clinical XAI Guidelines. The simulatability objective may not have its clinical utility: as we discussed in the manuscript \S6.1.2, model prediction and its probability are \textit{known} information to the model, and are easily accessible to users. Therefore, it may not be well worth physicians' extra effort to interpret an explanation, and just to guess model's output from it without gaining any new information.
Guideline 2 Clinical relevance is not listed in Table~\ref{tab:obj}, because it is a clinical requirement and not mentioned in the technical literature.

\begin{table*}[!h]
    \centering
    \begin{tabular}{>{}L{4cm}|>{}L{7cm}|>{}L{4cm}}
       \toprule
       \textbf{Objective}  & \textbf{Definition} & \textbf{Reference}\\
       \toprule
$\star$ \textbf{Explanation audience} (G1 Understandability) & The required computational literacy to comprehend the explanation should fit audiences' background knowledge.
& \cite{Sokol2020, jin2021euca, Vaughan_2021}; U3.3: Making AI transparent
\\
\hline
$\star$ \textbf{Truthfulness}, faithfulness, or fidelity (G3) & The adherence of explanation to the underlying model. &\cite{jacovi-goldberg-2020-towards, Sokol2020, 10.5555/3305890.3306024, NEURIPS2019_a7471fdc, NEURIPS2018_294a8ed2,DBLP:journals/corr/abs-2104-08782,DBLP:conf/nips/HookerEKK19,7552539,Lundberg2020,10.5555/3327757.3327875, deyoung-etal-2020-eraser}; U2.3. Verifying AI decision, and calibrating trust\\
\hline
       $\star$ \textbf{Identification of errors, biases, or new patterns} (G4 Informative plausibility)  & The effect of explanation for end-tasks (such as identification of errors, biases, or new facts), compared with the baseline of human-produced explanation. & \cite{Doshi-Velez2018, jacovi-goldberg-2020-towards, Sokol2020, 10.1145/3387166};
U2. Clinical utility of explainable AI;
U5. Clinical assessment of explainable AI \\
       \hline

    $\star$ \textbf{Computational complexity} (G5 Computational efficiency)& The explanation algorithm should consider the constraints of time, memory, or computational power & \cite{Sokol2020}; U1.2.1: Decision support for time-sensitive cases
    \\
    \hline
\textbf{Consistency}, invariance, or robustness & 
For a fixed model, explanation of similar data points (with similar prediction outputs) should be similar. 
&\cite{Sokol2020, 10.5555/3305890.3306024, VILONE202189, DBLP:journals/corr/abs-1806-08049}\\
\hline
       \textbf{Simulatability} & Given an explanation, how well can humans simulate the model's output. & \cite{Doshi-Velez2018, Sokol2020, 10.1145/3236386.3241340, 10.1145/3387166, hase-bansal-2020-evaluating}\\
    \bottomrule
    \end{tabular}
    \caption{\textbf{Summary of XAI evaluation objectives in the technical literature}. $\star$ indicates an overlap between the technical evaluation objective and the Clinical XAI Guidelines.\\
    G - the Clinical XAI Guidelines, U - Physician user study findings (in Supplementary Material S1)}
    \label{tab:obj}
\end{table*}
\section{Review of the Evaluated Post-Hoc Heatmap Methods}\label{xai_method}
We select 16 commonly-used gradient- and perturbation-based heatmap methods. We give a brief review for each of them.

\subsection{Gradient- and Activation-Based Heatmap Methods}
\subsubsection*{CAM} CAM (Class Activation Mapping)~\cite{7780688} generates a heatmap for a prediction by aggregating the internal activations of a neural network layer and weighting each neuron's weights in that layer to the final decision layer.

\subsubsection*{Grad-CAM} It is similar to CAM but replaces the weights with gradients of the target prediction with respect to the activation map~\cite{8237336}. We only include Grad-CAM in our evaluation, because it does not require special model architecture as CAM does.

For activation-based methods including CAM and Grad-CAM, because the activation maps at a deeper layer could not reflect the modality-specific information, which is aggregated at the first convolutional layer, the output heatmap is a single-modality image, which is not modality-specific. We copy such a heatmap to all modalities to compare it with other methods.

\subsubsection*{Gradient} It reflects how quickly the output changes when input changes~\cite{simonyan2014deep}.

\subsubsection*{Input $\times$ Gradient} It multiplies the input by the gradient signal to obtain a first-order Taylor approximation~\cite{shrikumar2017just}.
Compared with Gradient, it tends to produce sharper heatmaps. Since \cite{shrikumar2017just} showed layer-wise relevance propagation (LRP) is equivalence to Input $\times$ Gradient when all activations are piece-wise linear and biases are included, we only include Input $\times$ Gradient in the evaluation.

\subsubsection*{SmoothGrad} It smooths the noisy gradient signals by averaging the heatmaps for an input and its random neighborhood samples~\cite{smilkov2017smoothgrad}.

\subsubsection*{Deconvolution} It modifies the gradient computation rule at ReLU activation function. Instead of back-propagating non-negative \textit{input} gradients as in the vanilla Gradient method, Deconvolution only back-propagates non-negative \textit{output} gradients~\cite{10.1007/978-3-319-10590-1_53}. 

\subsubsection*{Guided Backpropagation} It combines Gradient and Deconvolution methods by back-propagating \textit{input} and \textit{output} gradients that are both non-negative~\cite{springenberg2015striving}. 

\subsubsection*{Guided Grad-CAM} It  computes the element-wise product between Guided Backpropagation and the up-sampled \& broadcasted Grad-CAM signal~\cite{8237336}.

\subsubsection*{Integrated Gradient} It approximates the path integral of gradients along the straight line from a neutral baseline input to the target input~\cite{10.5555/3305890.3306024}.

\subsubsection*{DeepLIFT} It explains the prediction difference from an uninformative baseline by introducing difference-from-reference operation in the backpropagation rule~\cite{10.5555/3305890.3306006}. DeepLIFT and Integrated Gradients both address the gradient ``saturation'' problem, and DeepLIFT is faster than Integrated Gradient as it only needs one backward pass to compute the explanation.

\subsubsection*{Gradient SHAP} It approximates Shapley values by computing the expectation of gradients~\cite{NIPS2017_8a20a862}.

\subsection{Perturbation-Based Heatmap Methods}

\subsubsection*{Occlusion} It occludes part of the image with a sliding window, and averages the output differences as the feature attribution~\cite{10.1007/978-3-319-10590-1_53,DBLP:conf/iclr/ZintgrafCAW17}. In our implementation, the occlusion is done modality-wise to generate heatmaps that are modality specific. The occluded regions are replaced by values drawn from a normal distribution with the same mean and standard deviation of the given input modality. We experimented with different sizes of sliding window and stride to balance heatmap resolution and computational time.

\subsubsection*{Feature Ablation} It is similar to Occlusion, but occludes the individual image features rather than using a sliding window. In our implementation, we use modality-wise superpixel segmentation masks as the image features to generate modality-specific heatmaps, and replace the ablated feature with baseline value of $0$s.

\subsubsection*{Feature Permutation}It replaces image feature by shuffling the feature values within a batch, and computes the prediction difference accordingly~\cite{JMLR:v20:18-760}. 

\subsubsection*{LIME} LIME (local interpretable model-agnostic explanation) learns an interpretable model by perturbing and sampling the neighbor data points around the input~\cite{10.1145/2939672.2939778}. 

\subsubsection*{Shapley Value Sampling} It relies on the concept of a feature's Shapley value, which is the average marginal feature attribution across all possible feature combination subsets~\cite{RM-670-PR}. Shapley Value Sampling is an efficient sampling method to overcome the expensive enumeration of all possible feature combinations~\cite{CASTRO20091726}.

\subsubsection*{Kernel SHAP} It uses the LIME framework to compute Shapley values~\cite{NIPS2017_8a20a862}. Since it only receives one superpixel feature segmentation mask that is shared across modalities, the produced heatmaps are \textit{not} modality-specific.

\section{Method}
\subsection{Data}

The multi-modal images in BraTS dataset are pre-registered and pre-processed. The BraTS dataset includes tumor grade labels of lower-grade (LGG) and high-grade gliomas (HGG)
(with the number of cases of LGG: HGG = 76: 293), and tumor segmentation masks. The tumor/feature segmentation masks contain several labels of the whole tumor, or each sub-region of necrotic tumor core, edema, and GD-enhancing areas. In our evaluation, we focus on the single segmentation mask of the whole tumor, which covers the region of all other feature masks.

\subsection{Model Training and Performance}

For the BraTS dataset, we built a VGG-like 3D CNN that receives multi-modal 3D MR images $X \in \mathbb{R}^{4 \times 240 \times 240 \times 155}$, where 4 is the number of MRI modalities, and 240, 240, 155 are width, height, and depth respectively. We split the data into a training, validation, and test set with a 65\%, 15\%, 20\% split ratio. We trained five models using the same training scheme and train/validation dataset, by only varying the random seed for model parameter initialization.
We used a weighted sampler to handle the imbalanced data. The models were trained with a learning rate $= 0.0005$, batch size = 4, and training epoch of 45, 66, 54, 87, 46 for each model selected by the accuracy of validation data.
The average accuracy of the five models is 
0.89 $\pm$ 0.02 (Table~\ref{tab:brats_perf}, Fig.~\ref{fig:acc_brain}).

For the synthetic brain tumor dataset, we first fitted a classification model to the synthesized brain images by fine-tuning the pre-trained DenseNet121 that receives 2D multi-modal MRI input slices of $X \in \mathbb{R}^{4 \times 256 \times 256}$, where 4 is the number of MRI modality, and 256 and 256 are the image width and height. The number of cases of  LGG:HGG=1:1.
We used the same training strategies as the BraTS dataset. The model achieves $95.70 \pm 0.06\%$ accuracy on the test set. The heatmaps are generated on a test set with the same ground-truth alignment probability as its training set.  

We used PyTorch\footnote{\href{http://pytorch.org}{http://pytorch.org}} and MONAI API\footnote{\href{http://monai.io}{http://monai.io}} for model training, and Captum\footnote{\href{http://captum.ai}{http://captum.ai}} to generate post-hoc heatmaps.  
To train the models and generate heatmaps, we used a computer with 1 GTX Quadro 24 GB GPU and 8 CPU cores, and a SLURM\footnote{\href{https://slurm.schedmd.com/overview.html}{https://slurm.schedmd.com/overview.html}} based high performance computing cluster with jobs configured to use no more than a minimum of 1 GPU, and 8 cores CPU each with 128 RAM.
\begin{table}[!ht]
    \centering
    \begin{tabular}{l|l|l|l|l|l|l}
    \toprule
    Accuracy & Mean$\pm$Std &    Model 1 & Model 2 & Model 3 & Model 4 & Model 5 \\
    \hline
     Train & 0.9306 $\pm$ 0.0244 &
0.9208 & 0.9375 & 0.9278 & 0.9708 & 0.8958  \\
     Validation & 0.9464 $\pm$ 0.0160 &
0.9286 & 0.9464 & 0.9643 & 0.9643 & 0.9286 \\
     Test & 0.8946 $\pm$ 0.0199 & 0.8784 & 0.9189 & 0.9054 & 0.9054 & 0.8649 \\
     \hline
    Train epochs & & 45 &66&54&87 &46\\

     \bottomrule
    \end{tabular}
    \caption{\textbf{Model performance of five models on glioma grading prediction on BraTS dataset}. Models were trained on the same training dataset and selected by validation set, and differ by their random parameter initialization.}
    \label{tab:brats_perf}
\end{table}

\begin{figure}[H]
    \centering
    \includegraphics[width=0.99\linewidth]{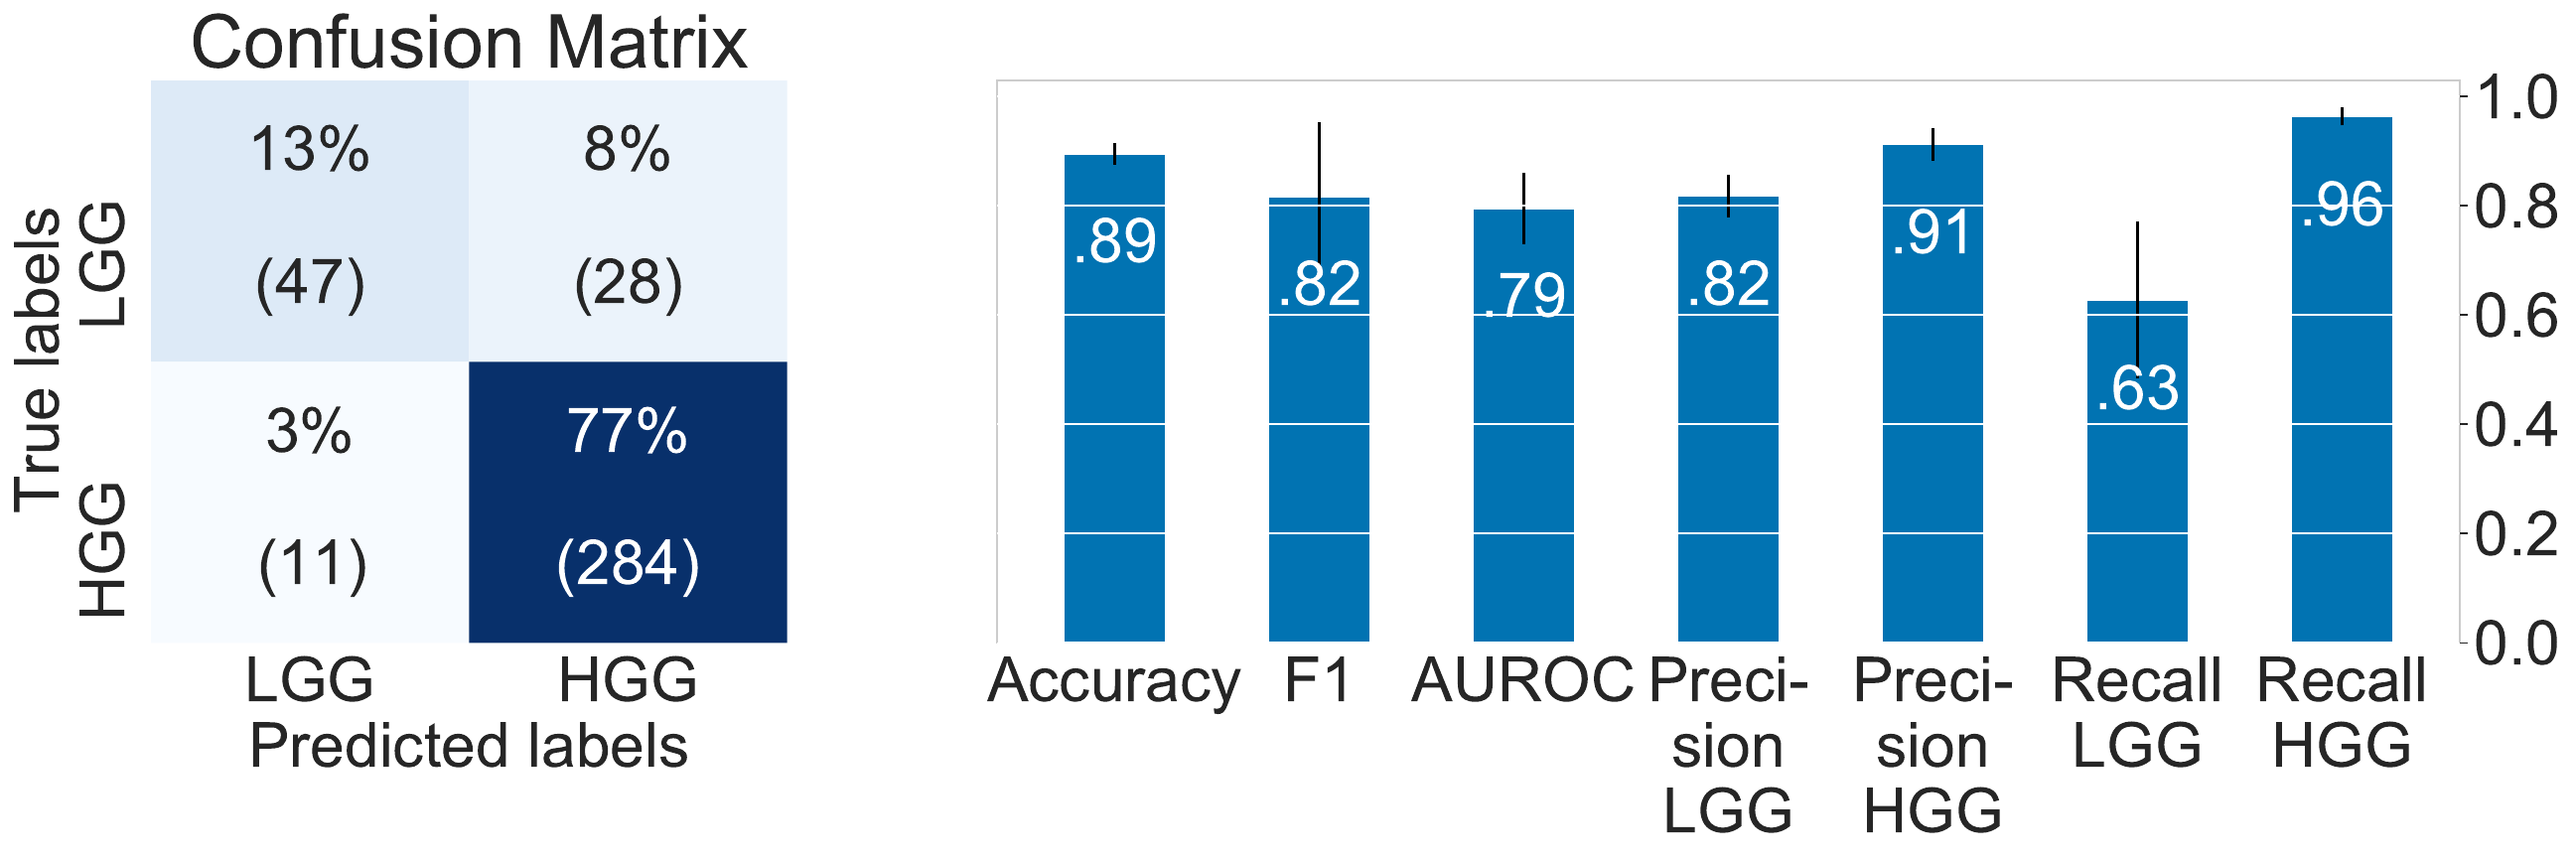}
    \caption{\textbf{Model performance of five models on glioma grading prediction on BraTS dataset}. Left: Aggregated confusion matrix of test performance from the five models. Right: Mean and standard deviation of the model performance metrics.}
    \label{fig:acc_brain}
\end{figure}

\begin{table}[!h]
    \centering
    \begin{tabular}{l|l|l|l|l|l|l}
    \toprule
    AUC & Mean$\pm$Std&   Model 6 & Model 7 & Model 8 & Model 9 & Model 10 \\
    \hline
     Train    & 0.9896 $\pm$ 0.0078 & 0.9782 & 0.9822& 0.9959 &0.9962 & 0.9954 \\
     Validation & 0.8395 $\pm$ 0.0107 & 0.8510 & 0.8288 & 0.8291 & 0.8534 & 0.8353 \\
     Test  &0.7934 $\pm$ 0.0162 & 0.7859 &0.7803 & 0.8230 &0.7981 &0.7797 \\
     \bottomrule
    \end{tabular}
    \caption{\textbf{Model performance of five knee MRI models.} All models were trained on the same training dataset for 27 epochs, and differed by their random parameter initialization. We number them 6-10 to differentiate them with the glioma models 1-5.}
    \label{tab:perf_knee}
\end{table}
\FloatBarrier

\begin{figure}[!h]
    \centering
    \includegraphics[width=0.99\linewidth]{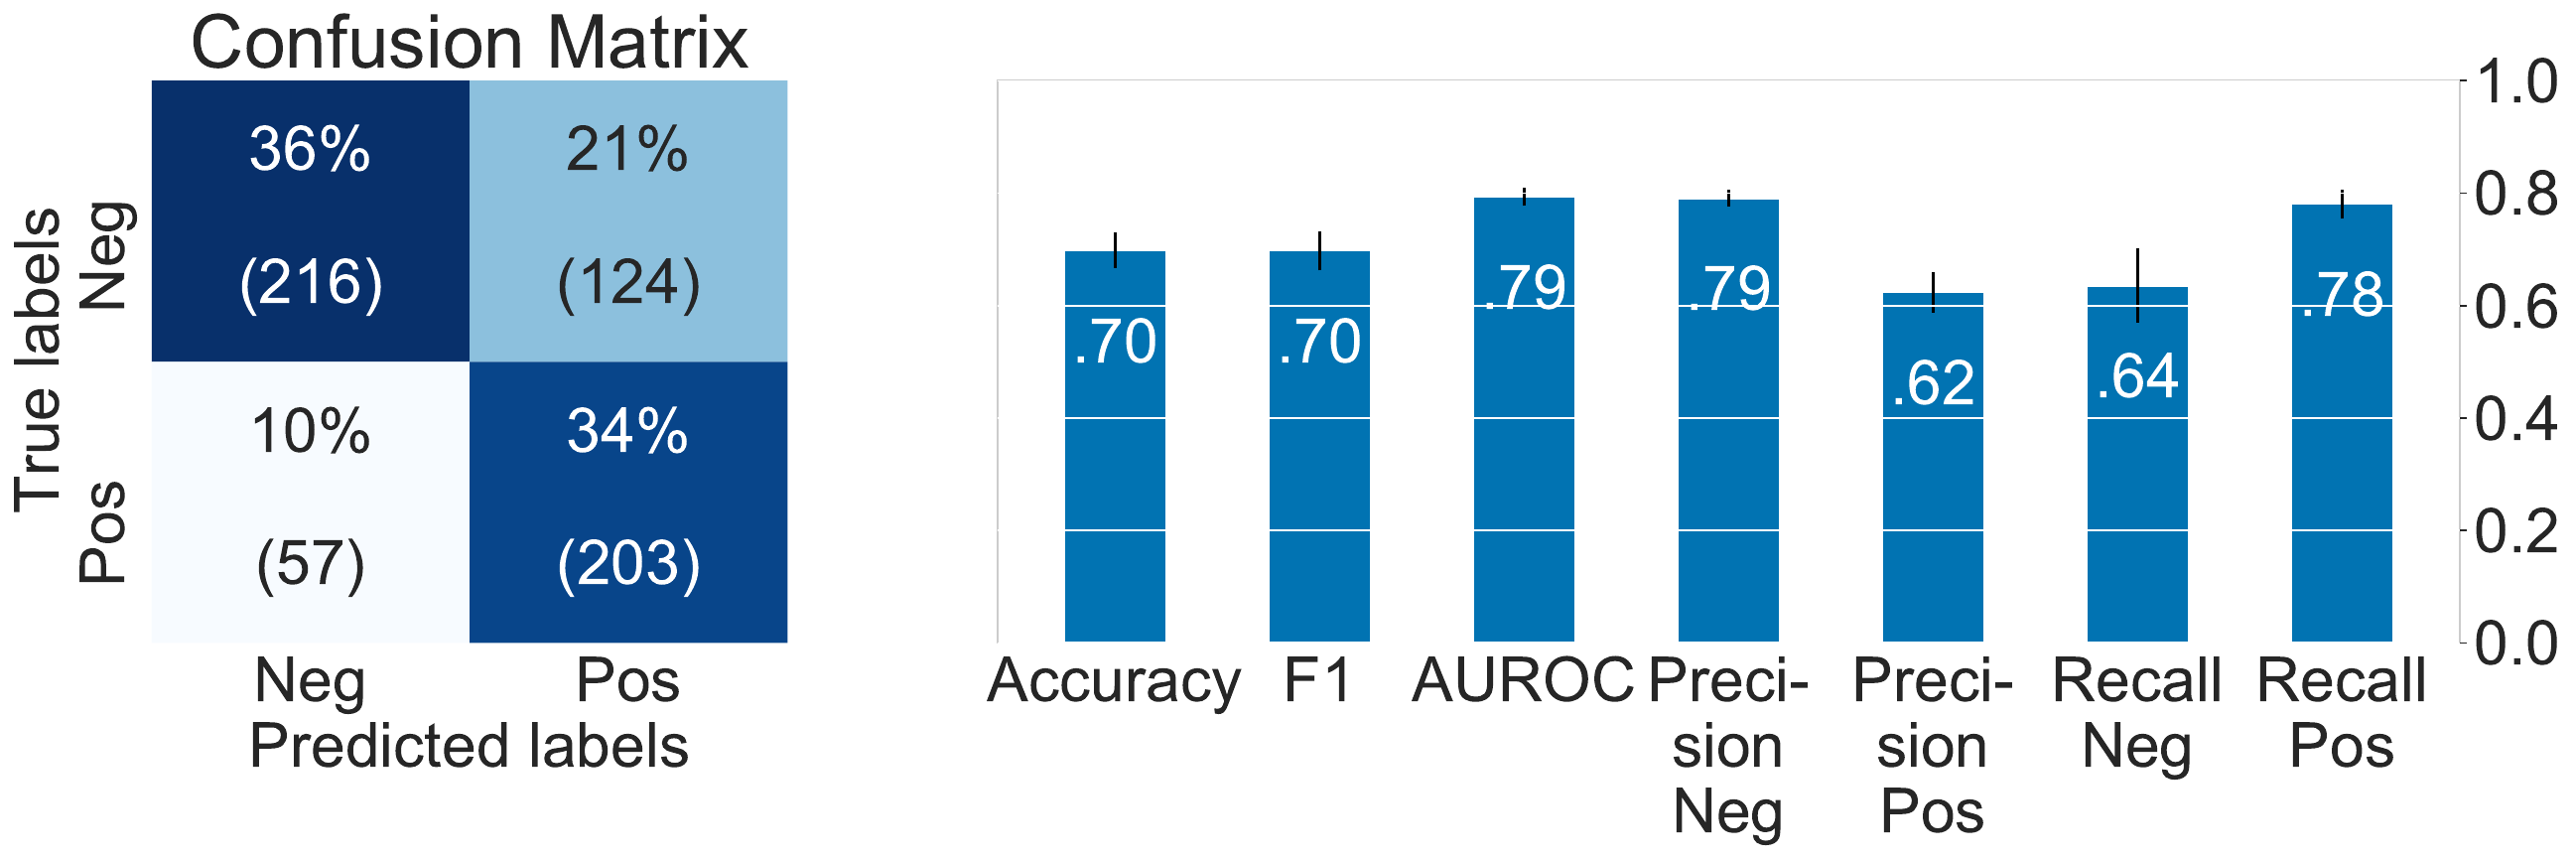}
    \caption{\textbf{Model performance of five knee MRI models}. The positive label is meniscus tear, and the negative label is intact. Left: Aggregated confusion matrix of testing performance from the five models. Right: Mean and standard deviation of the model performance metrics.}
    \label{fig:acc_knee}
\end{figure}
\FloatBarrier

\begin{figure}[!h]
    \centering
    \includegraphics[width=0.8\linewidth]{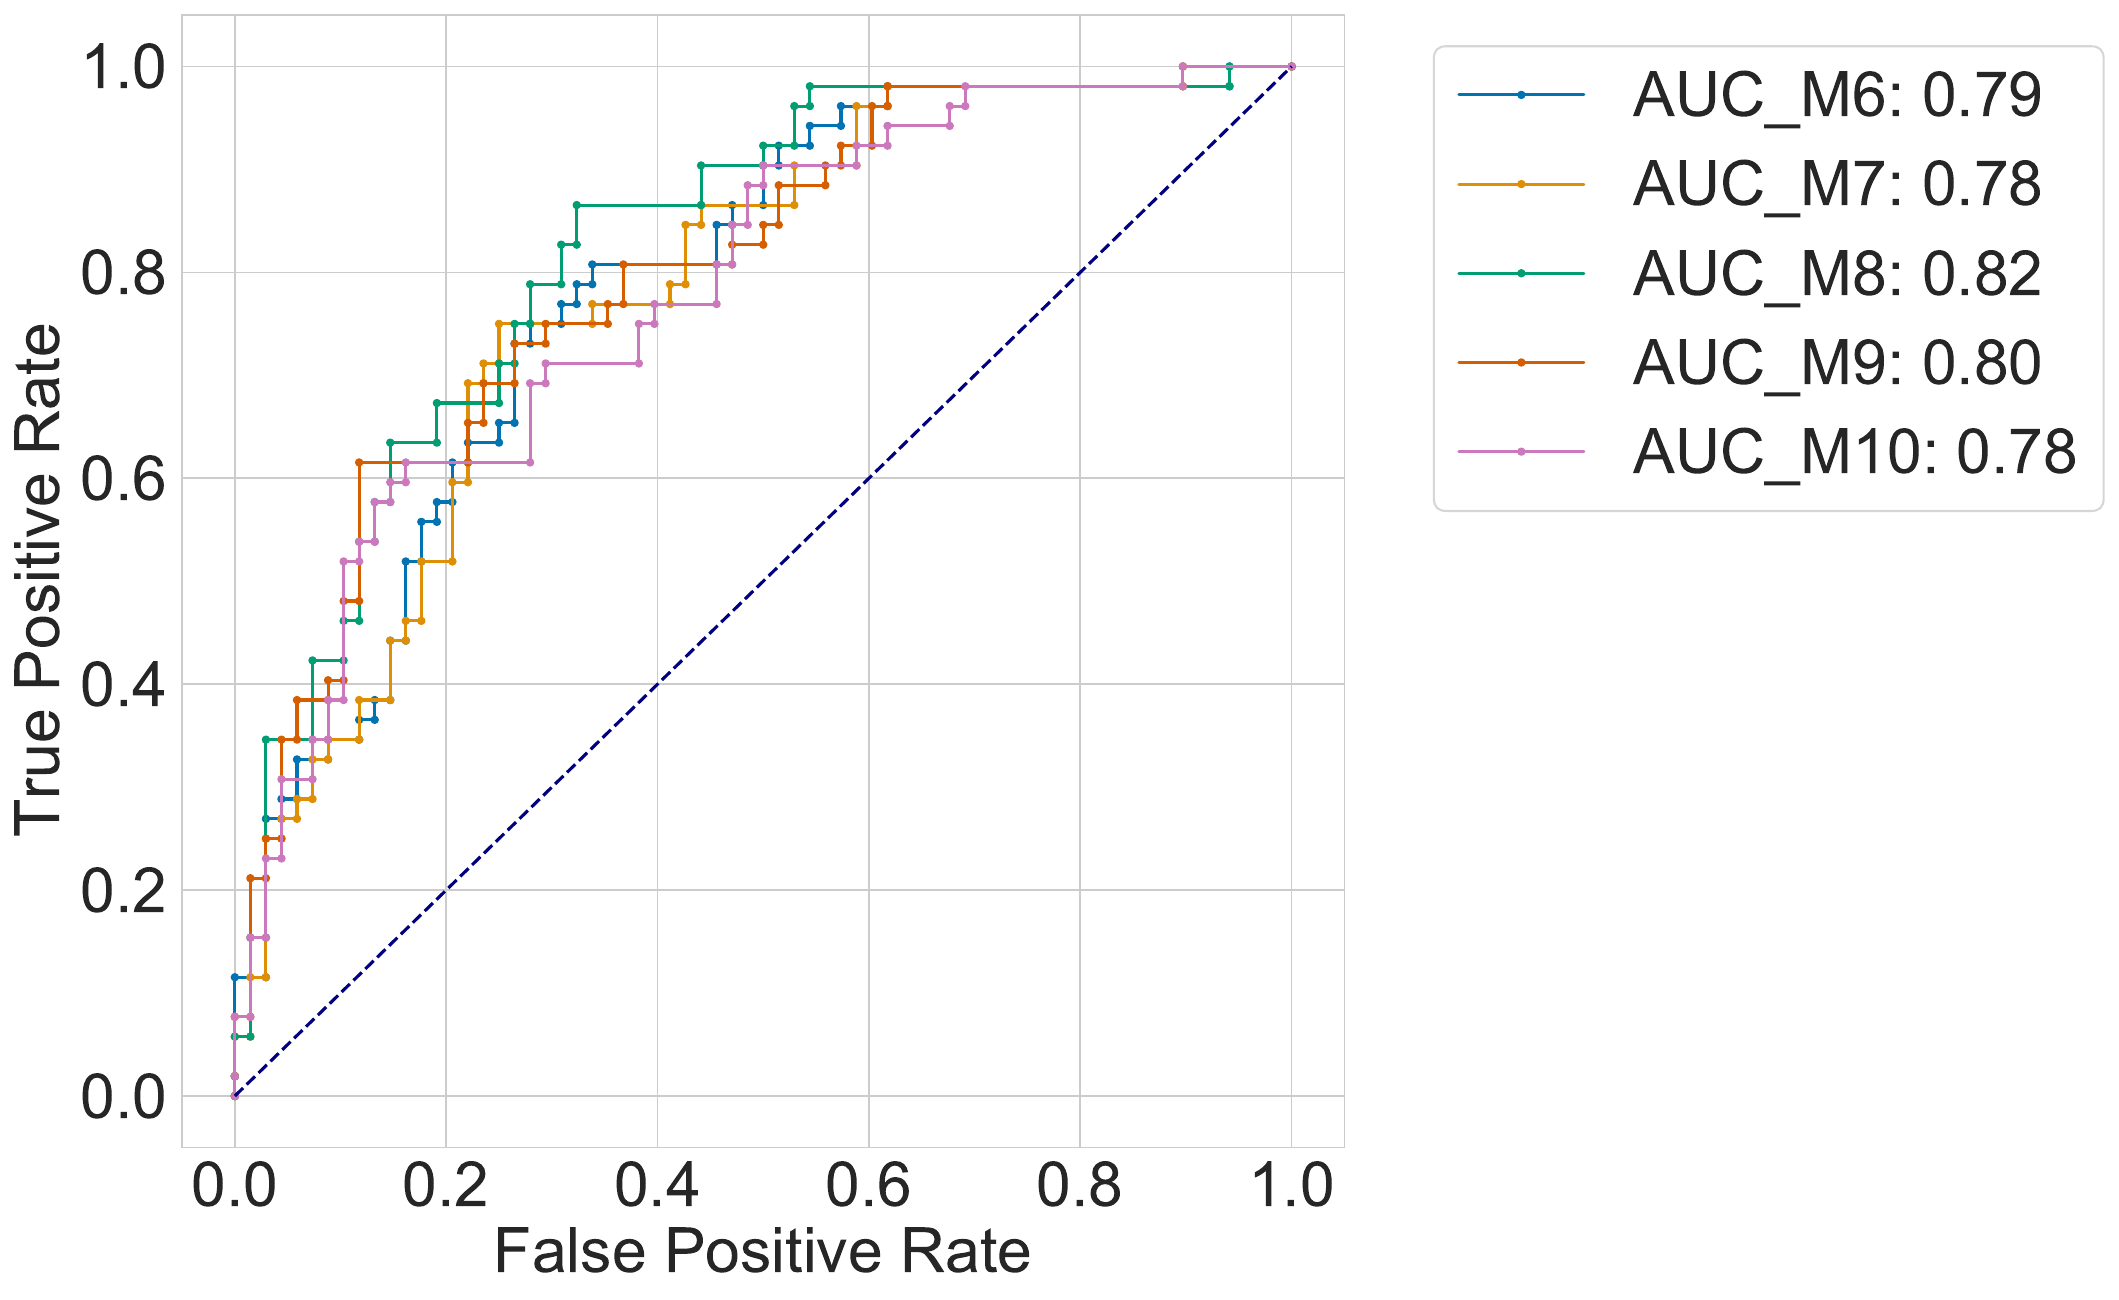}
    \caption{\textbf{Model performance receiver operating characteristic (ROC) curves of five knee MRI models}. Model 6-10 and their area under the curve (AUC) are shown in the legend.}
    \label{fig:acc_knee}
\end{figure}
\FloatBarrier
\subsection{Post-Processing Heatmaps} \label{postproc}
Before evaluating and visualizing the heatmaps, we post-processed them by first capping the top 1\% outlying values (following~\cite{smilkov2017smoothgrad}). We focused on the positive values of the heatmaps as they are interpreted as evidence towards the model decision (a.k.a. importance scores). Since the negative values in the heatmaps may carry different meanings for different XAI algorithms, and since it is difficult for end-users to understand and interpret the negative values from our pilot study, in the evaluation pipeline, except for the visualization, we ignored the negative values by setting them to $0$.
We then scaled the values of the heatmaps to $[0,1]$, and applied a Gaussian kernel to visually smoothen the heatmaps.

\subsection{G3 Truthfulness: Cumulative Feature Removal}\label{acc_drop}

In the cumulative feature removal experiment, to replace the removed features with null values that aims to not change the distribution of the input and not introduce new information, common approaches of feature replacement include replacing with zero~\cite{ancona2018towards}, mean~\cite{Lundberg2020}, random~\cite{7552539}, neighbor value~\cite{DBLP:conf/iclr/ZintgrafCAW17, DBLP:journals/corr/abs-2004-00668}, or a generated input~\cite{frye2021shapley, DBLP:journals/corr/abs-2105-10719}. Since there is no consensus on the choice of feature replacement approach, we utilized two approaches: (1) replacing the removed features with a constant value: for the glioma task, the constant value is 0 to be the same with the blank background; for the knee task, the constant value is a modality mean. (2) replacing with random unimportant values: the unimportant values are defined by the lower 1\% quantile of positive values in a heatmap. 
The cumulative feature removal procedure is shown in Algorithm~\ref{algo:diffauc}.

\begin{algorithm*}
    \caption{Cumulative Feature Removal}\label{euclid}
    \hspace*{\algorithmicindent} \textbf{Input} test dataset $D$, a trained model $M$, a heatmap method $\mathcal{H}$ \\
    \hspace*{\algorithmicindent} \textbf{Output} $\text{$\Delta$AUPC}(x)$, and two lists to record performance metrics during feature removal, $S_\mathcal{H}$ for heatmap method $\mathcal{H}$, $S_{\mathcal{H}_b}$ for random baseline $\mathcal{H}_b$.   
    \begin{algorithmic}[1]
    \Procedure{CumulativeFeatureRemoval}{steps = 10}
    \State $S_\mathcal{H} \gets \{\}$
    \State $S_{\mathcal{H}_b} \gets \{\}$
    \State $\text{Heatmaps} \gets \text{GenerateHeatmaps}(D, M, \mathcal{H})$
    \State $\text{HeatmapBaselines} \gets \text{RandomPermutation}(\text{Heatmaps})$
    \For{$i$ in (0, \text{steps}, $i++$)}
    \State $q \gets 100- i \times 100/steps$
    \State $\text{AblationMask} \gets \text{GetTopQuantileMaskFromHeatmaps}(\text{Heatmaps}, q)$
    \State $\text{AblatedInput} \gets \text{MaskInput}(D, \text{AblationMask})$ 
    \State $\text{Accuracy} \gets \text{GetModelPerformance}(M, \text{AblatedInput})$
    \State $S_\mathcal{H} \gets S_\mathcal{H} + \text{Accuracy}$
    \State $\text{AblationMaskBaseline} \gets \text{GetTopQuantileMaskFromHeatmaps}(\text{HeatmapBaselines}, q)$
    \State $\text{AblatedInputBaseline} \gets \text{MaskInput}(D, \text{AblationMaskBaseline})$ 
    \State $\text{AccuracyBaseline} \gets \text{GetModelPerformance}(M, \text{AblatedInputBaseline})$
    \State $S_{\mathcal{H}_b} \gets S_{\mathcal{H}_b} + \text{AccuracyBaseline}$
    \EndFor
    \State $ \text{AUPC}(\mathcal{H}) \gets \text{PlotFeaturePerturbationCurveAndGetAUPC}(S_{\mathcal{H}})$
    \State $ \text{AUPC}(\mathcal{H}_b) \gets \text{PlotFeaturePerturbationCurveAndGetAUPC}(S_{\mathcal{H}_b})$

    \State $\text{$\Delta$AUPC}(\mathcal{H}) = \text{AUPC}(\mathcal{H}_b) - \text{AUPC}(\mathcal{H})$
    \EndProcedure
    \end{algorithmic}
    \label{algo:diffauc}
\end{algorithm*}

\begin{figure*}[h]
    \centering
    \includegraphics[width=0.9\linewidth]{fig/Screen Shot 2021-09-12 at 1.08.16 AM.png}
    \caption{
    \textbf{Difference between the two plausibility metrics, intersection over union (IoU) and feature portion (FP)}. Both metrics compare a heatmap with the ground truth mask. The gray areas are used in the metric calculation. While IoU penalizes for both false positives and false negatives, FP is positive predictive value that only penalizes for false positives.}
    \label{fig:iou_fp}
\end{figure*}

\begin{figure}[!htb]
    \centering
    \includegraphics[width=1\linewidth]{fig/G1 card sorting_cameraReady.pdf}
    \caption{Sketches of different explanation forms (based on \cite{jin2021euca}) for the user study evaluation on G1 Understandability. The neurosurgeon was instructed to focus on the forms of explanation, as the contents of explanation were fictitiously made for the neuro-oncological task.
    }
    \label{fig:card}
\end{figure}
\FloatBarrier

\section{Result}

\subsection{G3 Truthfulness: Modality Importance (MI)}
The ground-truth modality importance Shapley values for each model are shown in Table~\ref{tab:mod_shapley} for the glioma task, and Table~\ref{tab:mod_shapley_knee} for the knee task. Both five models are similar in their most important modalities for prediction. For the glioma task, the important modalities are T1C and Flair, which align with human prior knowledge in interpreting MRI on the glioma task. For the knee task, all models prioritize the axial modality, which deviates from physicians' prior knowledge that mainly relies on sagittal and coronal views to identify knee lesions. 

The model-wise MI correlation performance is reported in Table~\ref{tab:mi_corr}. 

\begin{table}[!h]
    \centering
    \begin{tabular}{l|rrrrr}
    \toprule
     Glioma Modality & Model 1 & Model 2& Model 3 & Model 4 & Model 5    \\
     \midrule
     T1     & 0.032 & 0.026& 0.037 &0.059 &0.053\\
     T1C& \textit{0.164}  & \textit{0.082} & \textbf{0.444} & \textit{0.284} &\textit{0.319}\\
     T2 & 0.007 & -0.003 &-0.030 &0.009 & -0.046\\
     FLAIR & \textbf{0.473} & \textbf{0.611} & \textit{0.251} &\textbf{0.351} &\textbf{0.337}\\
     \bottomrule
    \end{tabular}
    \caption{\textbf{Modality importance ground truth Shapley value $\varphi_m$ for each model on the glioma task}. The first and second important modalities are bolded and italicized respectively. 
    }
    \label{tab:mod_shapley}
\end{table}

\begin{table}[!h]
    \centering
    \begin{tabular}{l|rrrrr}
    \toprule
     Knee Modality & Model 6 & Model 7& Model 8 & Model 9 & Model 10    \\
     \midrule
     Axial     & \textbf{0.113} & \textbf{0.103}& \textbf{0.119} &\textbf{0.128} &\textbf{0.121}\\
     Sagittal& \textit{0.104}  & 0.078 & \textit{0.117} & \textit{0.115} &\textit{0.090}\\
     Coronal & 0.069 & \textit{0.084} & 0.072 &0.069 &0.069\\
     \bottomrule
    \end{tabular}
    \caption{\textbf{Modality importance ground truth Shapley value $\varphi_m$ for each model on the knee task}. The first and second important modalities are bolded and italicized, respectively. 
    }
    \label{tab:mod_shapley_knee}
\end{table}

\begin{table*}[!h]

    \centering
    \resizebox{\textwidth}{!}{\begin{tabular}{m{0.2\linewidth} *{6}{>{\centering\arraybackslash}m{0.12\linewidth}}|
    *{6}{>{\centering\arraybackslash}m{0.12\linewidth}}
    }
    \toprule
     & \multicolumn{6}{c}{MI correlation: \textbf{Glioma}} & \multicolumn{6}{c}{MI correlation: \textbf{Knee}}\\
\cmidrule(lr){2-7}
\cmidrule(lr){8-13}
     & Model 1 & Model 2 & Model 3 & Model 4 & Model 5 & All & Model 6 & Model 7 & Model 8 & Model 9 & Model 10 & All\\
\hline

\hspace{0pt}Deconvolution &  -0.02$\pm$0.10 &  0.33$\pm$0.00 &  0.67$\pm$0.00 &  \textbf{ 0.67$\pm$0.00 } &  0.67$\pm$0.00 &  0.46$\pm$0.28 &  -1.00$\pm$0.00 &  -0.85$\pm$0.28 &  -0.30$\pm$0.15 &  -0.55$\pm$0.31 &  0.33$\pm$0.00 &  -0.47$\pm$0.51 &  \\ \hline 

\hspace{0pt}DeepLift &  \textbf{ 0.63$\pm$0.32 } &  0.45$\pm$0.38 &  0.85$\pm$0.29 &  0.49$\pm$0.29 &  0.59$\pm$0.23 &  0.60$\pm$0.33 &  NaN & NaN & NaN & NaN & NaN & NaN
\\ \hline 

\hspace{0pt}FeatureAblation &  0.39$\pm$0.45 &  0.50$\pm$0.49 &  0.67$\pm$0.38 &  0.63$\pm$0.38 &  \textbf{ 0.81$\pm$0.29 } &  0.60$\pm$0.43 &  -0.36$\pm$0.56 &  -0.07$\pm$0.54 &  \textbf{ 0.25$\pm$0.63 } &  \textbf{ 0.40$\pm$0.51 } &  0.02$\pm$0.66 &  0.05$\pm$0.64 &  \\ \hline 

\hspace{0pt}FeaturePermutation &  NaN &  NaN &  NaN &  NaN &  NaN &  NaN &  NaN & NaN & NaN & NaN & NaN & NaN
\\ \hline 

\hspace{0pt}GradCAM &  NaN &  NaN &  NaN &  NaN &  NaN &  NaN &  NaN & NaN & NaN & NaN & NaN & NaN
\\ \hline 

\hspace{0pt}Gradient &  0.22$\pm$0.24 &  0.37$\pm$0.59 &  0.78$\pm$0.28 &  0.50$\pm$0.33 &  0.60$\pm$0.26 &  0.49$\pm$0.41 &  -0.96$\pm$0.16 &  -0.34$\pm$0.06 &  -0.57$\pm$0.36 &  -1.00$\pm$0.00 &  0.27$\pm$0.26 &  -0.52$\pm$0.51 &  \\ \hline 

\hspace{0pt}GradientShap &  \textbf{ 0.63$\pm$0.29 } &  0.47$\pm$0.36 &  \textbf{ 0.90$\pm$0.25 } &  0.53$\pm$0.26 &  0.65$\pm$0.20 &  \textbf{  0.64$\pm$0.31 } &  -0.54$\pm$0.32 &  -0.33$\pm$0.12 &  -0.29$\pm$0.22 &  -0.78$\pm$0.36 &  \textbf{ 0.47$\pm$0.51 } &  -0.29$\pm$0.54 &  \\ \hline 

\hspace{0pt}GuidedBackProp &  0.48$\pm$0.34 &  0.33$\pm$0.00 &  0.70$\pm$0.10 &  \textbf{ 0.67$\pm$0.00 } &  0.67$\pm$0.00 &  0.57$\pm$0.21 &  -1.00$\pm$0.00 &  -0.54$\pm$0.31 &  -0.24$\pm$0.23 &  -0.78$\pm$0.32 &  0.36$\pm$0.13 &  -0.44$\pm$0.53 &  \\ \hline 

\hspace{0pt}GuidedGradCAM &  0.45$\pm$0.37 &  0.33$\pm$0.00 &  0.70$\pm$0.10 &  \textbf{ 0.67$\pm$0.04 } &  0.66$\pm$0.04 &  0.56$\pm$0.23 &  NaN & NaN & NaN & NaN & NaN & NaN
\\ \hline 

\hspace{0pt}InputXGradient &  \textbf{ 0.63$\pm$0.31 } &  \textbf{ 0.51$\pm$0.29 } &  \textbf{ 0.86$\pm$0.23 } &  0.55$\pm$0.30 &  0.66$\pm$0.18 &  \textbf{  0.64$\pm$0.29 } &  -0.68$\pm$0.33 &  -0.33$\pm$0.06 &  -0.35$\pm$0.16 &  -0.91$\pm$0.23 &  \textbf{ 0.50$\pm$0.41 } &  -0.35$\pm$0.55 &  \\ \hline 

\hspace{0pt}IntegratedGradients &  \textbf{ 0.63$\pm$0.30 } &  0.47$\pm$0.35 &  \textbf{ 0.90$\pm$0.25 } &  0.52$\pm$0.26 &  0.63$\pm$0.18 &  \textbf{  0.63$\pm$0.31 } &  \textbf{ 0.71$\pm$0.38 } &  -0.40$\pm$0.24 &  0.12$\pm$0.53 &  0.06$\pm$0.70 &  \textbf{ 0.71$\pm$0.46 } &  \textbf{  0.24$\pm$0.64 } &  \\ \hline 

\hspace{0pt}KernelShap &  NaN &  NaN &  NaN &  NaN &  NaN &  NaN &  \textbf{ -0.11$\pm$0.55 } &  \textbf{ 0.07$\pm$0.58 } &  \textbf{ 0.59$\pm$0.46 } &  \textbf{ 0.71$\pm$0.37 } &  0.37$\pm$0.49 &  \textbf{  0.33$\pm$0.58 } &  \\ \hline 

\hspace{0pt}Lime &  0.55$\pm$0.42 &  0.46$\pm$0.50 &  0.64$\pm$0.34 &  0.53$\pm$0.40 &  \textbf{ 0.70$\pm$0.39 } &  0.57$\pm$0.42 &  \textbf{ -0.09$\pm$0.52 } &  \textbf{ 0.07$\pm$0.56 } &  \textbf{ 0.63$\pm$0.46 } &  \textbf{ 0.69$\pm$0.39 } &  \textbf{ 0.46$\pm$0.50 } &  \textbf{  0.35$\pm$0.58 } &  \\ \hline 

\hspace{0pt}Occlusion &  0.48$\pm$0.45 &  \textbf{ 0.57$\pm$0.55 } &  0.43$\pm$0.38 &  \textbf{ 0.65$\pm$0.45 } &  \textbf{ 0.78$\pm$0.31 } &  0.58$\pm$0.45 &  -0.69$\pm$0.33 &  \textbf{ -0.03$\pm$0.47 } &  -0.34$\pm$0.47 &  -0.34$\pm$0.50 &  -0.18$\pm$0.65 &  -0.32$\pm$0.54 &  \\ \hline 

\hspace{0pt}ShapleyValueSampling &  0.60$\pm$0.43 &  \textbf{ 0.53$\pm$0.42 } &  0.66$\pm$0.27 &  0.43$\pm$0.26 &  \textbf{ 0.70$\pm$0.37 } &  0.59$\pm$0.37 &  \textbf{ 0.09$\pm$0.46 } &  \textbf{ 0.02$\pm$0.41 } &  \textbf{ 0.56$\pm$0.47 } &  \textbf{ 0.74$\pm$0.33 } &  0.33$\pm$0.44 &  \textbf{  0.35$\pm$0.50 } &  \\ \hline 

\hspace{0pt}SmoothGrad &  0.50$\pm$0.22 &  \textbf{ 0.96$\pm$0.11 } &  \textbf{ 0.91$\pm$0.15 } &  0.56$\pm$0.16 &  0.69$\pm$0.13 &  \textbf{  0.72$\pm$0.24 } &  -1.00$\pm$0.00 &  -0.92$\pm$0.21 &  -0.15$\pm$0.55 &  -0.42$\pm$0.23 &  0.33$\pm$0.00 &  -0.43$\pm$0.57 &  \\ 

\bottomrule
    \end{tabular}}
    \caption{\textbf{Model-wise evaluation results on Guideline 3 Truthfulness - MI correlation.} It shows MI correlation performances (mean $\pm$ std) of each model on the glioma (left half) and knee task (right half). For each column, we highlight MI correlation for the top three XAI methods in bold.
    }
    \label{tab:mi_corr}
\end{table*}

\subsection{G3 Truthfulness: Cumulative Feature Removal}

We report model-wise evaluation results on $\Delta$AUPC performance in Table~\ref{tab:aupc_brain} for the glioma task, and Table~\ref{tab:aupc_knee} for the knee task. The two feature replacement approaches (replacing the removed features with a constant value, or a random unimportant value, as described in \S\ref{acc_drop}) are listed in the tables. 
We test the correlation between the two feature replacement approaches using Kendall’s Tau-b ranking correlation on the average $\Delta$AUPC values of all five models (M $\pm$ SD column in Table~\ref{tab:aupc_brain} and \ref{tab:aupc_knee}). The two feature replacement approaches are highly correlated on both the glioma task ($\tau_b = 0.80$, $p < 0.001$), and the knee task ($\tau_b = 0.79$, $p < 0.001$).

We visualized the $\Delta$AUPC results in Fig.~\ref{fig:acc_drop_perf}. We selected one of the models to show the full cumulative feature removal plot for the glioma (Fig.~\ref{fig:acc_drop_fold1}) and knee (Fig.~\ref{fig:acc_drop_knee_model6}) tasks respectively.

We further tested whether the \textit{modality}-level performance (MI correlation) was correlated with \textit{feature}-level performance ($\Delta$AUPC): XAI method rankings based on the two metrics did not show a significant correlation on the glioma task, $\tau_b = -0.33, p=0.13$; they did show a moderate positive correlation that is statistically significant on the knee task, $\tau_b = 0.51, p=0.02$.

\begin{table*}[!h]

    \centering
    \resizebox{\textwidth}{!}{\begin{tabular}{m{0.2\linewidth} *{5}{>{\centering\arraybackslash}m{0.08\linewidth}}{>{\centering\arraybackslash}m{0.1\linewidth}}|
    *{5}{>{\centering\arraybackslash}m{0.08\linewidth}{>{\centering\arraybackslash}m{0.1\linewidth}}}
    }
    \toprule
     & \multicolumn{6}{c}{Glioma $\Delta$AUPC: replace with constant pixel} & \multicolumn{6}{c}{Glioma $\Delta$AUPC: replace with random unimportant pixel}\\

    \cline{2-13}
     & Model 1 & Model 2 & Model 3 & Model 4 & Model 5 & M $\pm$ SD & Model 1 & Model 2 & Model 3 & Model 4 & Model 5 & M $\pm$ SD\\
\hline
\hspace{0pt}Deconvolution &   0.22&   0.51&   \textbf{ 0.55 } &  0.31&   0.31&   0.38$\pm$0.14&   0.14&   \textbf{ 0.53 } &  0.18&   0.06&   0.28&   0.24$\pm$0.18  \\ \hline 

\hspace{0pt}DeepLift &   0.30&   0.22&   0.10&   0.12&   0.08&   0.16$\pm$0.10&   0.32&   0.24&   0.06&   0.12&   0.08&   0.16$\pm$0.11  \\ \hline 

\hspace{0pt}FeatureAblation &   0.24&   0.39&   0.27&   0.51&   0.29&   0.34$\pm$0.11&   0.28&   0.39&   0.17&   0.34&   0.29&   0.29$\pm$0.08  \\ \hline 

\hspace{0pt}FeaturePermutation &   -0.15&   0.00&   0.06&   -0.03&   -0.02&   -0.03$\pm$0.08&   -0.16&   -0.16&   -0.03&   0.03&   -0.02&   -0.07$\pm$0.09  \\ \hline 

\hspace{0pt}GradCAM &   -0.01&   0.25&   0.32&   0.40&   0.15&   0.22$\pm$0.16&   -0.01&   0.27&   0.22&   0.27&   0.17&   0.19$\pm$0.12  \\ \hline 

\hspace{0pt}Gradient &   0.12&   0.08&   0.09&   0.07&   0.08&   0.09$\pm$0.02&   0.15&   0.12&   0.00&   0.02&   0.10&   0.08$\pm$0.06  \\ \hline 

\hspace{0pt}GradientShap &   0.30&   0.31&   0.10&   0.12&   0.05&   0.18$\pm$0.12&   0.32&   0.31&   0.07&   0.11&   0.05&   0.17$\pm$0.13  \\ \hline 

\hspace{0pt}GuidedBackProp &   \textbf{ 0.52 } &  \textbf{ 0.58 } &  \textbf{ 0.58 } &  \textbf{ 0.58 } &  0.38&   \textbf{ 0.53$\pm$0.09 }&   \textbf{ 0.46 } &  \textbf{ 0.59 } &  \textbf{ 0.44 } &  0.24&   0.40&   0.43$\pm$0.13  \\ \hline 

\hspace{0pt}GuidedGradCAM &   \textbf{ 0.50 } &  \textbf{ 0.58 } &  \textbf{ 0.61 } &  \textbf{ 0.56 } &  0.39&   \textbf{ 0.53$\pm$0.09 }&   \textbf{ 0.44 } &  \textbf{ 0.58 } &  \textbf{ 0.49 } &  0.29&   0.42&   \textbf{ 0.44$\pm$0.10 }&  \\ \hline 

\hspace{0pt}InputXGradient &   0.33&   0.19&   0.10&   0.11&   0.07&   0.16$\pm$0.11&   0.35&   0.20&   0.06&   0.11&   0.07&   0.16$\pm$0.12  \\ \hline 

\hspace{0pt}IntegratedGradients &   0.31&   0.31&   0.10&   0.12&   0.07&   0.18$\pm$0.12&   0.33&   0.31&   0.07&   0.11&   0.07&   0.18$\pm$0.13  \\ \hline 

\hspace{0pt}KernelShap &   0.32&   0.45&   0.32&   0.28&   0.16&   0.31$\pm$0.10&   0.33&   0.30&   0.30&   0.16&   0.14&   0.24$\pm$0.09  \\ \hline 

\hspace{0pt}Lime &   0.38&   \textbf{ 0.58 } &  0.50&   \textbf{ 0.58 } &  \textbf{ 0.51 } &  \textbf{ 0.51$\pm$0.08 }&   0.37&   0.47&   0.31&   \textbf{ 0.38 } &  \textbf{ 0.43 } &  0.39$\pm$0.06  \\ \hline 

\hspace{0pt}Occlusion &   0.28&   0.30&   0.11&   0.16&   0.19&   0.21$\pm$0.08&   0.22&   0.27&   0.03&   0.02&   0.25&   0.16$\pm$0.12  \\ \hline 

\hspace{0pt}ShapleyValueSampling &   \textbf{ 0.41 } &  0.50&   0.46&   0.50&   \textbf{ 0.68 } &  0.51$\pm$0.10&   \textbf{ 0.39 } &  0.47&   0.43&   \textbf{ 0.42 } &  \textbf{ 0.69 } &  \textbf{ 0.48$\pm$0.12 }&  \\ \hline 

\hspace{0pt}SmoothGrad &   0.33&   0.50&   0.52&   0.53&   \textbf{ 0.52 } &  0.48$\pm$0.08&   0.33&   0.49&   \textbf{ 0.52 } &  \textbf{ 0.52 } &  \textbf{ 0.50 } &  \textbf{ 0.47$\pm$0.08 }&  \\ 

\bottomrule
    \end{tabular}}
    \caption{\textbf{Model-wise evaluation results on Guideline 3 Truthfulness - Cumulative feature removal experiment on the glioma task.} Results for two feature replacement approaches are reported: replacement with constant pixel is on the left half, and replacement with random unimportant pixel is on the right half. For each column, the top three XAI methods have their $\Delta$AUPC in bold. 
    }
    \label{tab:aupc_brain}
\end{table*}

\begin{table*}[!h]

    \centering
    \resizebox{\textwidth}{!}{\begin{tabular}{m{0.2\linewidth} *{5}{>{\centering\arraybackslash}m{0.08\linewidth}}{>{\centering\arraybackslash}m{0.1\linewidth}}|
    *{5}{>{\centering\arraybackslash}m{0.08\linewidth}{>{\centering\arraybackslash}m{0.1\linewidth}}}
    }
    \toprule
     & \multicolumn{6}{c}{Knee $\Delta$AUPC: replace with constant pixel} & \multicolumn{6}{c}{Knee $\Delta$AUPC: replace with random unimportant pixel}\\

    \cline{2-13}
     & Model 6 & Model 7 & Model 8 & Model 9 & Model 10 & M $\pm$ SD & Model 6 & Model 7 & Model 8 & Model 9 & Model 10 & M $\pm$ SD\\
\hline

\hspace{0pt}Deconvolution &   -0.05&   \textbf{ 0.03 } &  -0.05&   -0.06&   -0.07&   -0.04$\pm$0.04&   -0.09&   \textbf{ 0.01 } &  -0.12&   -0.09&   -0.12&   -0.08$\pm$0.06  \\ \hline 

\hspace{0pt}FeatureAblation &   0.03&   -0.04&   -0.07&   -0.04&   0.02&   -0.02$\pm$0.04&   -0.04&   -0.05&   -0.04&   -0.03&   -0.01&   -0.03$\pm$0.01  \\ \hline 

\hspace{0pt}Gradient &   -0.03&   -0.02&   -0.04&   -0.07&   -0.06&   -0.05$\pm$0.02&   -0.08&   -0.07&   -0.13&   -0.10&   -0.10&   -0.10$\pm$0.02  \\ \hline 

\hspace{0pt}GradientShap &   -0.02&   \textbf{ 0.00 } &  \textbf{ 0.02 } &  -0.03&   -0.07&   -0.02$\pm$0.03&   -0.11&   -0.04&   -0.09&   -0.09&   -0.04&   -0.07$\pm$0.03  \\ \hline 

\hspace{0pt}GuidedBackProp &   -0.05&   \textbf{ 0.02 } &  -0.06&   -0.05&   -0.07&   -0.04$\pm$0.03&   -0.09&   0.00&   -0.11&   -0.09&   -0.10&   -0.08$\pm$0.04  \\ \hline 

\hspace{0pt}InputXGradient &   -0.04&   -0.01&   -0.03&   -0.07&   -0.07&   -0.05$\pm$0.03&   -0.12&   -0.06&   -0.15&   -0.13&   -0.11&   -0.12$\pm$0.03  \\ \hline 

\hspace{0pt}IntegratedGradients &   -0.04&   -0.02&   \textbf{ -0.03 } &  -0.08&   -0.06&   -0.04$\pm$0.02&   -0.15&   -0.08&   -0.14&   -0.14&   -0.11&   -0.12$\pm$0.03  \\ \hline 

\hspace{0pt}KernelShap &   \textbf{ 0.03 } &  -0.01&   -0.04&   \textbf{ -0.01 } &  \textbf{ 0.03 } &  \textbf{ 0.00$\pm$0.03 }&   \textbf{ 0.01 } &  \textbf{ 0.02 } &  \textbf{ 0.02 } &  \textbf{ 0.01 } &  \textbf{ 0.02 } &  \textbf{ 0.02$\pm$0.01 }&  \\ \hline 

\hspace{0pt}Lime &   \textbf{ 0.04 } &  -0.03&   -0.04&   -0.02&   \textbf{ 0.05 } &  \textbf{ 0.00$\pm$0.04 }&   \textbf{ 0.05 } &  \textbf{ 0.03 } &  \textbf{ 0.05 } &  \textbf{ 0.01 } &  \textbf{ 0.05 } &  \textbf{ 0.04$\pm$0.02 }&  \\ \hline 

\hspace{0pt}Occlusion &   0.01&   -0.02&   \textbf{ -0.03 } &  \textbf{ -0.01 } &  0.00&   -0.01$\pm$0.02&   -0.03&   -0.05&   -0.06&   -0.07&   -0.07&   -0.06$\pm$0.02  \\ \hline 

\hspace{0pt}ShapleyValueSampling &   \textbf{ 0.03 } &  -0.01&   -0.05&   \textbf{ -0.02 } &  \textbf{ 0.03 } &  \textbf{ 0.00$\pm$0.04 }&   \textbf{ 0.00 } &  0.01&   \textbf{ 0.00 } &  \textbf{ -0.01 } &  \textbf{ 0.07 } &  \textbf{ 0.01$\pm$0.03 }&  \\ \hline 

\hspace{0pt}SmoothGrad &   0.00&   -0.09&   -0.04&   -0.07&   -0.04&   -0.05$\pm$0.03&   -0.07&   -0.14&   -0.07&   -0.10&   -0.14&   -0.10$\pm$0.03  \\

\bottomrule
    \end{tabular}}
    \caption{\textbf{Model-wise evaluation results on Guideline 3 Truthfulness - Cumulative feature removal experiment on the \textbf{knee} task.} Results for two feature replacement approaches are reported: replacement with constant pixel is on the left half, and replacement with random unimportant pixel is on the right half. For each column, the top three XAI methods have their $\Delta$AUPC in bold.  
    }
    \label{tab:aupc_knee}
\end{table*}

\begin{figure*}[!ht]
    \centering
    \includegraphics[width=1\linewidth]{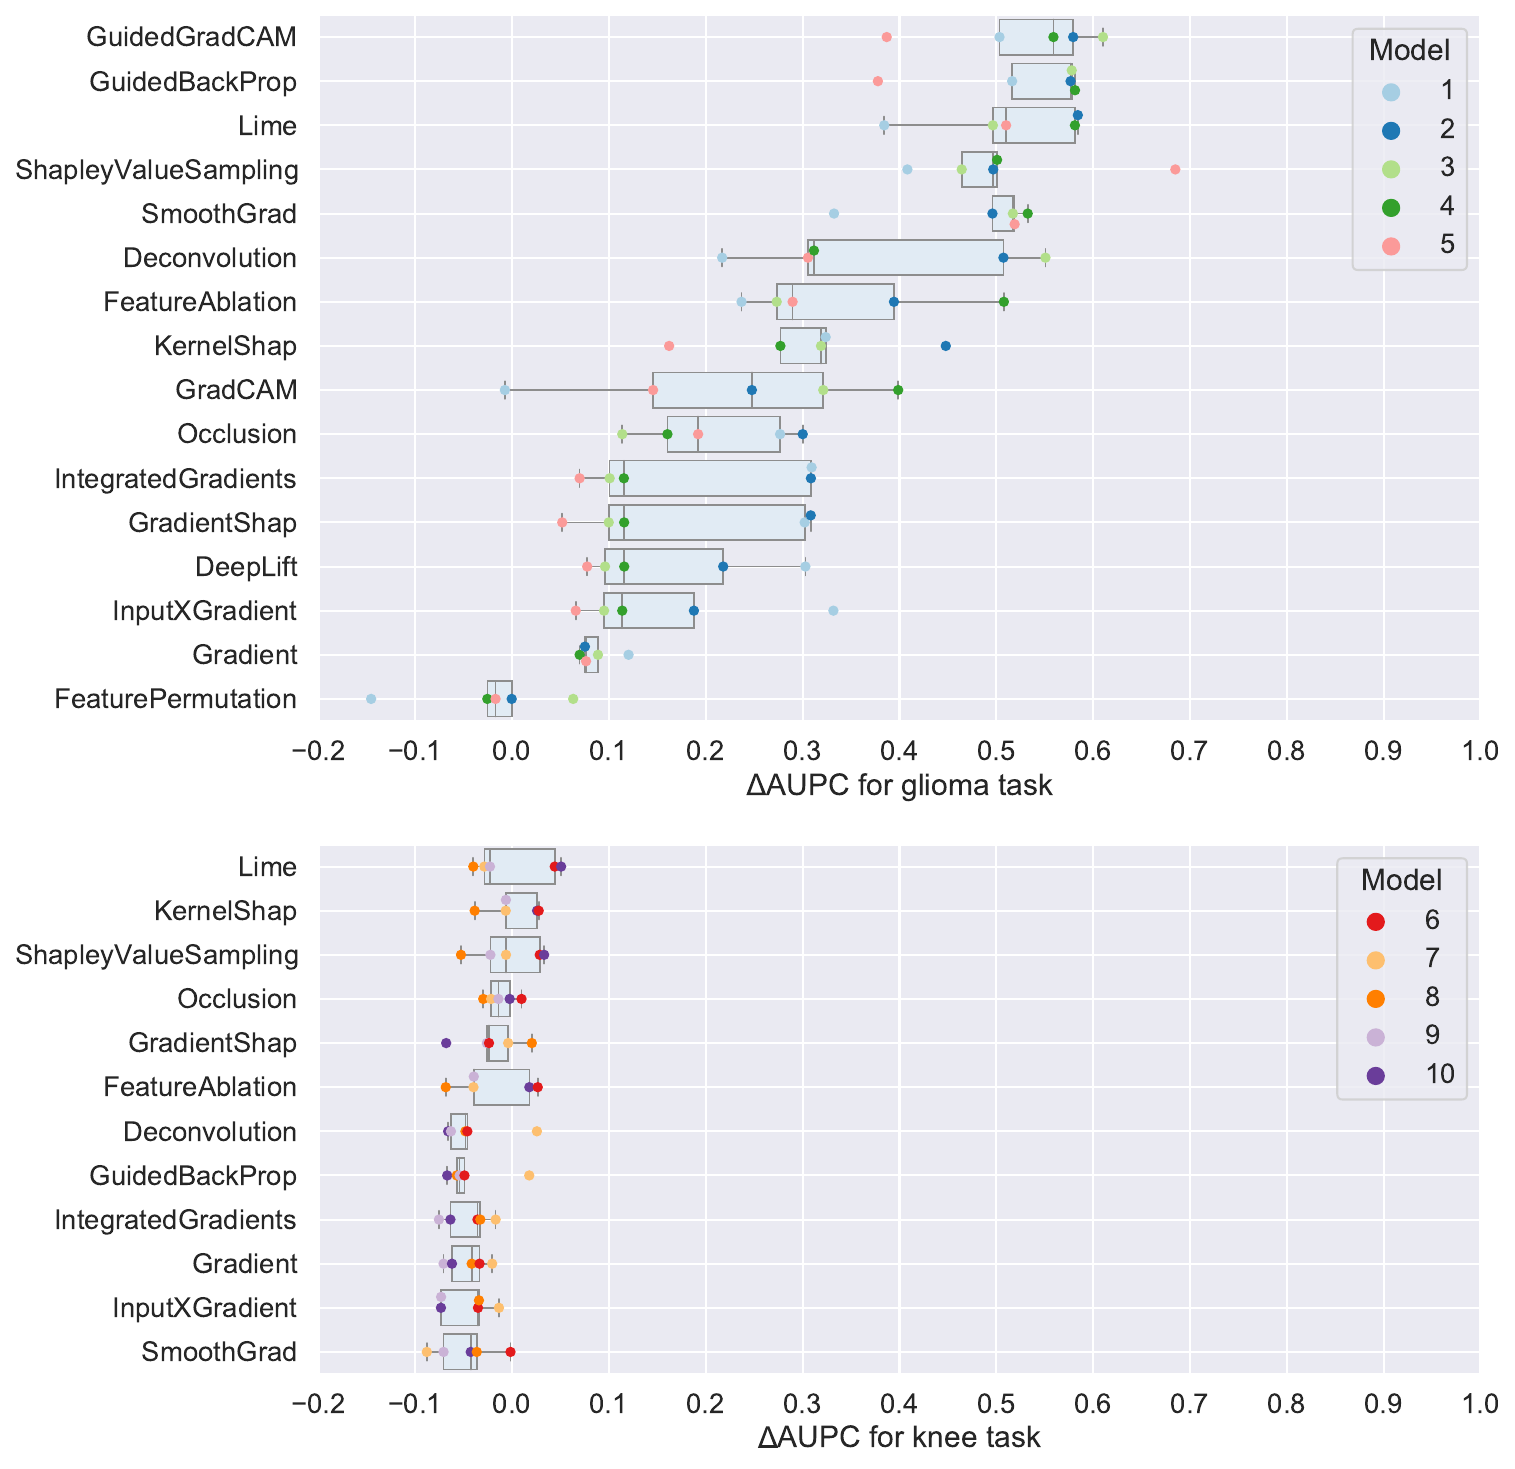}
    \caption{\textbf{Evaluation results on G3 Truthfulness - Cumulative feature removal.} Each dot is the $\Delta$AUPC value of an XAI method on a model, and the box plots show the range. We report $\Delta$AUPC using the feature replacement approach of constant pixel. The top and bottom plot shows the glioma (Model 1-5) and knee (Model 6-10) tasks, respectively.
XAI methods are ranked according to their mean $\Delta$AUPC value.} 
    \label{fig:acc_drop_perf}
\end{figure*}
\FloatBarrier

\begin{figure*}[h]
    \centering
    \includegraphics[width=1\linewidth]{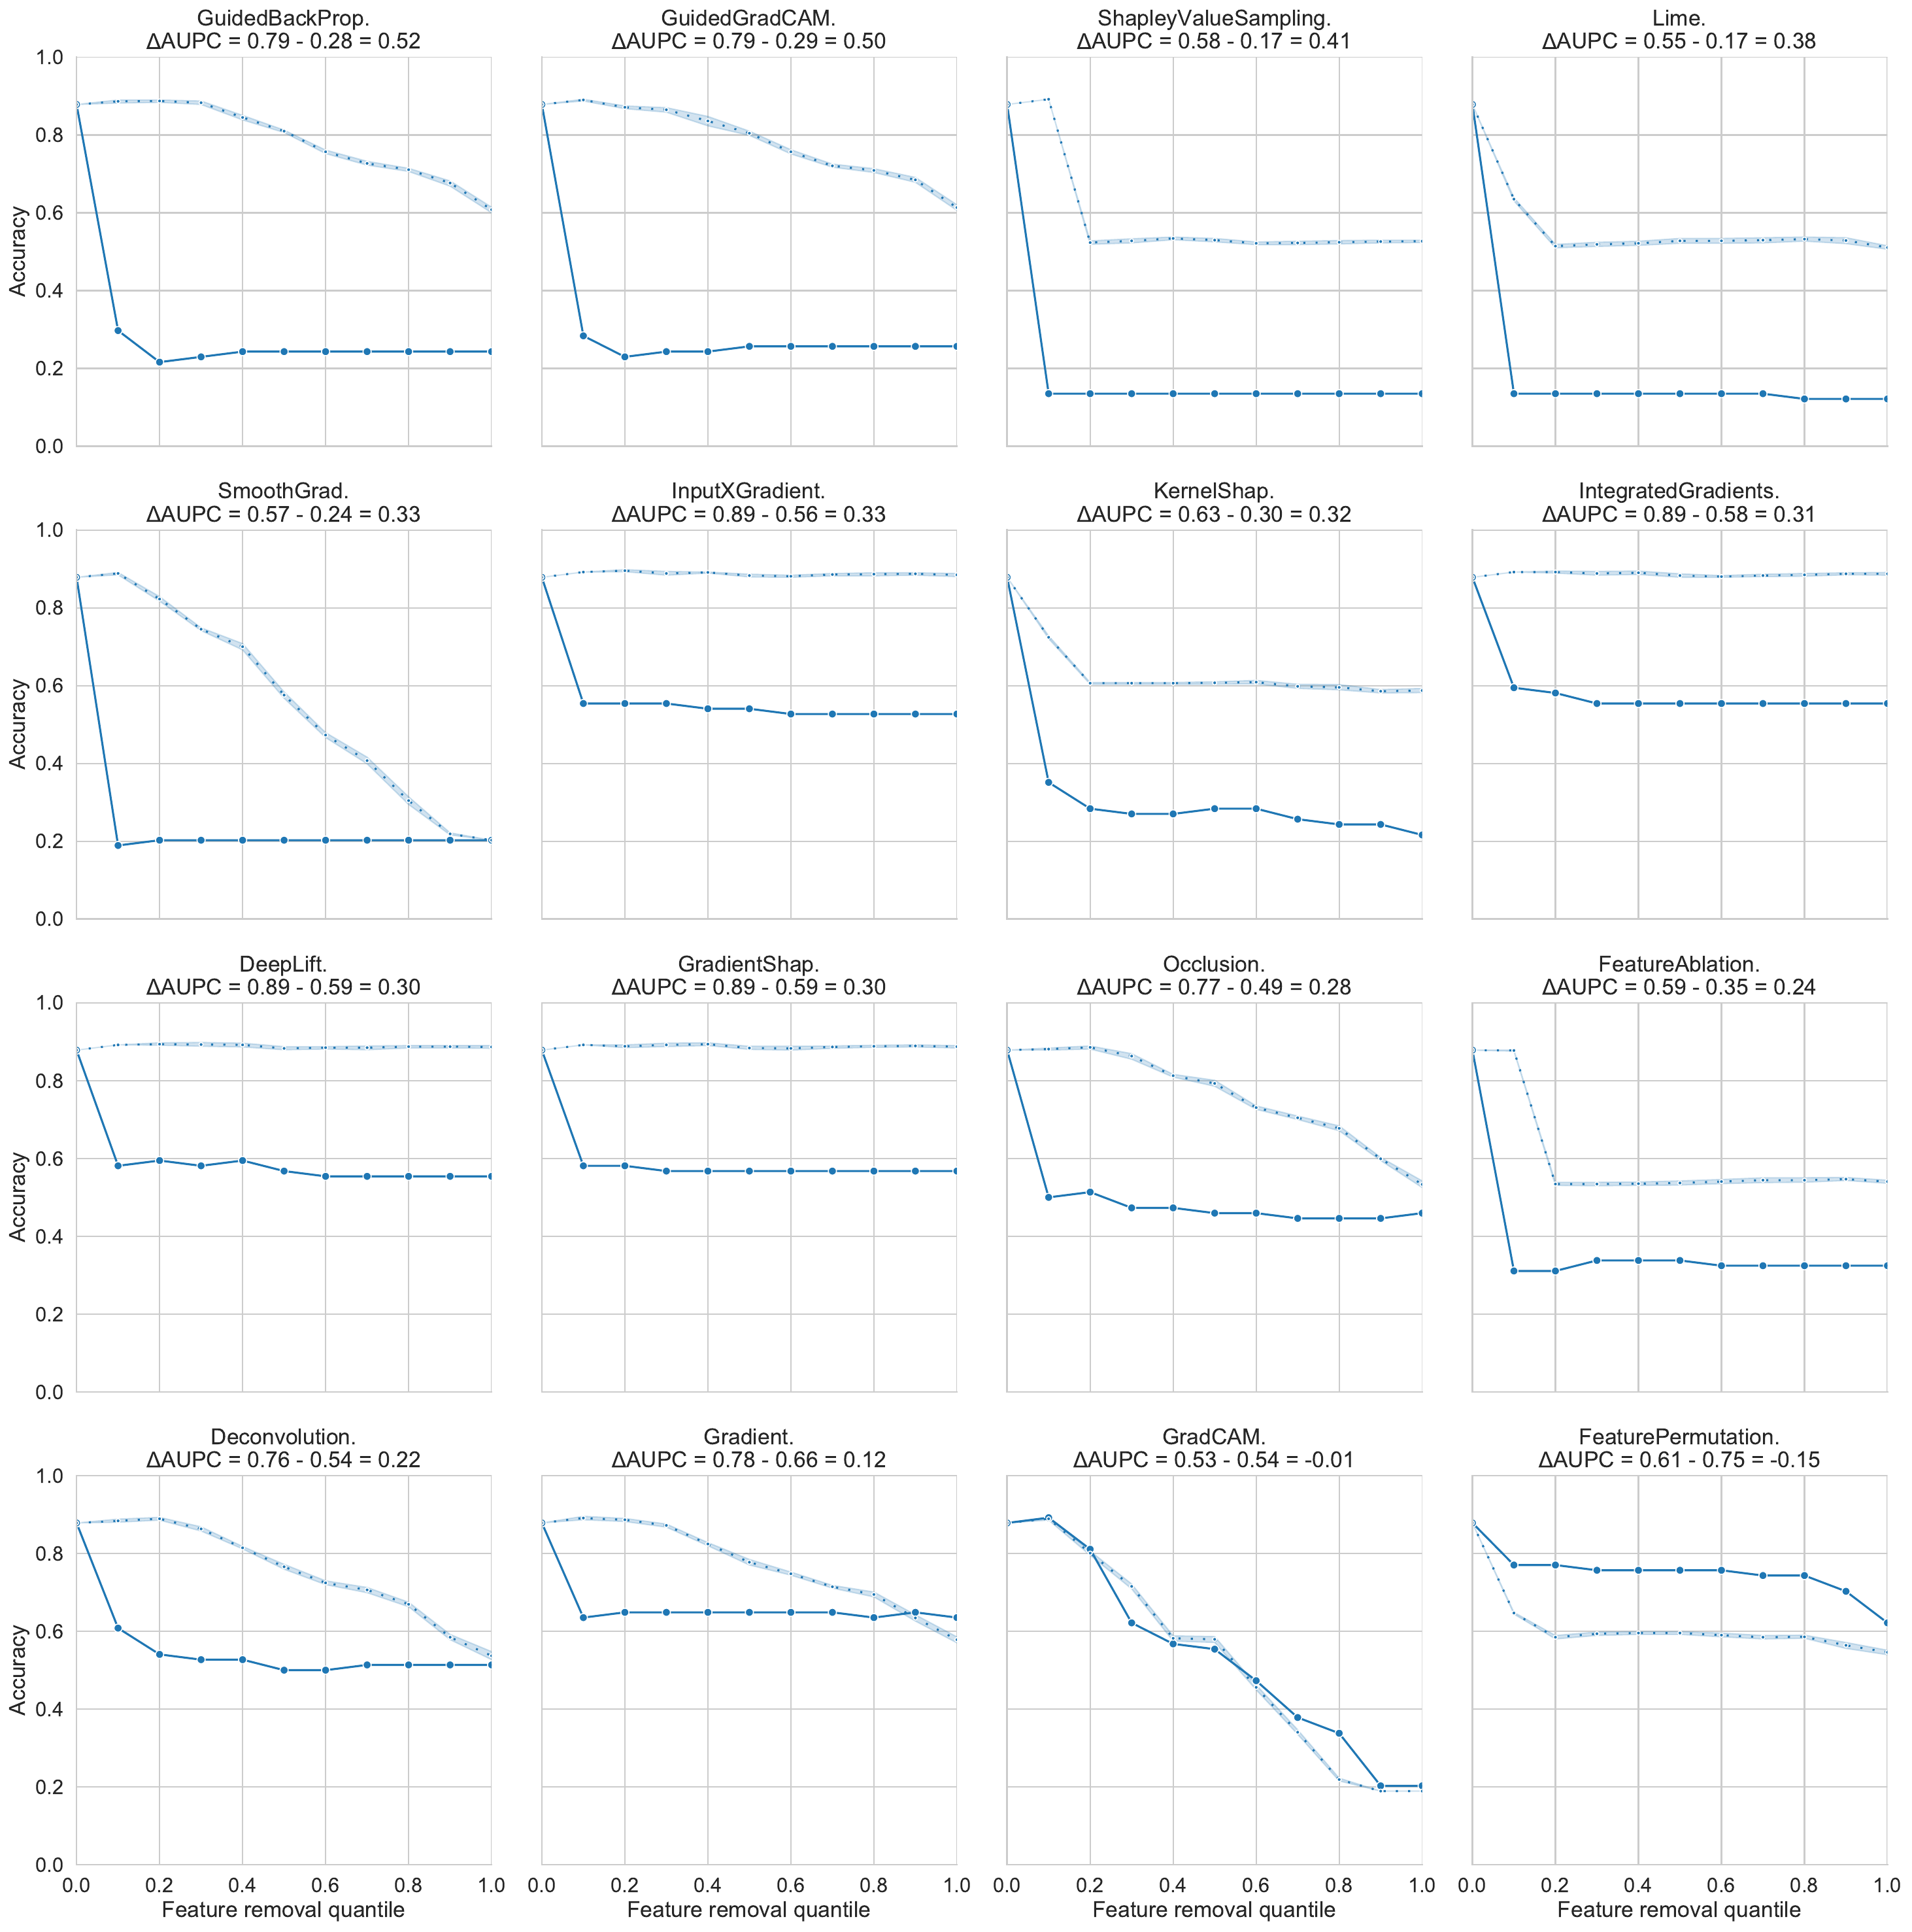}
    \caption{\textbf{Feature perturbation curve of cumulative feature removal experiment on the glioma task.} Each plot shows the feature perturbation curve of an XAI method ($\mathcal{H}$, solid line) and its random baseline ($\mathcal{H}_b$, dashed line). A bigger gap between the two curves indicates a higher $\Delta$AUPC, thus a better performance. 
     Plots were arranged 
    according to their $\Delta$AUPC value ($\Delta\text{AUPC}(\mathcal{H}) = \text{AUPC}(\mathcal{H}_b) -
\text{AUPC}(\mathcal{H})$, with numbers rounded to two decimal places) as indicated in the plot subtitle. We report $\Delta$AUPC from model 1 using the feature replacement approach of constant pixel.
    }
    \label{fig:acc_drop_fold1}
\end{figure*}
\FloatBarrier

\begin{figure*}[h]
    \centering
    \includegraphics[width=1\linewidth]{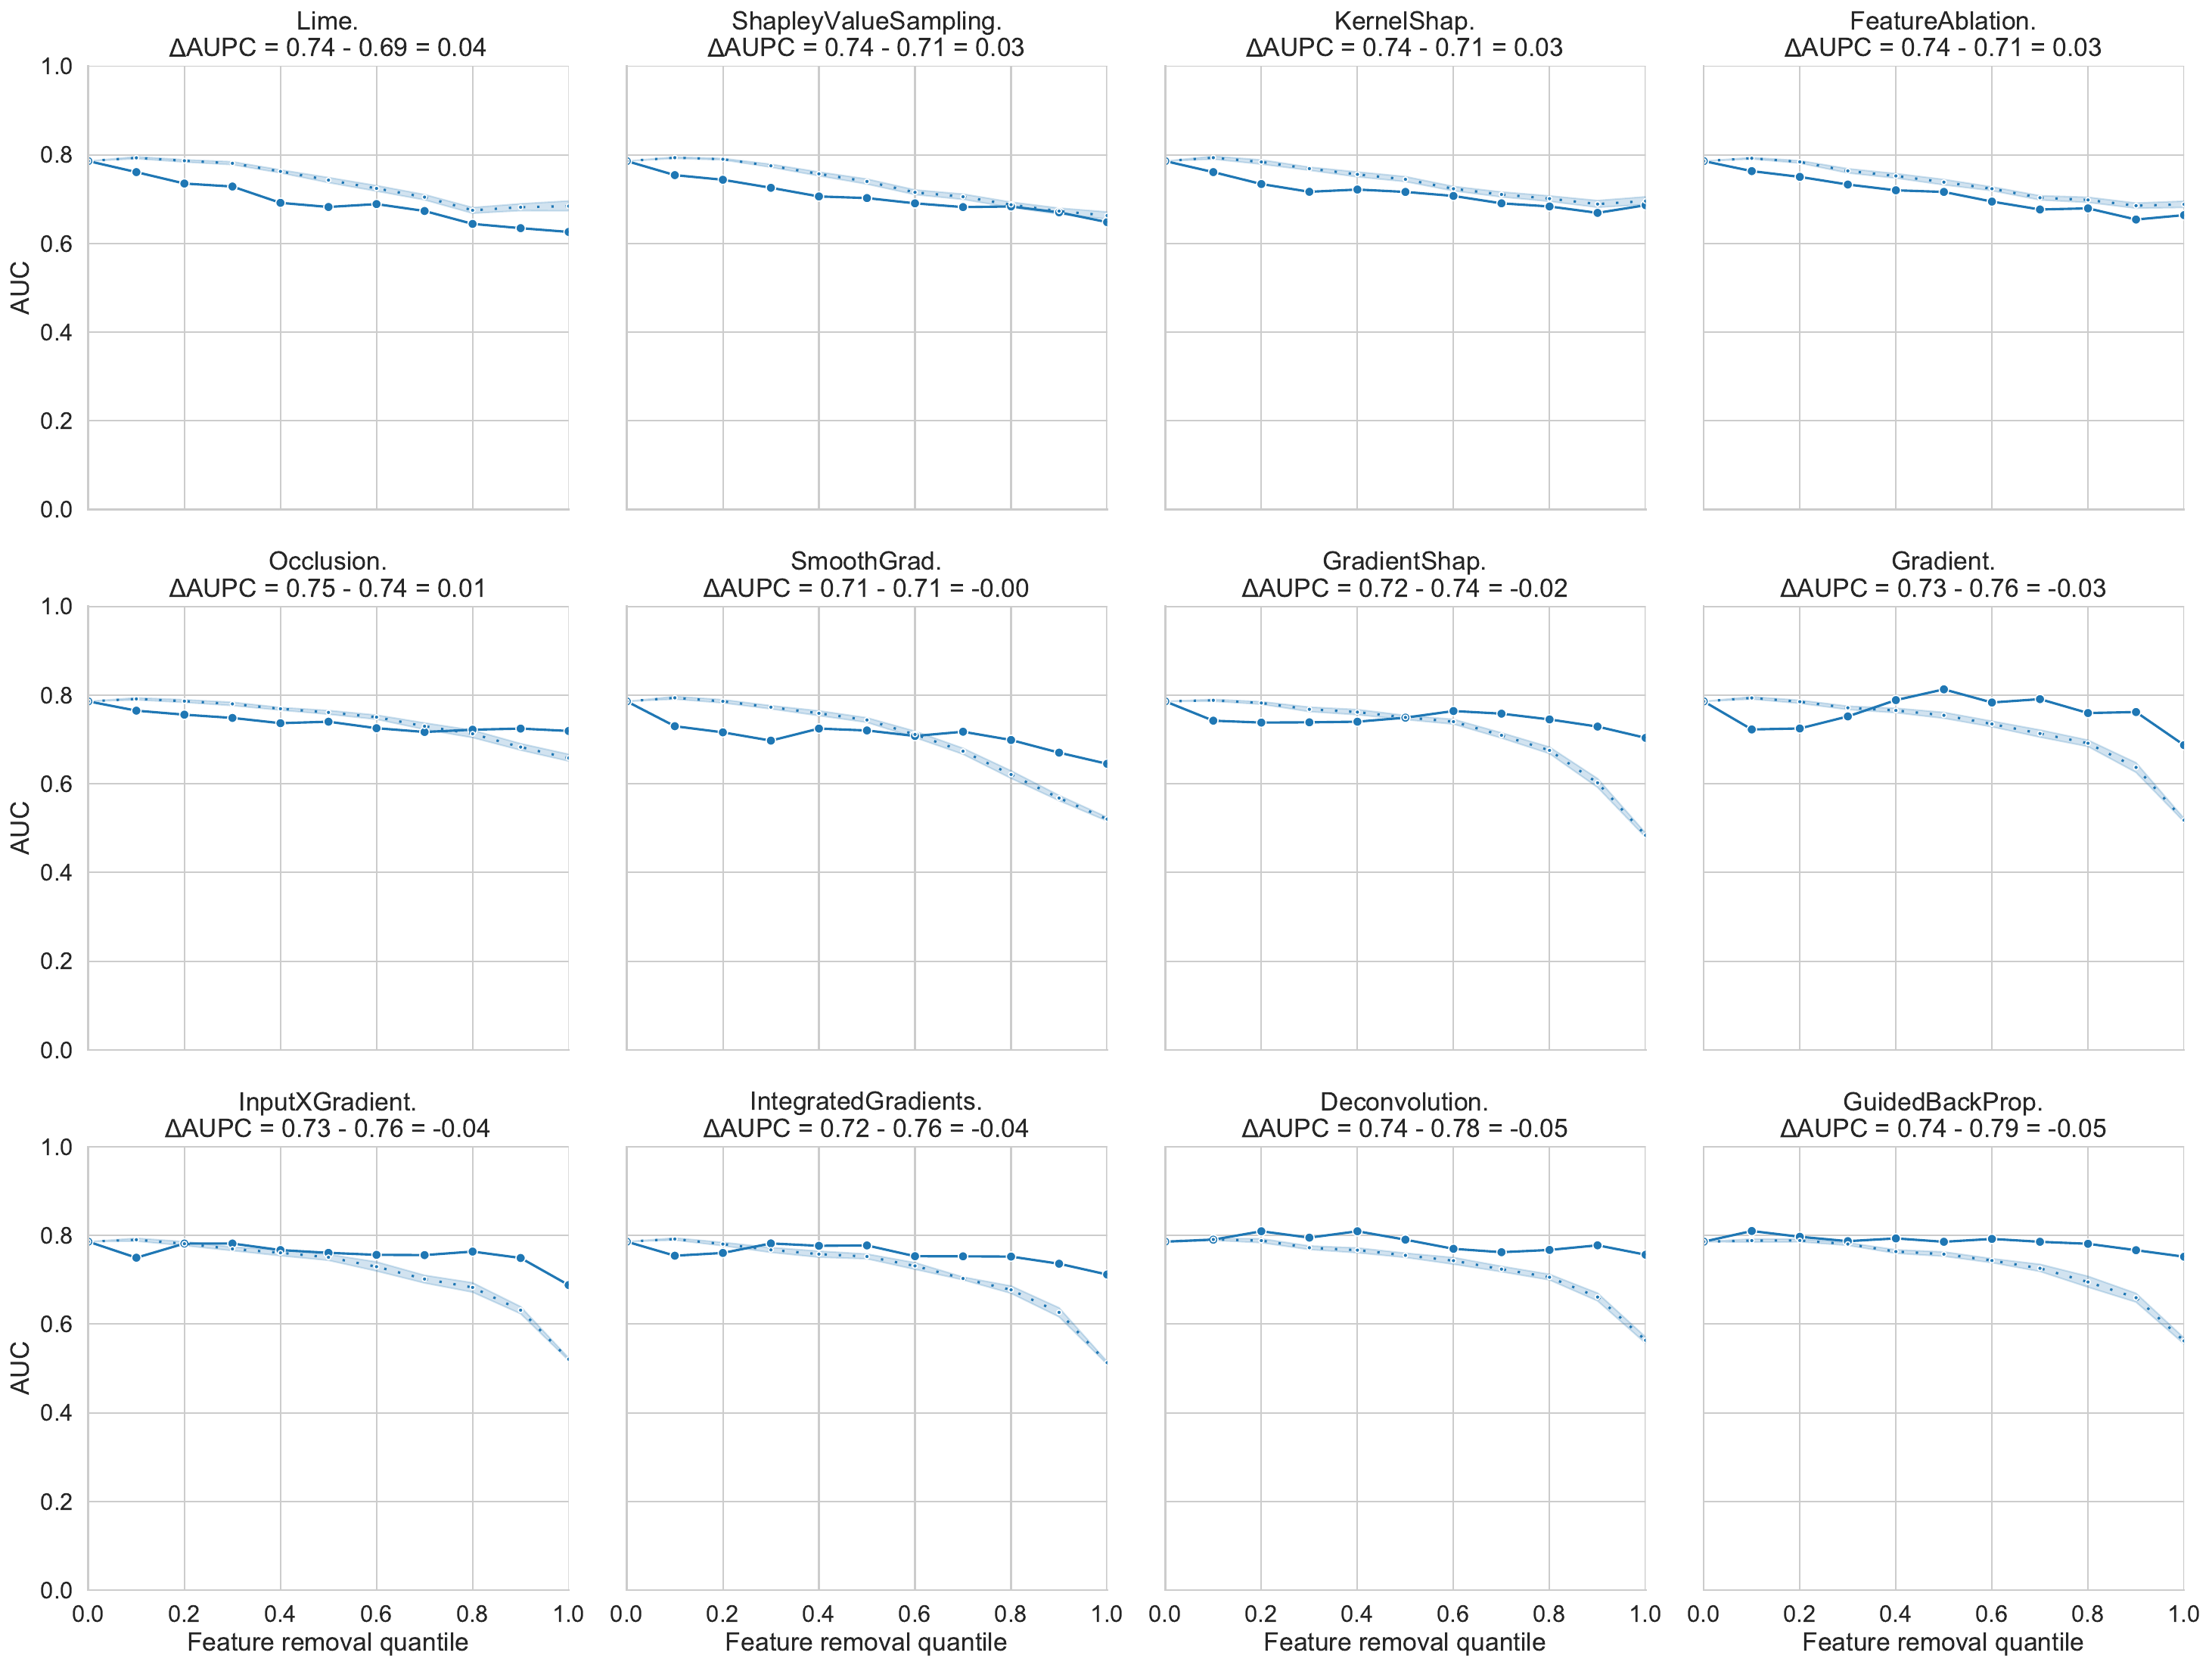}
    \caption{\textbf{Feature perturbation curve of cumulative feature removal experiment on the knee task.} Each plot shows the feature perturbation curve of an XAI method ($\mathcal{H}$, solid line) and its random baseline ($\mathcal{H}_b$, dashed line). A bigger gap between the two curves indicates a higher $\Delta$AUPC, thus a better performance. 
     Plots were arranged 
    according to their $\Delta$AUPC value ($\Delta\text{AUPC}(\mathcal{H}) = \text{AUPC}(\mathcal{H}_b) -
\text{AUPC}(\mathcal{H})$, with numbers rounded to two decimal places) as indicated in the plot subtitle. We report $\Delta$AUPC from model 6 using the feature replacement approach of constant pixel.
    }
    \label{fig:acc_drop_knee_model6}
\end{figure*}
\FloatBarrier

\subsection{G4 Informative Plausibility}

\subsubsection{Correlation between Plausibility Measures and Model Output Probability}

We describe our pre-processing method to convert model output probability to probability for the target label, in order to calculate the correlation between it and the plausibility measure. Both clinical tasks are binary classifications.
For the glioma task, we directly used the softmax output for the target class; for the knee task, since the output probability used the sigmoid function with $>0.5$ indicating positive class and $\leq0.5$ for negative one, the model probability for the target (ground-truth or prediction) label $T$ is converted from the sigmoid output probability $p$ as follows:
\begin{align}\label{eq:prob_conf}
    T = 
\begin{cases}
  p & \text{if target class = 1} \\
  1-p & \text{otherwise}
\end{cases}
\end{align}

For the correlation between model output probability and plausibility measure, we report model-wise performance in Table~\ref{tab:spearman_brain}, \ref{tab:spearman_brain_gt}, \ref{tab:spearman_knee}, \ref{tab:spearman_knee_gt} with plausibility measure using MSFI or FP, and the target being prediction or ground-truth label.
From the results, we observed that the plausibility measure (using MSFI or FP) has a higher correlation with \textit{prediction} probability, than the correlation with \textit{ground-truth} probability on both tasks using either MSFI or FP. 
This may be due to the fact that estimating the ground-truth probability requires additional information on the ground truth, which is unknown to the model. It indicates that explanation is better at explaining the known information from the model (i.e.  prediction label probability), rather than the unknown (i.e. ground truth label probability).

\begin{table*}[!h]

    \centering
    \resizebox{\textwidth}{!}{\begin{tabular}{m{0.2\linewidth} *{5}{>{\centering\arraybackslash}m{0.08\linewidth}}{>{\centering\arraybackslash}m{0.1\linewidth}}|
    *{5}{>{\centering\arraybackslash}m{0.08\linewidth}{>{\centering\arraybackslash}m{0.1\linewidth}}}
    }
    \toprule
     & \multicolumn{6}{c}{\textbf{Glioma}: \textbf{MSFI} correlation with \textbf{prediction} probability} & \multicolumn{6}{c}{\textbf{Glioma}: \textbf{FP} correlation with \textbf{prediction} probability}\\

    \cline{2-13}
     & Model 1 & Model 2 & Model 3 & Model 4 & Model 5 & All & Model 1 & Model 2 & Model 3 & Model 4 & Model 5 & All \\
\hline

\hspace{0pt}Deconvolution &  0.46 & \underline{ 0.20 }  & 0.50 & 0.37 & \textbf{ 0.72 }  & 0.41 & 0.40 & 0.41 & 0.51 & 0.33 & \textbf{ 0.72 }  & 0.44 & \\ \hline 

\hspace{0pt}DeepLift &  0.59 & 0.51 & \textbf{ 0.69 }  & 0.49 & \textbf{ 0.65 }  & 0.49 & \textbf{ 0.62 }  & 0.45 & \textbf{ 0.71 }  & 0.48 & \textbf{ 0.62 }  & 0.46 & \\ \hline 

\hspace{0pt}FeatureAblation &  0.55 & 0.58 & \textbf{ 0.75 }  & 0.59 & \textbf{ 0.75 }  & 0.59 & 0.54 & 0.52 & \textbf{ 0.65 }  & 0.55 & \textbf{ 0.74 }  & 0.58 & \\ \hline 

\hspace{0pt}FeaturePermutation &  \underline{ -0.07 }  & 0.26 & \underline{ 0.20 }  & 0.46 & \underline{ 0.10 }  & 0.19 & \underline{ -0.07 }  & \underline{ -0.03 }  & 0.26 & 0.44 & \underline{ 0.14 }  & 0.16 & \\ \hline 

\hspace{0pt}GradCAM &  \underline{ 0.04 }  & \underline{ 0.12 }  & 0.46 & \underline{ 0.21 }  & \underline{ 0.15 }  & 0.18 & \underline{ 0.04 }  & \underline{ 0.08 }  & 0.45 & \underline{ 0.22 }  & \underline{ 0.19 }  & 0.18 & \\ \hline 

\hspace{0pt}Gradient &  0.50 & 0.24 & 0.55 & 0.40 & \textbf{ 0.63 }  & 0.41 & 0.48 & 0.32 & 0.48 & 0.34 & 0.58 & 0.40 & \\ \hline 

\hspace{0pt}GradientShap &  0.59 & 0.52 & \textbf{ 0.63 }  & 0.50 & \textbf{ 0.64 }  & 0.49 & 0.59 & 0.39 & \textbf{ 0.65 }  & 0.49 & \textbf{ 0.65 }  & 0.47 & \\ \hline 

\hspace{0pt}GuidedBackProp &  0.47 & 0.26 & 0.58 & 0.34 & \textbf{ 0.65 }  & 0.41 & 0.43 & 0.42 & 0.57 & 0.28 & 0.58 & 0.39 & \\ \hline 

\hspace{0pt}GuidedGradCAM &  0.29 & 0.24 & \textbf{ 0.63 }  & 0.38 & 0.45 & 0.37 & 0.32 & 0.44 & \textbf{ 0.65 }  & 0.36 & 0.46 & 0.37 & \\ \hline 

\hspace{0pt}InputXGradient &  \textbf{ 0.63 }  & 0.55 & 0.60 & 0.54 & \textbf{ 0.77 }  & 0.57 & \textbf{ 0.64 }  & 0.48 & \textbf{ 0.63 }  & 0.53 & \textbf{ 0.73 }  & 0.53 & \\ \hline 

\hspace{0pt}IntegratedGradients &  \textbf{ 0.62 }  & 0.52 & \textbf{ 0.64 }  & 0.51 & \textbf{ 0.67 }  & 0.50 & \textbf{ 0.61 }  & 0.44 & \textbf{ 0.67 }  & 0.50 & \textbf{ 0.64 }  & 0.49 & \\ \hline 

\hspace{0pt}KernelShap &  \underline{ 0.22 }  & 0.46 & 0.59 & 0.38 & 0.34 & 0.36 & 0.26 & 0.38 & \textbf{ 0.63 }  & 0.39 & 0.39 & 0.36 & \\ \hline 

\hspace{0pt}Lime &  0.33 & 0.39 & 0.51 & \underline{ 0.19 }  & 0.39 & 0.36 & 0.35 & 0.38 & 0.48 & \underline{ 0.15 }  & 0.37 & 0.33 & \\ \hline 

\hspace{0pt}Occlusion &  \textbf{ 0.75 }  & \textbf{ 0.61 }  & \textbf{ 0.67 }  & \textbf{ 0.62 }  & \textbf{ 0.78 }  & 0.60 & \textbf{ 0.60 }  & 0.54 & \textbf{ 0.68 }  & 0.56 & \textbf{ 0.76 }  & 0.52 & \\ \hline 

\hspace{0pt}ShapleyValueSampling &  0.59 & 0.58 & \textbf{ 0.62 }  & 0.50 & \textbf{ 0.70 }  & 0.53 & 0.55 & 0.52 & 0.56 & 0.40 & \textbf{ 0.67 }  & 0.50 & \\ \hline 

\hspace{0pt}SmoothGrad &  \textbf{ 0.67 }  & 0.27 & 0.54 & 0.40 & \textbf{ 0.64 }  & 0.36 & 0.55 & \underline{ 0.20 }  & 0.46 & 0.34 & \textbf{ 0.63 }  & 0.28 & \\

\bottomrule
    \end{tabular}}
    \caption{
    Model-wise Spearman's correlation coefficient $r$ between prediction probability and heatmap plausibility measures of MSFI (left half) and FP (right half) on the glioma task. We indicate the strongly positive correlated ones ($\geq 0.6$) in bold. Except for the correlation coefficients that are underlined, the remaining correlations are statistically significant.
    }
    \label{tab:spearman_brain}
\end{table*}
\FloatBarrier

\begin{table*}[!h]

    \centering
    \resizebox{\textwidth}{!}{\begin{tabular}{m{0.2\linewidth} *{5}{>{\centering\arraybackslash}m{0.08\linewidth}}{>{\centering\arraybackslash}m{0.1\linewidth}}|
    *{5}{>{\centering\arraybackslash}m{0.08\linewidth}{>{\centering\arraybackslash}m{0.1\linewidth}}}
    }
    \toprule
     & \multicolumn{6}{c}{\textbf{Glioma}: \textbf{MSFI} correlation with \textbf{ground-truth} probability} & \multicolumn{6}{c}{\textbf{Glioma}: \textbf{FP} correlation with \textbf{ground-truth} probability}\\

    \cline{2-13}
     & Model 1 & Model 2 & Model 3 & Model 4 & Model 5 & All & Model 1 & Model 2 & Model 3 & Model 4 & Model 5 & All \\
\hline

\hspace{0pt}Deconvolution &  0.36 & \underline{ 0.07 }  & 0.35 & 0.24 & 0.53 & 0.30 & 0.28 & 0.34 & 0.35 & \underline{ 0.19 }  & 0.52 & 0.32 & \\ \hline 

\hspace{0pt}DeepLift &  0.57 & 0.44 & 0.57 & 0.40 & 0.53 & 0.41 & 0.57 & 0.39 & 0.59 & 0.37 & 0.48 & 0.38 & \\ \hline 

\hspace{0pt}FeatureAblation &  0.47 & 0.51 & \textbf{ 0.64 }  & 0.54 & \textbf{ 0.65 }  & 0.52 & 0.50 & 0.47 & 0.53 & 0.48 & \textbf{ 0.61 }  & 0.50 & \\ \hline 

\hspace{0pt}FeaturePermutation &  \underline{ -0.08 }  & \underline{ 0.22 }  & \underline{ 0.19 }  & 0.42 & \underline{ 0.10 }  & 0.17 & \underline{ -0.07 }  & \underline{ 0.02 }  & 0.23 & 0.40 & \underline{ 0.15 }  & 0.16 & \\ \hline 

\hspace{0pt}GradCAM &  \underline{ -0.02 }  & \underline{ 0.07 }  & 0.37 & \underline{ 0.12 }  & \underline{ 0.14 }  & 0.12 & \underline{ -0.03 }  & \underline{ 0.06 }  & 0.36 & \underline{ 0.13 }  & \underline{ 0.15 }  & 0.12 & \\ \hline 

\hspace{0pt}Gradient &  0.46 & \underline{ 0.15 }  & 0.41 & 0.30 & 0.48 & 0.32 & 0.42 & 0.23 & 0.33 & 0.24 & 0.43 & 0.30 & \\ \hline 

\hspace{0pt}GradientShap &  0.53 & 0.46 & 0.51 & 0.41 & 0.52 & 0.41 & 0.50 & 0.32 & 0.53 & 0.40 & 0.51 & 0.38 & \\ \hline 

\hspace{0pt}GuidedBackProp &  0.47 & \underline{ 0.15 }  & 0.47 & 0.26 & 0.49 & 0.32 & 0.36 & 0.33 & 0.43 & \underline{ 0.19 }  & 0.41 & 0.30 & \\ \hline 

\hspace{0pt}GuidedGradCAM &  0.30 & \underline{ 0.11 }  & 0.52 & 0.28 & 0.36 & 0.28 & \underline{ 0.22 }  & 0.35 & 0.52 & 0.25 & 0.33 & 0.28 & \\ \hline 

\hspace{0pt}InputXGradient &  0.59 & 0.48 & 0.47 & 0.44 & \textbf{ 0.63 }  & 0.47 & 0.59 & 0.42 & 0.50 & 0.44 & 0.58 & 0.44 & \\ \hline 

\hspace{0pt}IntegratedGradients &  0.56 & 0.45 & 0.52 & 0.42 & 0.54 & 0.42 & 0.54 & 0.37 & 0.53 & 0.41 & 0.49 & 0.39 & \\ \hline 

\hspace{0pt}KernelShap &  \underline{ 0.15 }  & 0.45 & 0.51 & 0.31 & \underline{ 0.18 }  & 0.28 & \underline{ 0.17 }  & 0.28 & 0.55 & 0.31 & \underline{ 0.21 }  & 0.26 & \\ \hline 

\hspace{0pt}Lime &  0.30 & 0.38 & 0.46 & \underline{ 0.18 }  & 0.28 & 0.31 & 0.31 & 0.27 & 0.43 & \underline{ 0.13 }  & 0.26 & 0.27 & \\ \hline 

\hspace{0pt}Occlusion &  \textbf{ 0.61 }  & 0.53 & \textbf{ 0.62 }  & 0.53 & \textbf{ 0.67 }  & 0.52 & 0.45 & 0.47 & 0.57 & 0.47 & \textbf{ 0.63 }  & 0.42 & \\ \hline 

\hspace{0pt}ShapleyValueSampling &  0.52 & 0.50 & 0.49 & 0.39 & 0.53 & 0.43 & 0.48 & 0.46 & 0.44 & 0.30 & 0.49 & 0.40 & \\ \hline 

\hspace{0pt}SmoothGrad &  0.58 & \underline{ 0.18 }  & 0.39 & 0.30 & 0.47 & 0.27 & 0.43 & \underline{ 0.15 }  & 0.31 & 0.25 & 0.45 & 0.21 & \\ 

\bottomrule
    \end{tabular}}
    \caption{
    Model-wise Spearman's correlation coefficient $r$ between model ground-truth probability and heatmap plausibility measures of MSFI (left half) and FP (right half) on the glioma task. We indicate the strongly positive correlated ones ($\geq 0.6$) in bold. Except for the correlation coefficients that are underlined, the remaining correlations are statistically significant.
    }
    \label{tab:spearman_brain_gt}
\end{table*}
\FloatBarrier

\begin{table*}[!h]

    \centering
    \resizebox{\textwidth}{!}{\begin{tabular}{m{0.2\linewidth} *{5}{>{\centering\arraybackslash}m{0.08\linewidth}}{>{\centering\arraybackslash}m{0.1\linewidth}}|
    *{5}{>{\centering\arraybackslash}m{0.08\linewidth}{>{\centering\arraybackslash}m{0.1\linewidth}}}
    }
    \toprule
     & \multicolumn{6}{c}{\textbf{Knee}: \textbf{MSFI} correlation with \textbf{prediction} probability} & \multicolumn{6}{c}{\textbf{Knee}: \textbf{FP} correlation with \textbf{prediction} probability}\\

    \cline{2-13}
     & Model 6 & Model 7 & Model 8 & Model 9 & Model 10 & All & Model 6 & Model 7 & Model 8 & Model 9 & Model 10 & All \\
\hline

\hspace{0pt}Deconvolution &  \underline{ -0.08 }  & \underline{ -0.15 }  & \underline{ -0.05 }  & \underline{ -0.01 }  & \underline{ -0.14 }  & -0.08 & \underline{ -0.09 }  & \underline{ -0.11 }  & \underline{ -0.03 }  & \underline{ -0.06 }  & \underline{ -0.13 }  & \underline{ -0.08 }  & \\ \hline 

\hspace{0pt}FeatureAblation &  -0.26 & -0.20 & \underline{ -0.15 }  & \underline{ -0.14 }  & \underline{ -0.09 }  & -0.16 & -0.26 & \underline{ -0.12 }  & \underline{ -0.11 }  & \underline{ -0.15 }  & \underline{ -0.07 }  & -0.14 & \\ \hline 

\hspace{0pt}Gradient &  \underline{ -0.09 }  & \underline{ -0.13 }  & \underline{ 0.00 }  & \underline{ -0.05 }  & \underline{ -0.12 }  & -0.08 & \underline{ -0.09 }  & \underline{ -0.07 }  & \underline{ 0.03 }  & \underline{ -0.09 }  & \underline{ -0.12 }  & \underline{ -0.08 }  & \\ \hline 

\hspace{0pt}GradientShap &  \underline{ -0.11 }  & -0.19 & \underline{ -0.01 }  & \underline{ -0.01 }  & \underline{ -0.10 }  & -0.09 & \underline{ -0.11 }  & \underline{ -0.14 }  & \underline{ -0.02 }  & \underline{ -0.05 }  & \underline{ -0.08 }  & -0.09 & \\ \hline 

\hspace{0pt}GuidedBackProp &  \underline{ -0.08 }  & \underline{ -0.14 }  & \underline{ -0.03 }  & \underline{ 0.00 }  & \underline{ -0.10 }  & \underline{ -0.07 }  & \underline{ -0.08 }  & \underline{ -0.10 }  & \underline{ -0.02 }  & \underline{ -0.05 }  & \underline{ -0.10 }  & \underline{ -0.07 }  & \\ \hline 

\hspace{0pt}InputXGradient &  \underline{ -0.12 }  & \underline{ -0.13 }  & \underline{ -0.02 }  & \underline{ 0.00 }  & \underline{ -0.13 }  & -0.08 & \underline{ -0.13 }  & \underline{ -0.08 }  & \underline{ -0.01 }  & \underline{ -0.04 }  & \underline{ -0.11 }  & -0.08 & \\ \hline 

\hspace{0pt}IntegratedGradients &  \underline{ -0.09 }  & \underline{ -0.16 }  & \underline{ -0.12 }  & \underline{ 0.03 }  & \underline{ -0.04 }  & \underline{ -0.08 }  & \underline{ -0.09 }  & \underline{ -0.14 }  & \underline{ -0.12 }  & \underline{ 0.01 }  & \underline{ -0.03 }  & \underline{ -0.08 }  & \\ \hline 

\hspace{0pt}KernelShap &  -0.20 & \underline{ -0.15 }  & \underline{ -0.09 }  & \underline{ -0.14 }  & \underline{ -0.10 }  & -0.13 & -0.25 & -0.23 & \underline{ -0.14 }  & \underline{ -0.09 }  & \underline{ -0.15 }  & -0.16 & \\ \hline 

\hspace{0pt}Lime &  \underline{ -0.16 }  & \underline{ -0.13 }  & \underline{ -0.09 }  & \underline{ -0.16 }  & \underline{ -0.09 }  & -0.13 & -0.24 & -0.19 & \underline{ -0.18 }  & \underline{ -0.11 }  & \underline{ -0.15 }  & -0.17 & \\ \hline 

\hspace{0pt}Occlusion &  \underline{ -0.11 }  & \underline{ -0.13 }  & \underline{ -0.04 }  & \underline{ -0.02 }  & \underline{ -0.02 }  & \underline{ -0.07 }  & \underline{ -0.11 }  & \underline{ -0.11 }  & \underline{ -0.03 }  & \underline{ 0.01 }  & \underline{ 0.01 }  & \underline{ -0.04 }  & \\ \hline 

\hspace{0pt}ShapleyValueSampling &  -0.16 & \underline{ -0.10 }  & \underline{ 0.02 }  & \underline{ -0.10 }  & \underline{ -0.11 }  & -0.10 & -0.23 & \underline{ -0.16 }  & \underline{ -0.16 }  & \underline{ -0.10 }  & \underline{ -0.13 }  & -0.16 & \\ \hline 

\hspace{0pt}SmoothGrad &  \underline{ -0.03 }  & \underline{ -0.08 }  & \underline{ 0.00 }  & \underline{ 0.04 }  & \underline{ -0.09 }  & \underline{ -0.03 }  & \underline{ -0.03 }  & \underline{ -0.07 }  & \underline{ 0.01 }  & \underline{ 0.00 }  & \underline{ -0.06 }  & \underline{ -0.03 }  & \\ 
\bottomrule
    \end{tabular}}
    \caption{
    Model-wise Spearman's correlation coefficient $r$ between prediction probability and heatmap plausibility measures of MSFI (left half) and FP (right half) on the knee task. We indicate the strongly positive correlated ones ($\geq 0.6$) in bold. Except for the correlation coefficients that are underlined, the remaining correlations are statistically significant.
    }
    \label{tab:spearman_knee}
\end{table*}
\FloatBarrier

\begin{table*}[!h]

    \centering
    \resizebox{\textwidth}{!}{\begin{tabular}{m{0.2\linewidth} *{5}{>{\centering\arraybackslash}m{0.08\linewidth}}{>{\centering\arraybackslash}m{0.1\linewidth}}|
    *{5}{>{\centering\arraybackslash}m{0.08\linewidth}{>{\centering\arraybackslash}m{0.1\linewidth}}}
    }
    \toprule
     & \multicolumn{6}{c}{\textbf{Knee}: \textbf{MSFI} correlation with \textbf{ground-truth} probability} & \multicolumn{6}{c}{\textbf{Knee}: \textbf{FP} correlation with \textbf{ground-truth} probability}\\

    \cline{2-13}
     & Model 6 & Model 7 & Model 8 & Model 9 & Model 10 & All & Model 6 & Model 7 & Model 8 & Model 9 & Model 10 & All \\
\hline

\hspace{0pt}Deconvolution &  \underline{ -0.09 }  & \underline{ -0.11 }  & \underline{ -0.16 }  & \underline{ -0.04 }  & \underline{ -0.18 }  & -0.12 & \underline{ -0.06 }  & \underline{ -0.09 }  & \underline{ -0.13 }  & \underline{ -0.05 }  & -0.20 & -0.11 & \\ \hline 

\hspace{0pt}FeatureAblation &  -0.26 & -0.22 & -0.31 & -0.22 & -0.25 & -0.25 & -0.29 & -0.24 & -0.26 & -0.26 & -0.26 & -0.26 & \\ \hline 

\hspace{0pt}Gradient &  \underline{ -0.12 }  & \underline{ -0.09 }  & \underline{ -0.09 }  & \underline{ -0.06 }  & \underline{ -0.13 }  & -0.10 & \underline{ -0.08 }  & \underline{ 0.00 }  & \underline{ -0.04 }  & \underline{ -0.07 }  & \underline{ -0.14 }  & \underline{ -0.08 }  & \\ \hline 

\hspace{0pt}GradientShap &  \underline{ -0.13 }  & \underline{ -0.10 }  & \underline{ -0.07 }  & \underline{ -0.06 }  & \underline{ -0.15 }  & -0.10 & \underline{ -0.09 }  & \underline{ -0.07 }  & \underline{ -0.03 }  & \underline{ -0.06 }  & \underline{ -0.13 }  & -0.08 & \\ \hline 

\hspace{0pt}GuidedBackProp &  \underline{ -0.08 }  & \underline{ -0.11 }  & \underline{ -0.16 }  & \underline{ -0.02 }  & -0.18 & -0.11 & \underline{ -0.06 }  & \underline{ -0.08 }  & \underline{ -0.13 }  & \underline{ -0.04 }  & -0.19 & -0.10 & \\ \hline 

\hspace{0pt}InputXGradient &  \underline{ -0.14 }  & \underline{ -0.11 }  & \underline{ -0.10 }  & \underline{ -0.05 }  & -0.21 & -0.12 & \underline{ -0.10 }  & \underline{ -0.03 }  & \underline{ -0.06 }  & \underline{ -0.04 }  & -0.20 & -0.10 & \\ \hline 

\hspace{0pt}IntegratedGradients &  \underline{ -0.06 }  & \underline{ -0.12 }  & \underline{ -0.14 }  & \underline{ 0.06 }  & \underline{ -0.12 }  & \underline{ -0.06 }  & \underline{ -0.06 }  & \underline{ -0.09 }  & \underline{ -0.14 }  & \underline{ 0.03 }  & \underline{ -0.10 }  & \underline{ -0.06 }  & \\ \hline 

\hspace{0pt}KernelShap &  -0.23 & -0.25 & -0.20 & -0.25 & -0.25 & -0.23 & -0.29 & -0.34 & -0.22 & -0.27 & -0.30 & -0.27 & \\ \hline 

\hspace{0pt}Lime &  -0.20 & \underline{ -0.15 }  & -0.22 & -0.22 & -0.25 & -0.21 & -0.28 & -0.25 & -0.24 & -0.26 & -0.31 & -0.26 & \\ \hline 

\hspace{0pt}Occlusion &  \underline{ -0.04 }  & \underline{ -0.10 }  & \underline{ -0.12 }  & \underline{ -0.05 }  & \underline{ -0.06 }  & -0.08 & \underline{ -0.02 }  & \underline{ -0.09 }  & \underline{ -0.09 }  & \underline{ -0.01 }  & \underline{ -0.05 }  & \underline{ -0.06 }  & \\ \hline 

\hspace{0pt}ShapleyValueSampling &  -0.16 & \underline{ -0.12 }  & \underline{ -0.08 }  & \underline{ -0.15 }  & -0.22 & -0.15 & -0.24 & -0.23 & -0.23 & -0.23 & -0.28 & -0.23 & \\ \hline 

\hspace{0pt}SmoothGrad &  \underline{ -0.05 }  & \underline{ -0.06 }  & \underline{ -0.07 }  & \underline{ -0.03 }  & \underline{ -0.14 }  & \underline{ -0.06 }  & \underline{ -0.01 }  & \underline{ -0.05 }  & \underline{ -0.04 }  & \underline{ -0.02 }  & \underline{ -0.14 }  & \underline{ -0.05 }  & \\ 

\bottomrule
    \end{tabular}}
    \caption{
    Model-wise Spearman's correlation coefficient $r$ between ground-truth probability and heatmap plausibility measures of MSFI (left half) and FP (right half) on the knee task. We indicate the strongly positive correlated ones ($\geq 0.6$) in bold. Except for the correlation coefficients that are underlined, the remaining correlations are statistically significant.
    }
    \label{tab:spearman_knee_gt}
\end{table*}
\FloatBarrier

\subsubsection{Testing for Plausibility Informativeness between Right and Wrong Predictions}
The statistical test for plausibility informativeness between correctly and incorrectly predicted data was conducted on test data points from all five models, because there was not sufficient sample size on the incorrectly predicted data group from a single model. In addition to the result reporting using MSFI in the manuscript, we reported the evaluation results using FP in Table~\ref{tab:eval_result_g4_fp} and Fig.~\ref{fig:fp}, which gave similar results to those using MSFI.
The model-wise MSFI and FP distributions for the correctly and incorrectly predicted data groups are visualized in Fig.~\ref{fig:LandscapeFigure-glioma} for the glioma task, and Fig.~\ref{fig:LandscapeFigure-knee} for the knee task.

\begin{table*}[!h]

    \centering
    \begin{tabular}{m{0.2\linewidth} *{3}{>{\centering\arraybackslash}m{0.1\linewidth}}|
    *{3}{>{\centering\arraybackslash}m{0.1\linewidth}}
    }
    \toprule
     & \multicolumn{3}{c}{FP on Glioma Task} & \multicolumn{3}{c}{FP on Knee Task}\\

    \cline{2-7}
     & Stat. Sig. & Right Pred. & Wrong Pred. & Stat. Sig. & Right Pred. & Wrong Pred.\\

\hline

Deconvolution & NS & 0.37 (0.33,0.40) & 0.40 (0.24,0.44) & NS & 0.23 (0.22,0.23) & 0.23 (0.22,0.24)\\ \hline

DeepLift & $\star$ & 0.71 (0.67,0.75) & 0.60 (0.44,0.72) & NaN & NaN & NaN\\ \hline

FeatureAblation & $\star\star$ & 0.47 (0.44,0.51) & 0.33 (0.19,0.48) & NS & 0.17 (0.16,0.18) & 0.21 (0.19,0.22)\\ \hline

FeaturePermutation & NS & 0.10 (0.07,0.13) & 0.06 (0.02,0.15) & NaN & NaN & NaN\\ \hline

GradCAM & NS & 0.02 (0.01,0.02) & 0.01 (0.01,0.02) & NaN & NaN & NaN\\ \hline

Gradient & NS & 0.30 (0.28,0.33) & 0.32 (0.23,0.37) & NS & 0.25 (0.24,0.25) & 0.25 (0.24,0.25)\\ \hline

GradientShap & NS & 0.63 (0.59,0.66) & 0.50 (0.39,0.62) & NS & 0.23 (0.22,0.23) & 0.22 (0.22,0.24)\\ \hline

GuidedBackProp & NS & 0.64 (0.61,0.67) & 0.58 (0.34,0.71) & NS & 0.25 (0.24,0.25) & 0.25 (0.24,0.26)\\ \hline

GuidedGradCAM & NS & 0.68 (0.66,0.71) & 0.57 (0.19,0.76) & NaN & NaN & NaN\\ \hline

InputXGradient & $\star$ & 0.65 (0.61,0.66) & 0.51 (0.33,0.63) & NS & 0.23 (0.23,0.23) & 0.24 (0.22,0.24)\\ \hline

IntegratedGradients & NS & 0.63 (0.59,0.67) & 0.51 (0.37,0.65) & NS & 0.22 (0.21,0.23) & 0.22 (0.21,0.23)\\ \hline

KernelShap & NS & 0.10 (0.08,0.12) & 0.09 (0.01,0.22) & NS & 0.16 (0.16,0.17) & 0.19 (0.18,0.20)\\ \hline

Lime & NS & 0.12 (0.09,0.14) & 0.12 (0.07,0.16) & NS & 0.17 (0.16,0.18) & 0.20 (0.19,0.20)\\ \hline

Occlusion & NS & 0.24 (0.21,0.27) & 0.14 (0.09,0.27) & NS & 0.19 (0.19,0.20) & 0.19 (0.18,0.20)\\ \hline

ShapleyValueSampling & NS & 0.37 (0.35,0.42) & 0.30 (0.17,0.40) & NS & 0.19 (0.19,0.20) & 0.22 (0.20,0.23)\\ \hline

SmoothGrad & NS & 0.32 (0.29,0.35) & 0.33 (0.18,0.39) & NS & 0.25 (0.24,0.25) & 0.25 (0.23,0.26)\\ 

\bottomrule
    \end{tabular}
    \caption{\textbf{Evaluation results on Guideline 4 - Testing for plausibility informativeness using FP metric}. The median and 95\% confidence interval of the FP metric for the correctly and incorrectly predicted data groups are shown in their corresponding columns, for the glioma and knee tasks, respectively. 
    The statistical significance columns report FP distribution significance results between right and wrong predictions using a upper-tailed Mann–Whitney U test: $\star$ indicates $p<0.025$; $\star\star$ for $p<0.005$; $\star\star\star$ for
    $p<0.0005$; NS for not significant. 
    ``NaN'' in the knee task is because the XAI method was not included in the evaluation. XAI methods are in alphabetic order. 
    }
    \label{tab:eval_result_g4_fp}
\end{table*}
\FloatBarrier

\begin{figure}
    \centering
    \includegraphics[width=\textwidth]{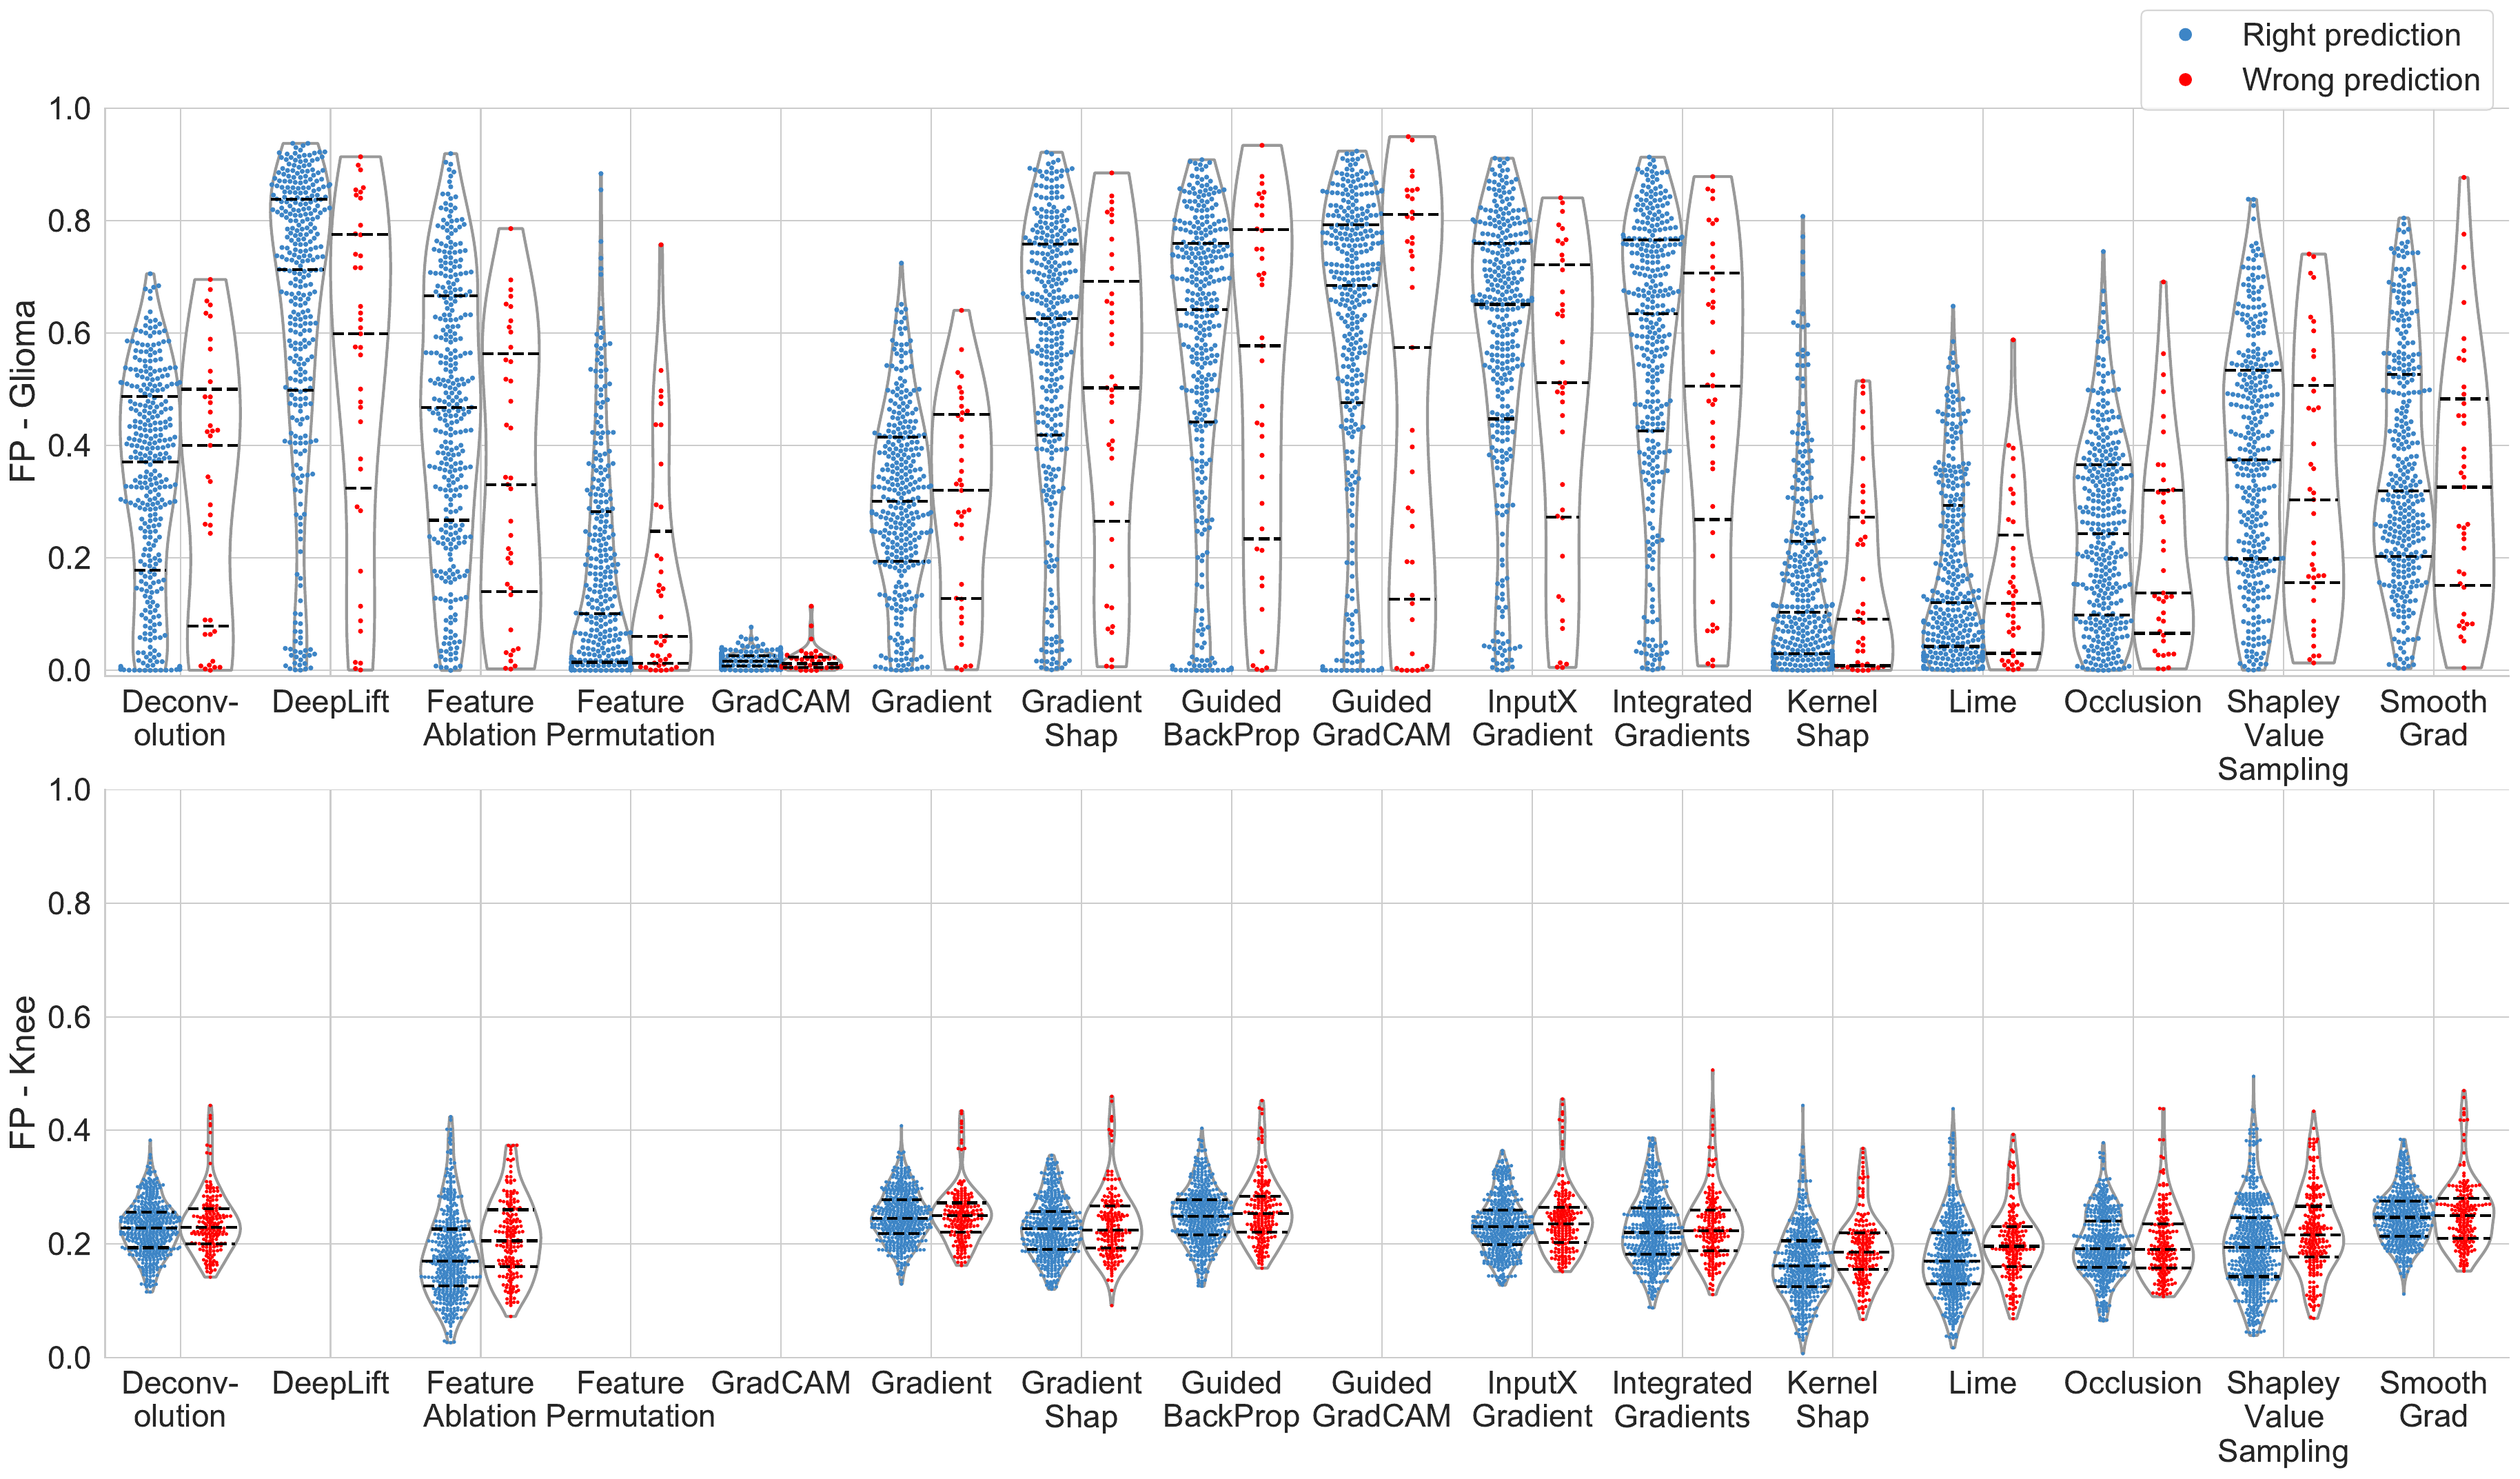}
    \caption{\textbf{Evaluation results on Guideline 4 - Testing for plausibility informativeness using FP metric.} 
    For each heatmap method (X-axis), the violin and swarm plots show the plausibility quantification score distribution of FP for the right (blue, left) and wrong (red, right) predictions on the glioma (top) and knee task (bottom). Each dot is a data sample in the test set, and we aggregate results from five similarly-trained models. Y-axis is the FP measure, with a higher score indicating more agreeable of a heatmap with clinical prior knowledge on tumor mask. The black dashed lines indicate the quartiles of each distribution.
}
    \label{fig:fp}
\end{figure}
\FloatBarrier

\begin{sidewaysfigure}[ht]
    \includegraphics[width=\textwidth]{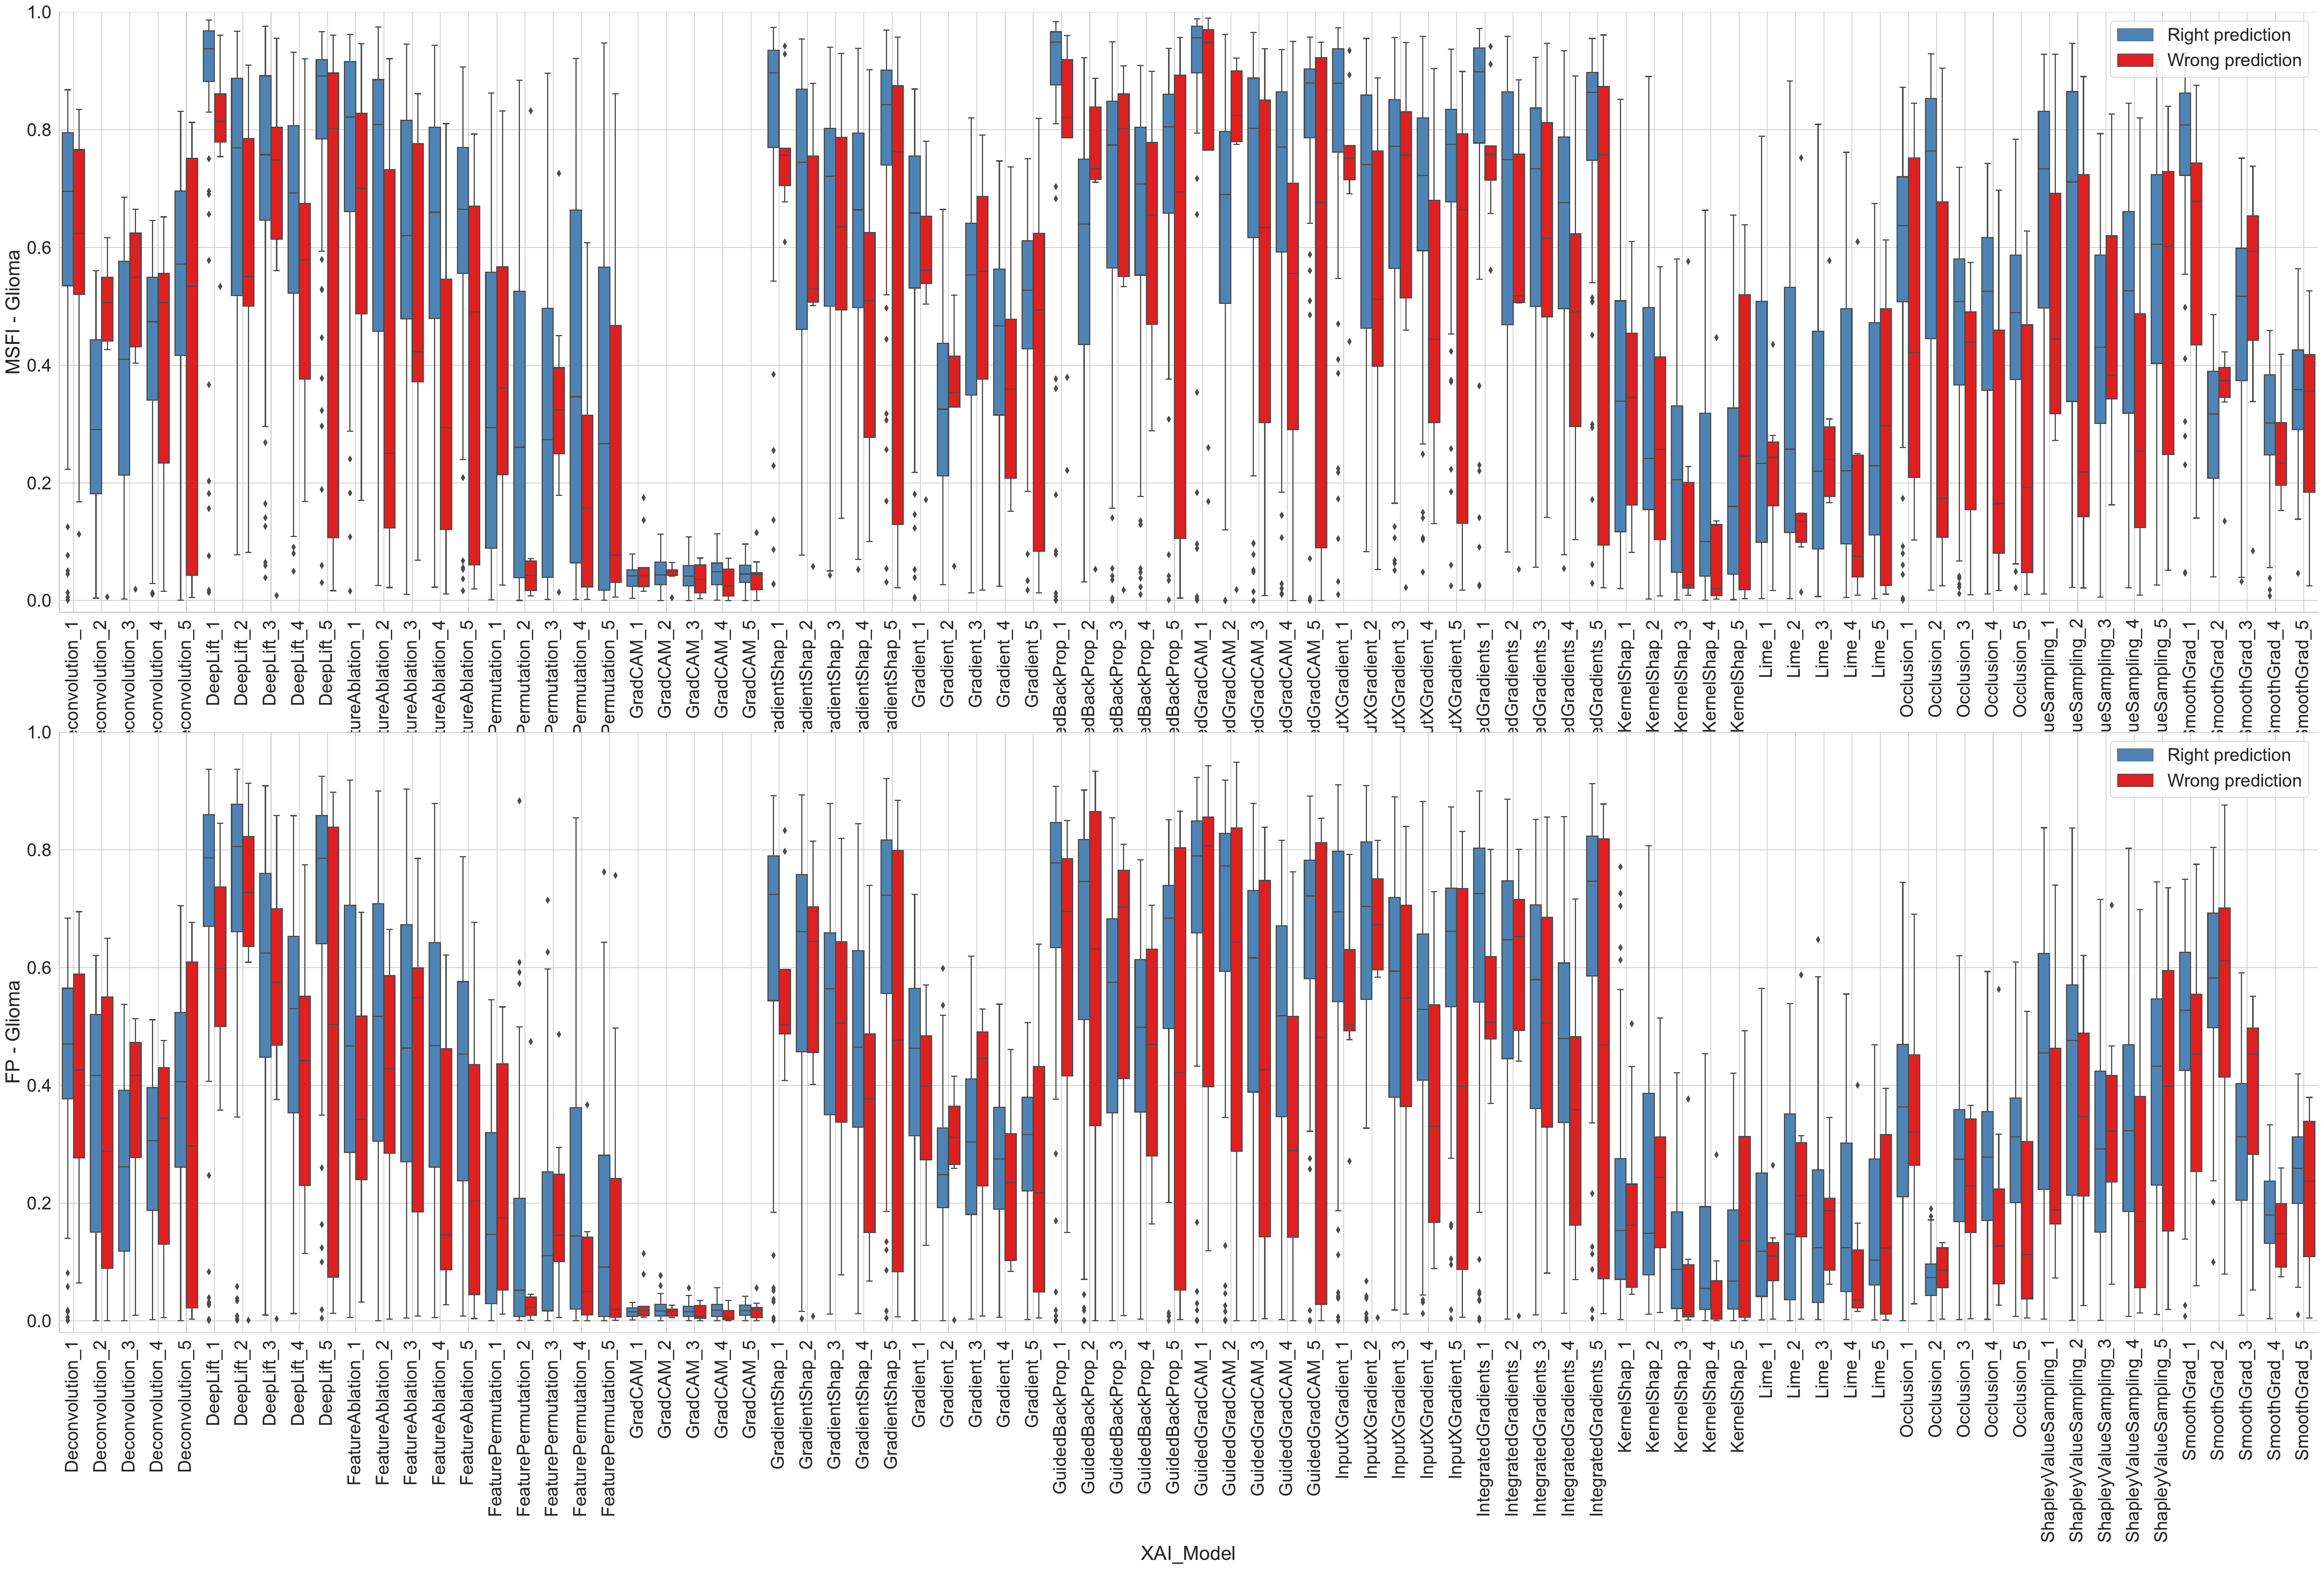}
    \caption{\textbf{Model-wise evaluation results on Guideline 4 - Testing for plausibility informativeness on the glioma task.} The box plots show the distribution difference of MSFI (top) and FP (bottom) metric between the correctly/incorrectly predicted subgroups of five models.}
    \label{fig:LandscapeFigure-glioma}
\end{sidewaysfigure}
\FloatBarrier

\begin{sidewaysfigure}[ht]
    \includegraphics[width=\textwidth]{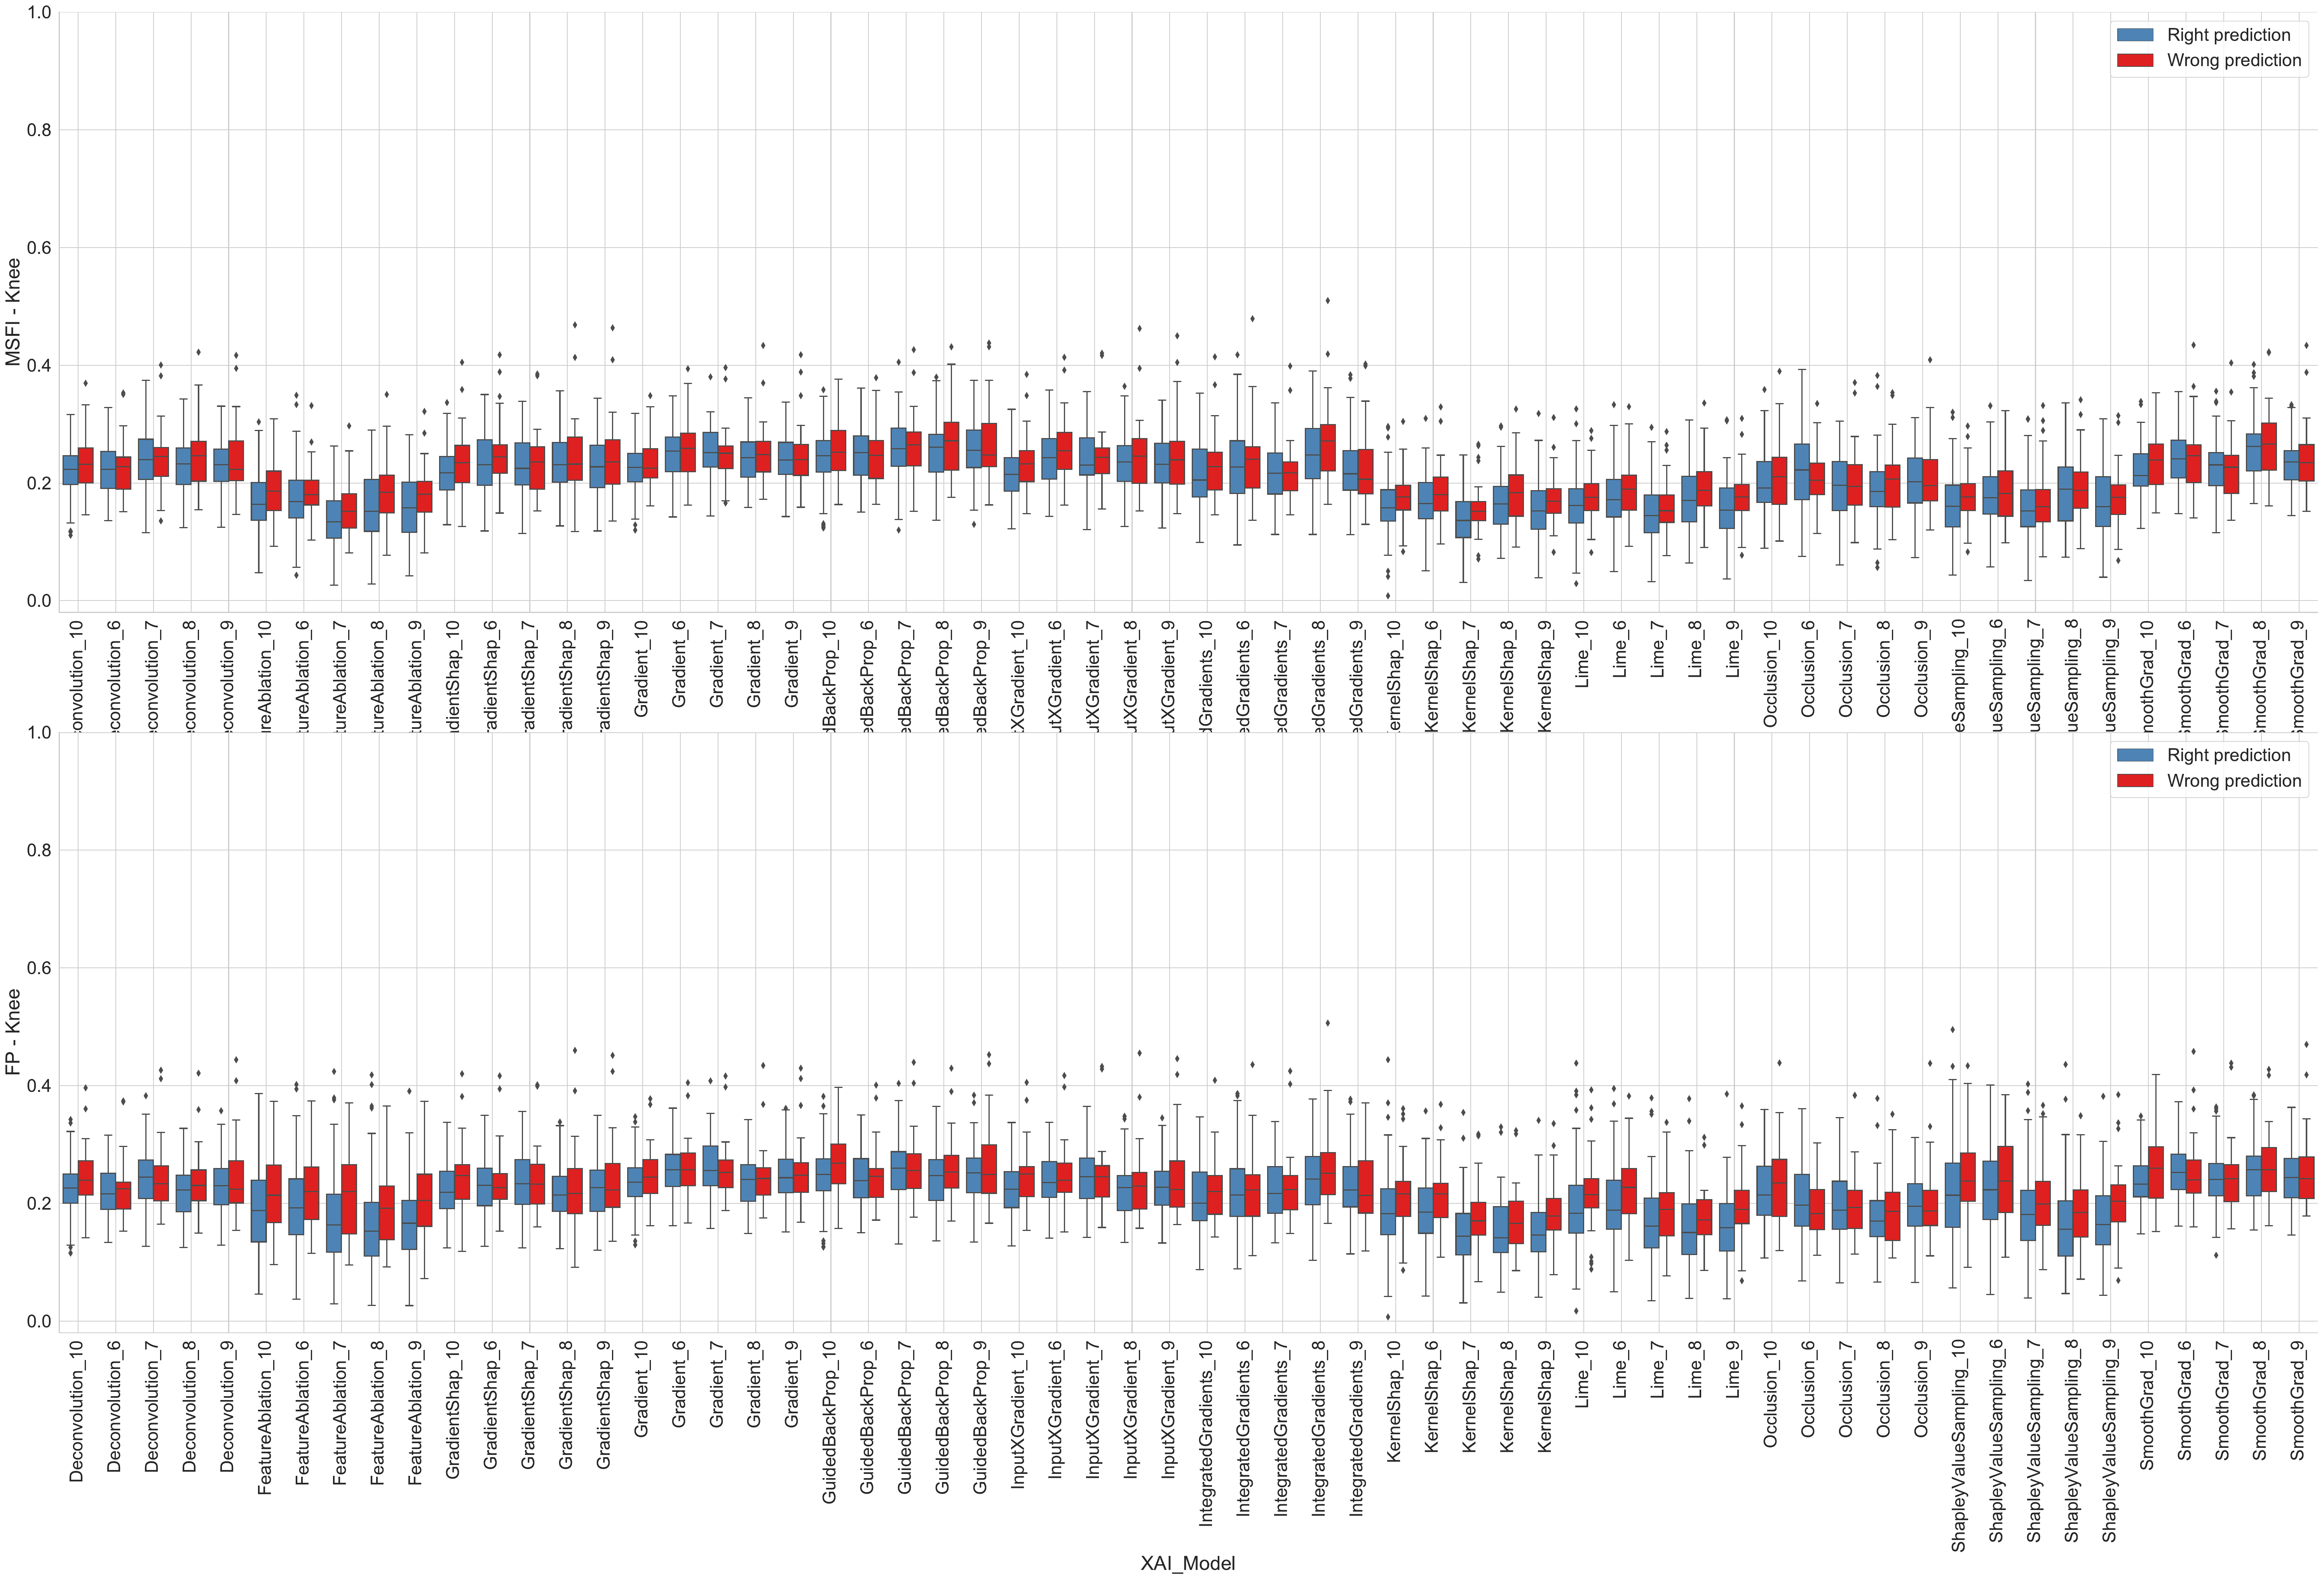}
    \caption{\textbf{Model-wise evaluation results on Guideline 4 - Testing for plausibility informativeness on the knee task.} The box plots show the distribution difference of MSFI (top) and FP (bottom) metric between the correctly/incorrectly predicted subgroups of five models.}
    \label{fig:LandscapeFigure-knee}
\end{sidewaysfigure}
\FloatBarrier

In addition to the statistical test on correctly and incorrectly predicted data unconditioned on their labels, next we conducted additional analysis conditioned on each target (predicted or ground-truth) class.

The first step is to test if the plausibility metrics have different distributions on different labels.
For the glioma task, Mann-Whitney U test showed both the predicted and ground-truth HGG label had a significantly higher ($p <0.0005$) MSFI score compared to LGG (Fig.~\ref{fig:conditioned_MSFI}). Statistical test using FP metric also showed the same results (Fig.~\ref{fig:conditioned_FP}).
The different pattern of heatmaps on HGG and LGG class can be visualized in Fig.~\ref{fig:hgg_lgg}, in it heatmaps for HGG class tend to focus on the tumor region, whereas heatmaps for LGG class pay more attention to regions outside tumor.

\begin{figure}[!h]
    \centering
    \includegraphics[width=\textwidth]{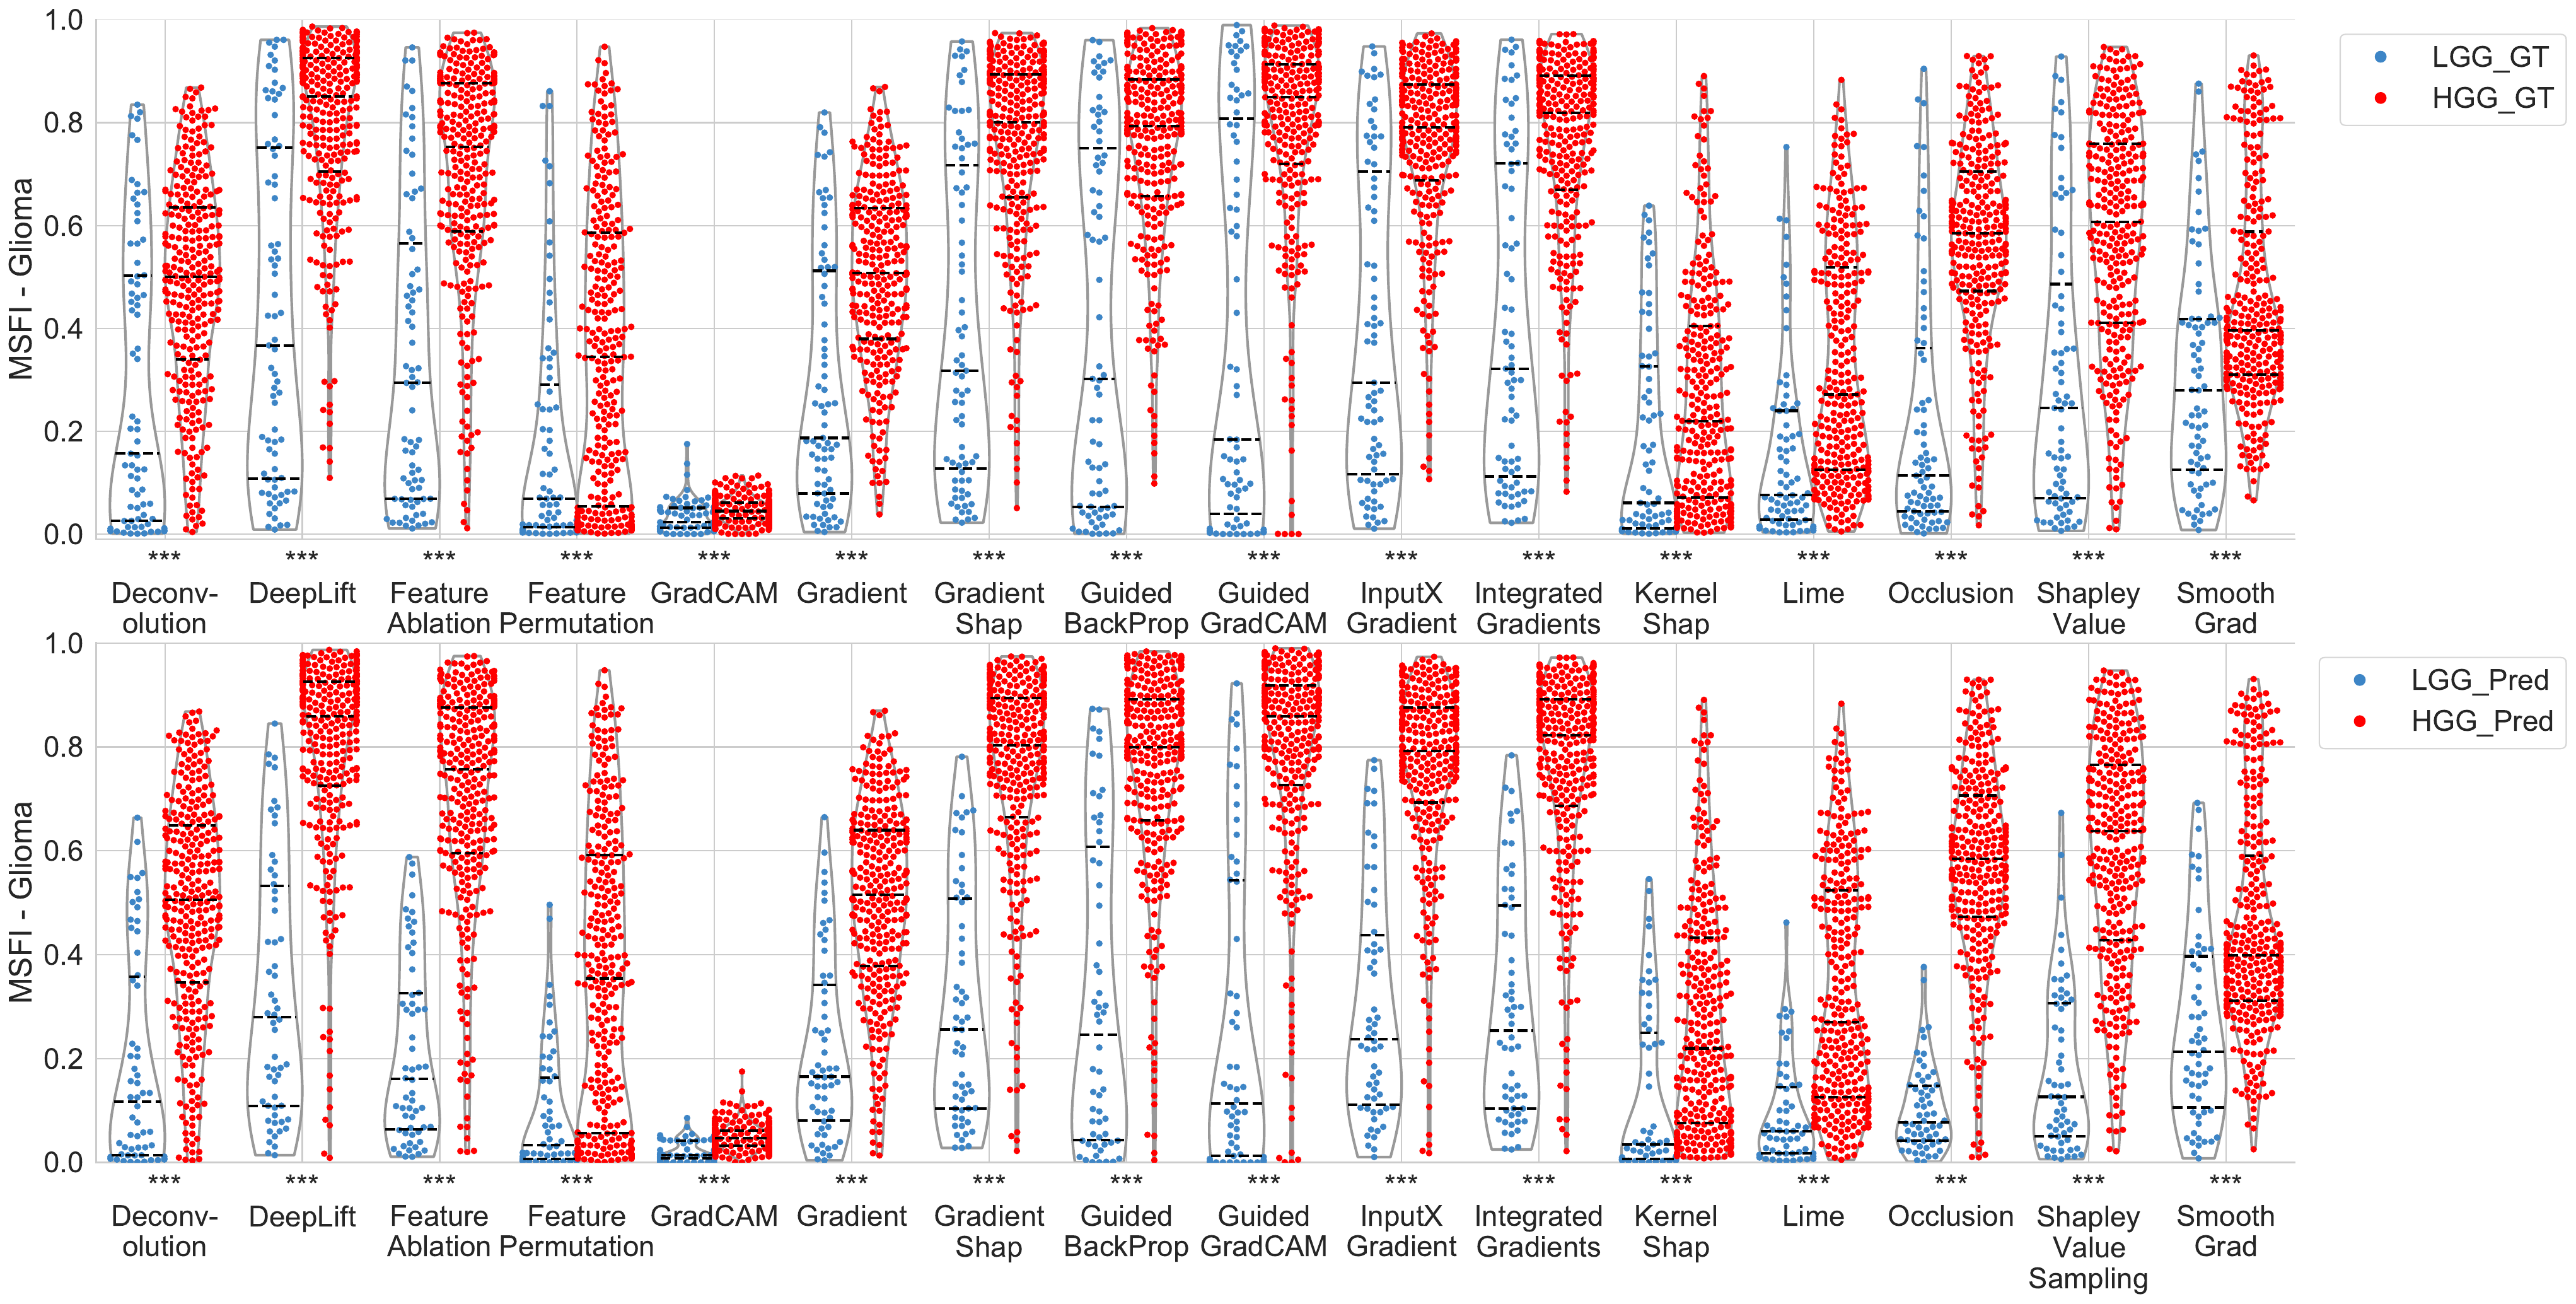}
    \caption{\textbf{MSFI distribution conditioned on the LGG and HGG class for the glioma task.} The top and bottom plots are MSFI distribution conditioned on the \textit{ground truth} and \textit{prediction} label of LGG and HGG, respectively. Statistical significance level that HGG has higher MSFI than LGG is indicated for each XAI: $*$ indicates $p<0.025$; $**$ for $p<0.005$; $***$ for $p<0.0005$, the same for the plots below.}
    \label{fig:conditioned_MSFI}
\end{figure}
\FloatBarrier
\begin{figure}[!h]
    \centering
    \includegraphics[width=\textwidth]{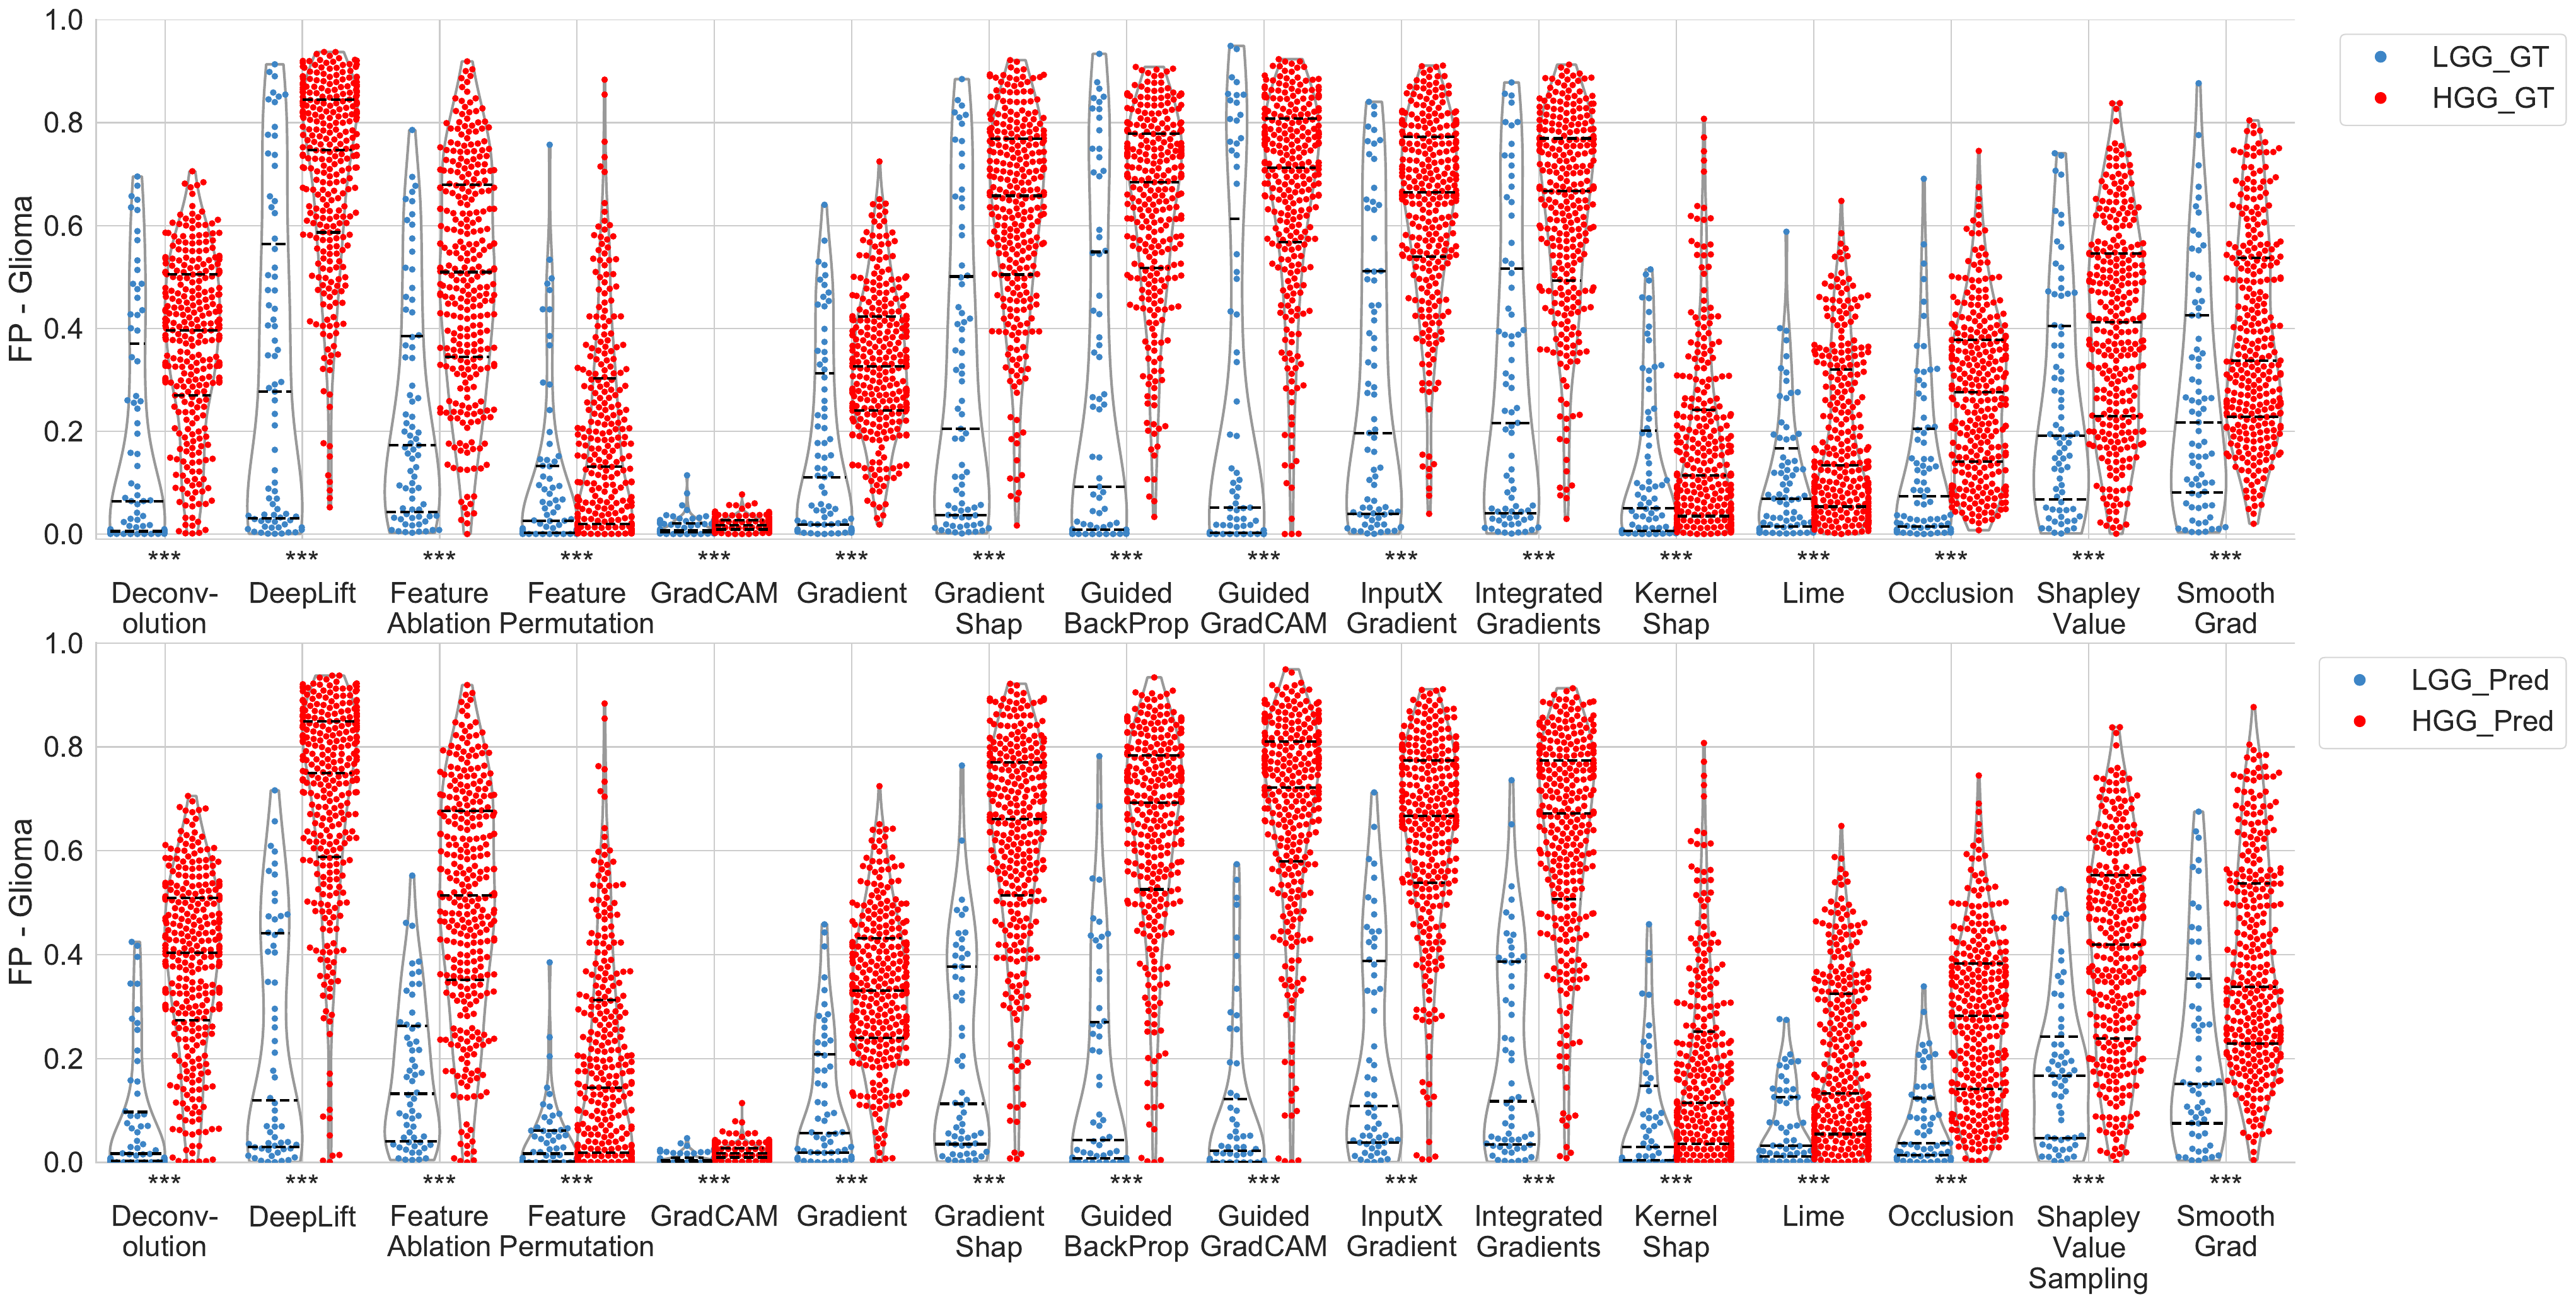}
    \caption{\textbf{FP distribution conditioned on the LGG and HGG class for the glioma task.} The top and bottom plots are FP distribution conditioned on the \textit{ground truth} and \textit{prediction} label of LGG and HGG, respectively. 
    }
    \label{fig:conditioned_FP}
\end{figure}
\FloatBarrier

The knee task also showed plausibility metric difference on different labels: for most XAI methods, the MSFI or FP distribution is significantly higher for the positive class (meniscus tear) than the negative class (intact) on the prediction labels. But when conditioned on the ground-truth labels, the plausibility distribution did not show statistical difference. 
The significant level is indicated using $*$ in front of each XAI method name in Fig.~\ref{fig:conditioned_MSFI_knee} and \ref{fig:conditioned_FP_knee}.

\begin{figure}[!h]
    \centering
    \includegraphics[width=\textwidth]{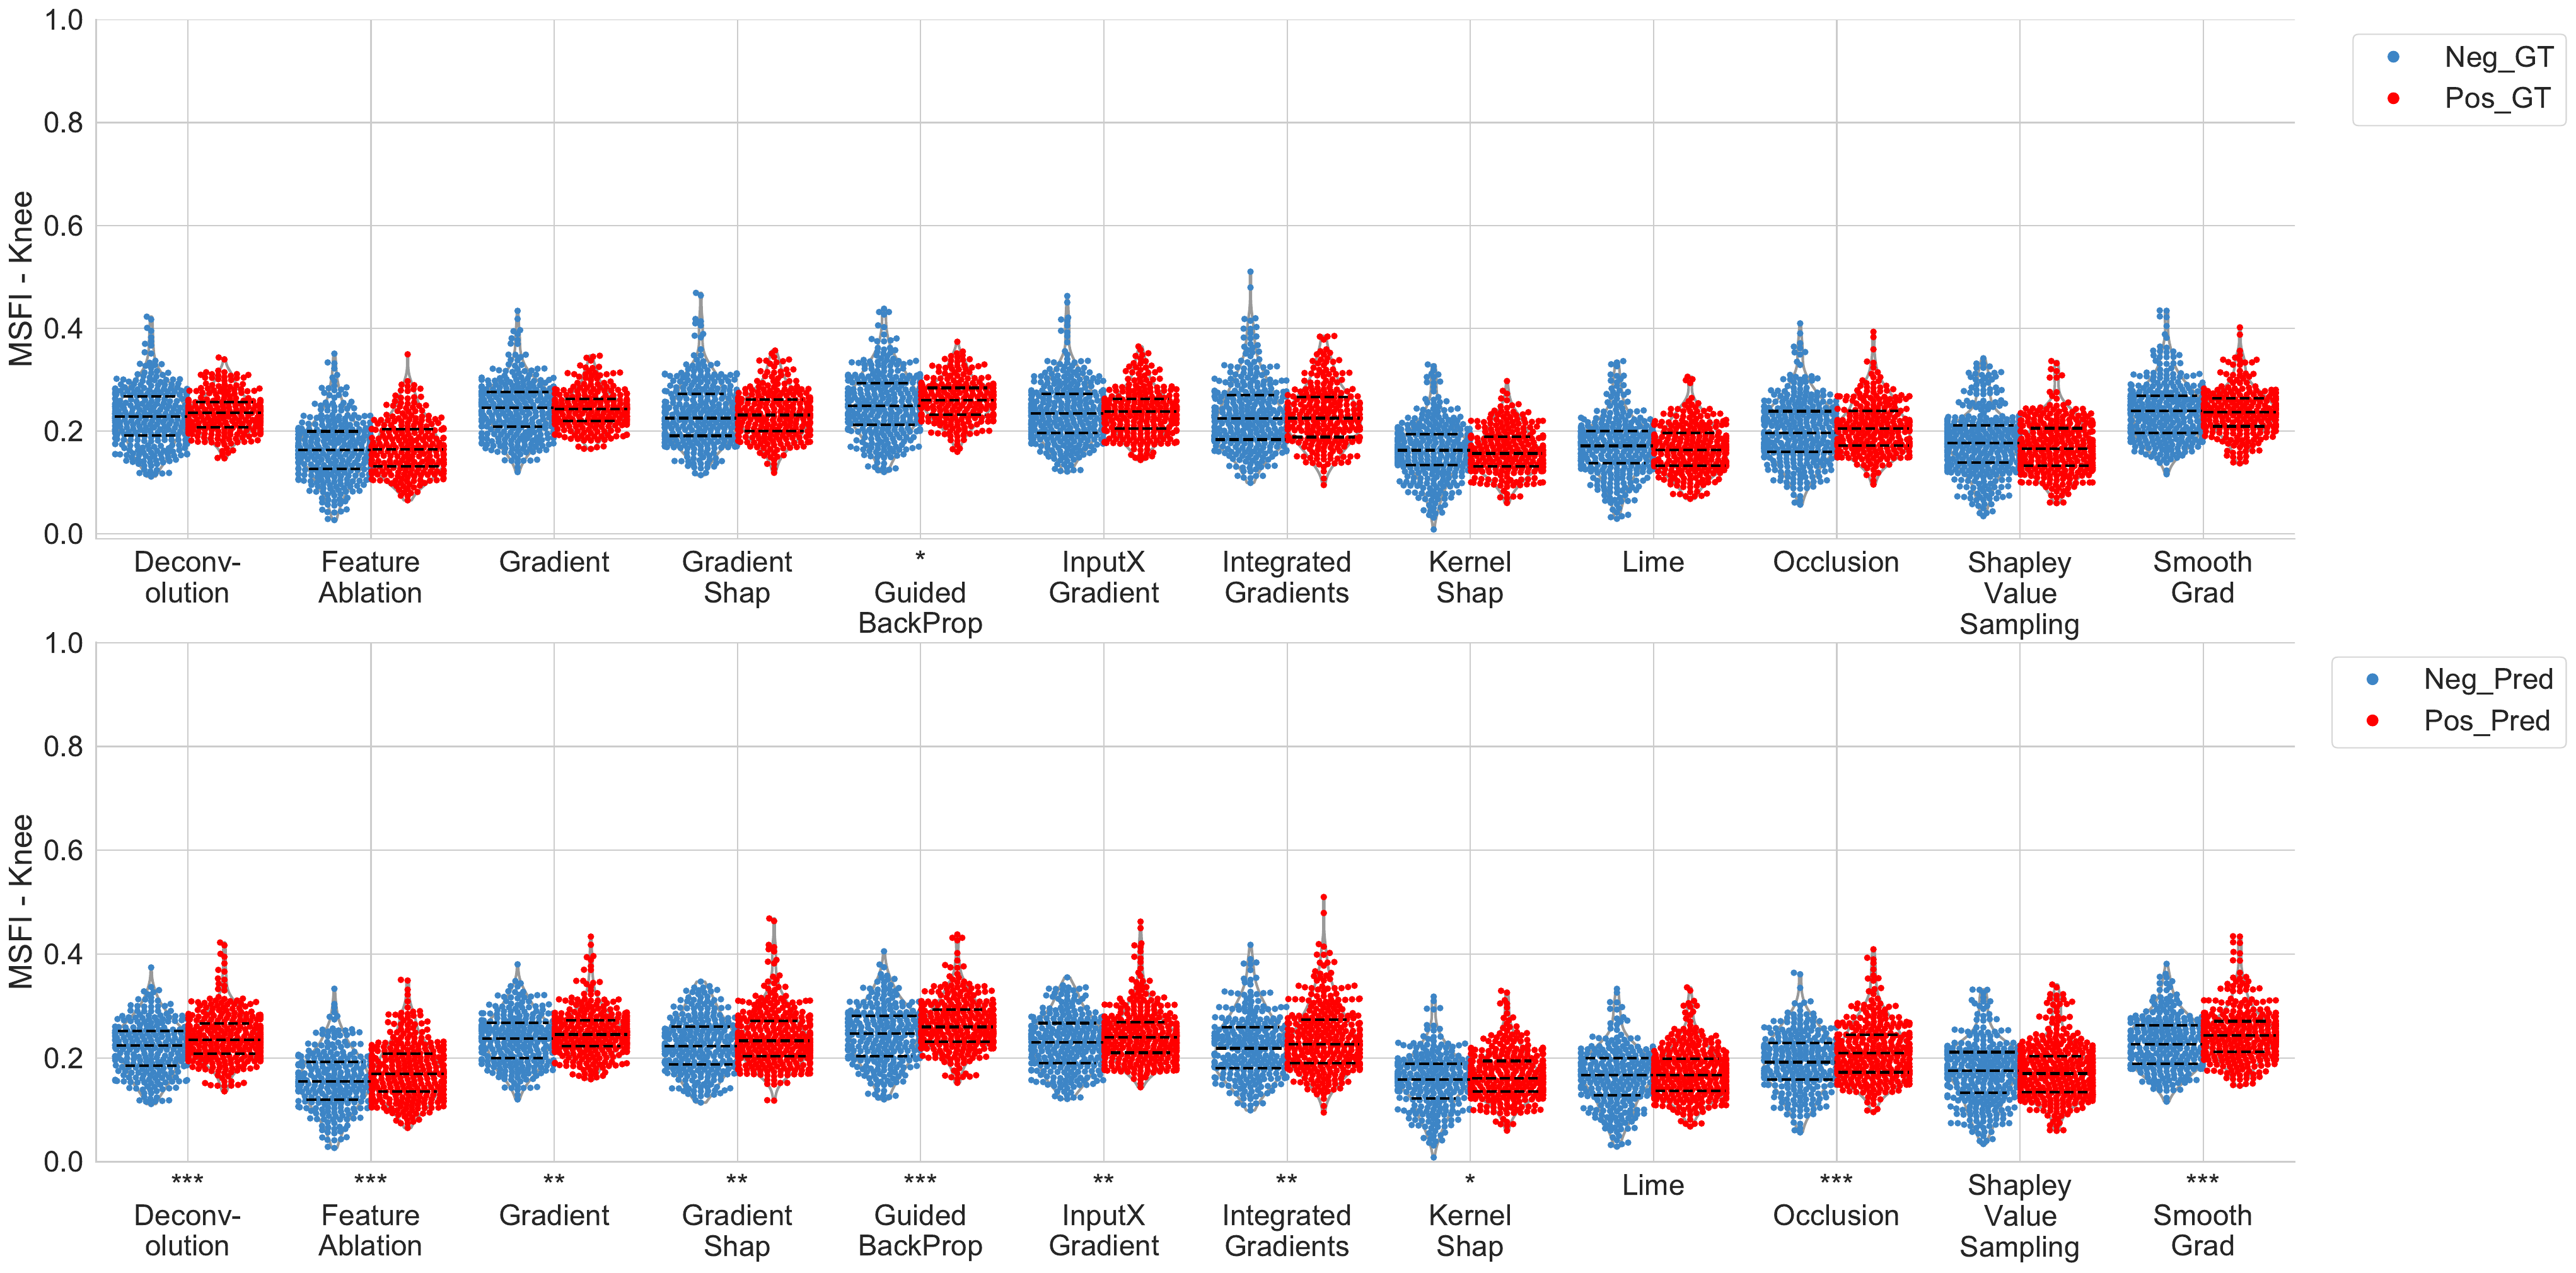}
    \caption{\textbf{MSFI distribution conditioned on positive and negative classes for the knee task.} The top and bottom plots are MSFI distribution conditioned on the \textit{ground truth} and \textit{prediction} labels of negative and positive class, respectively. }
    \label{fig:conditioned_MSFI_knee}
\end{figure}
\FloatBarrier
\begin{figure}[!h]
    \centering
    \includegraphics[width=\textwidth]{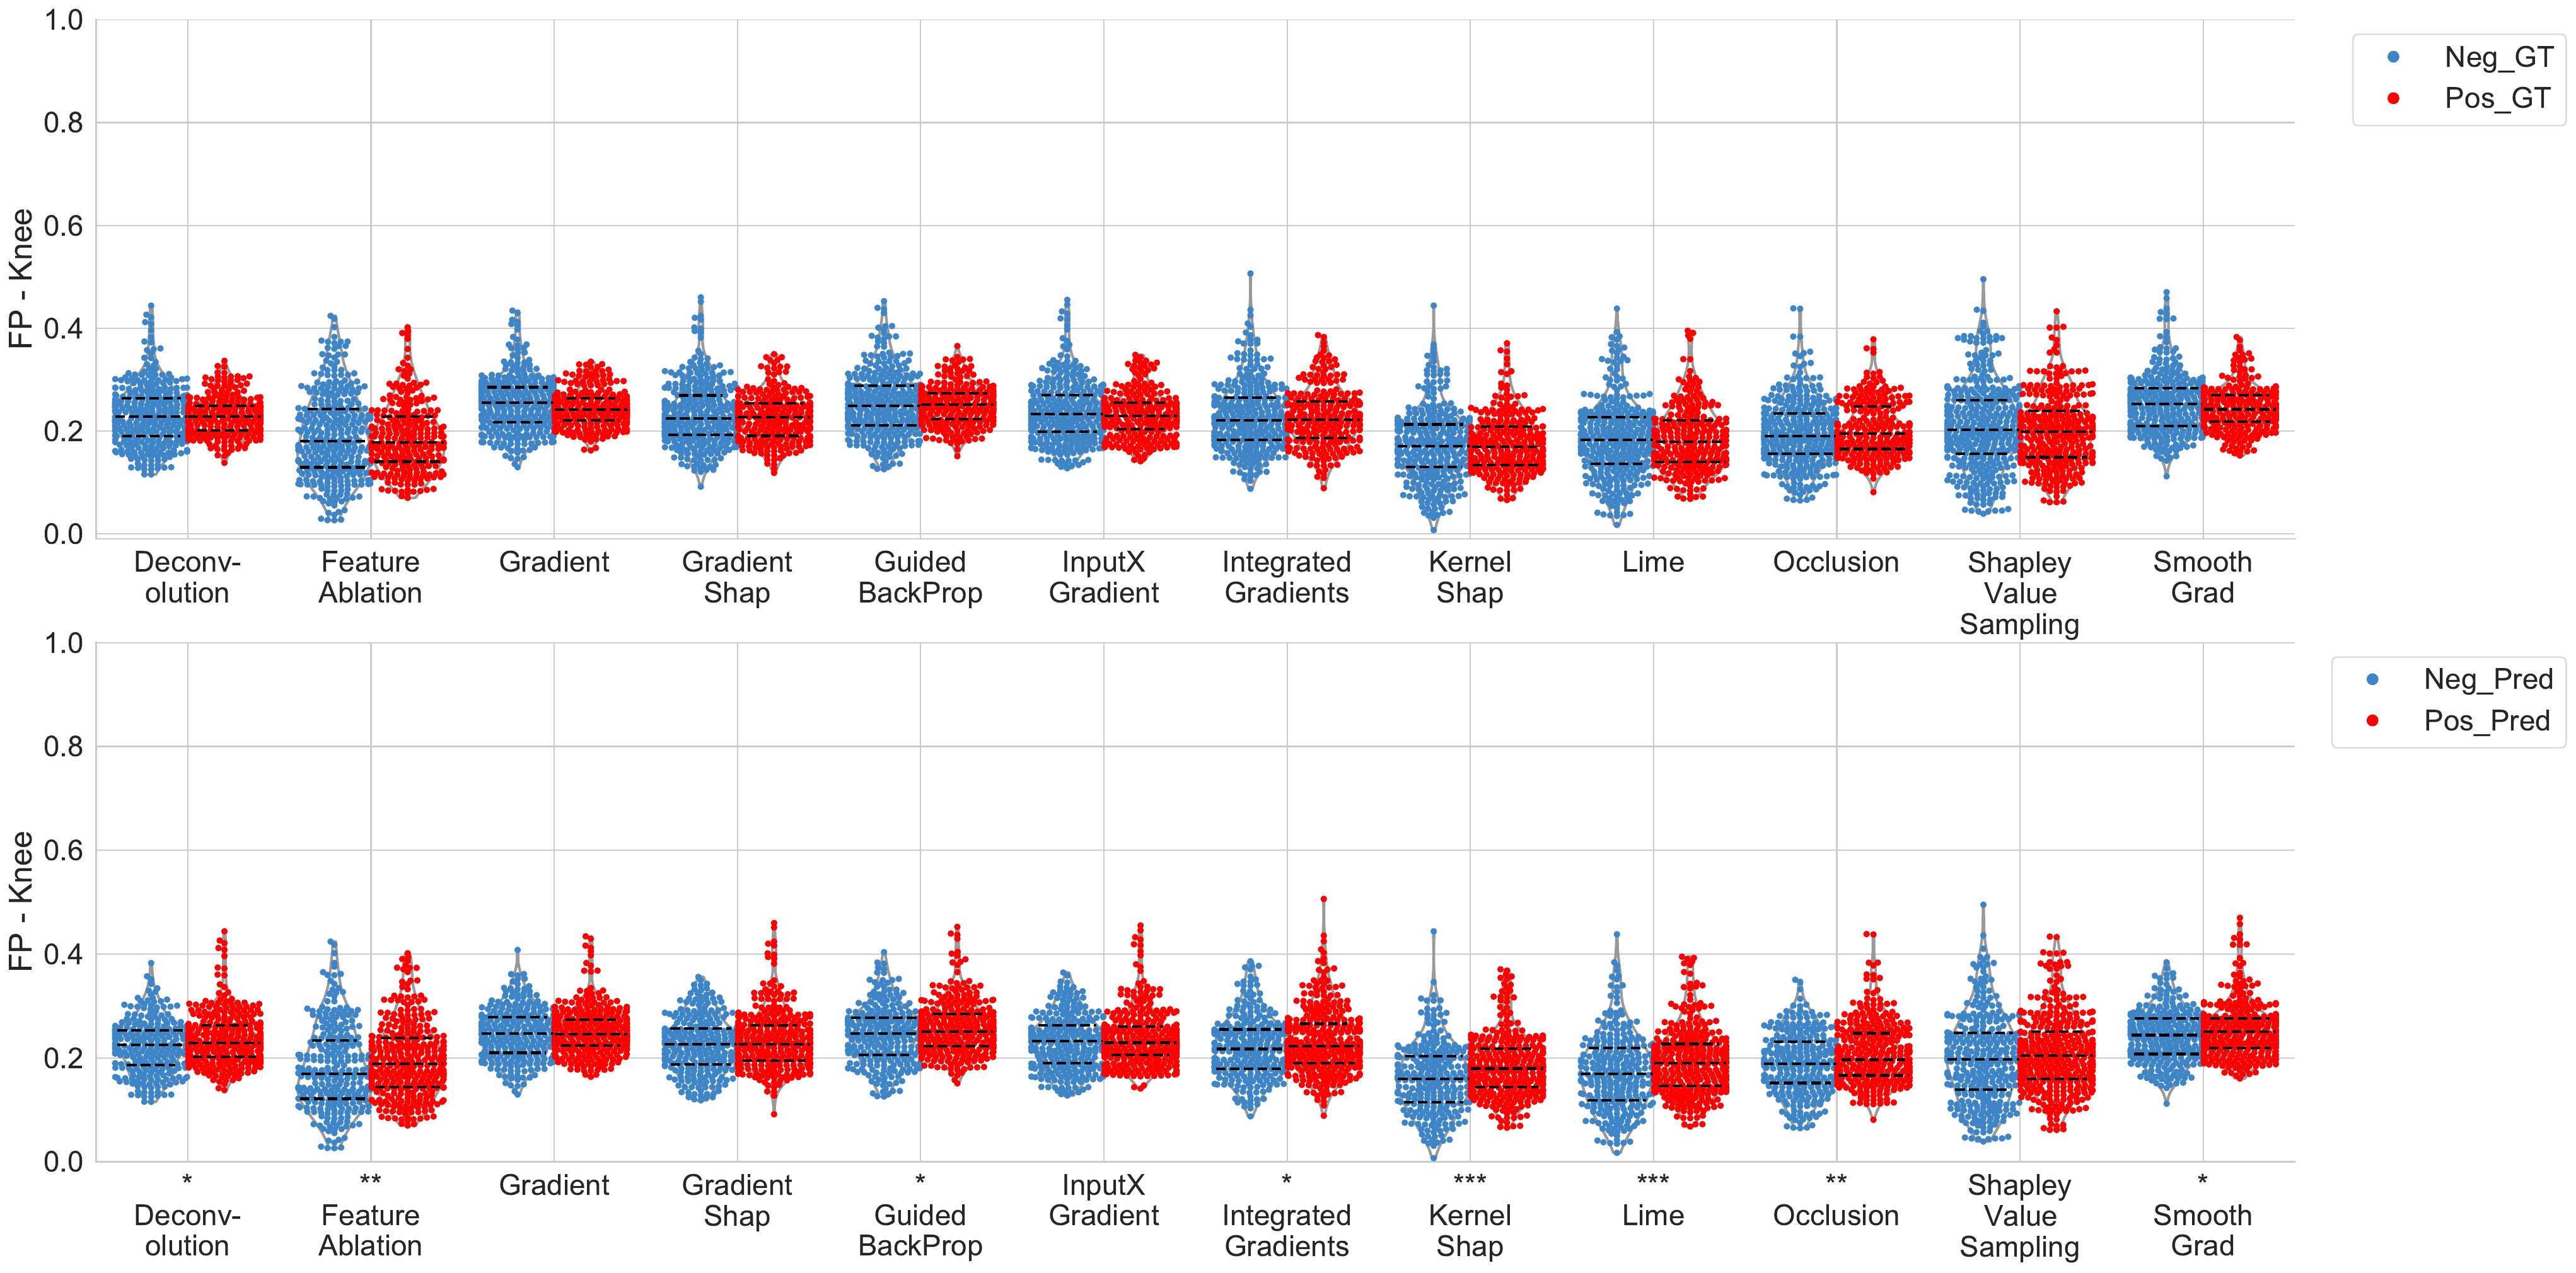}
    \caption{\textbf{FP distribution conditioned on positive and negative classes for the knee task.} The top and bottom plots are FP distribution conditioned on the \textit{ground truth} and \textit{prediction} labels of negative and positive class, respectively. 
    }
    \label{fig:conditioned_FP_knee}
\end{figure}
\FloatBarrier

Because the plausibility measure had different distributions conditioned on class labels, in the second step, we conducted the same testing for plausibility informativeness conditioned on the different labels on both tasks. 

For the glioma task, the significant level of Mann-Whitney U test on whether right predictions have higher MSFI than wrong predictions is indicated in front of each XAI method in Fig.~\ref{fig:class_conditioned_MSFI_pred} and \ref{fig:class_conditioned_MSFI_gt}. Results showed when conditioned on the predicted labels, most XAI methods did not show significant higher MSFI on correctly predicted data than incorrectly predicted ones, for both LGG and HGG class, except for Occlusion and Feature Ablation conditioned on predicted HGG labels, with $p = 0.003$ and $0.01$ respectively. Further visualization in Fig.~\ref{fig:class_conditioned_MSFI_pred} however, still showed MSFI range overlapping for right and wrong predictions in Occlusion and Feature Ablation. This showed that despite being conditioned on a certain predicted label, users still could not tell the wrong predictions from the right ones by plausibility assessment. Therefore, the examined XAI methods did not fulfill G4 Informative plausibility test when conditioned on each predicted label on the glioma task.

Plausibility informativeness testing conditioned on the \textit{predicted} labels (Fig.~\ref{fig:class_conditioned_MSFI_pred}) has more clinical utility than conditioned on the \textit{ground-truth} labels (Fig.~\ref{fig:class_conditioned_MSFI_gt}), because in the real-world usage of AI, conditioned on ground-truth labels cannot be acquired for new data when ground-truth is unavailable. Results showed when conditioned on the ground-truth label of HGG, many XAI methods showed significance (Fig.~\ref{fig:class_conditioned_MSFI_gt}-top). And when conditioned on the ground-truth label of LGG, no XAI methods showed significance (Fig.~\ref{fig:class_conditioned_MSFI_gt}-bottom). The significance shown on the ground-truth HGG label is because when conditioned on the ground-truth HGG label, the right and wrong predictions are predicted HGG and predicted LGG, and the statistical significance only reflects the previous finding (Fig.~\ref{fig:conditioned_MSFI}) that MSFI distribution is higher for the predicted HGG than the predicted LGG.

\begin{figure}[!h]
    \centering
    \includegraphics[width=\textwidth]{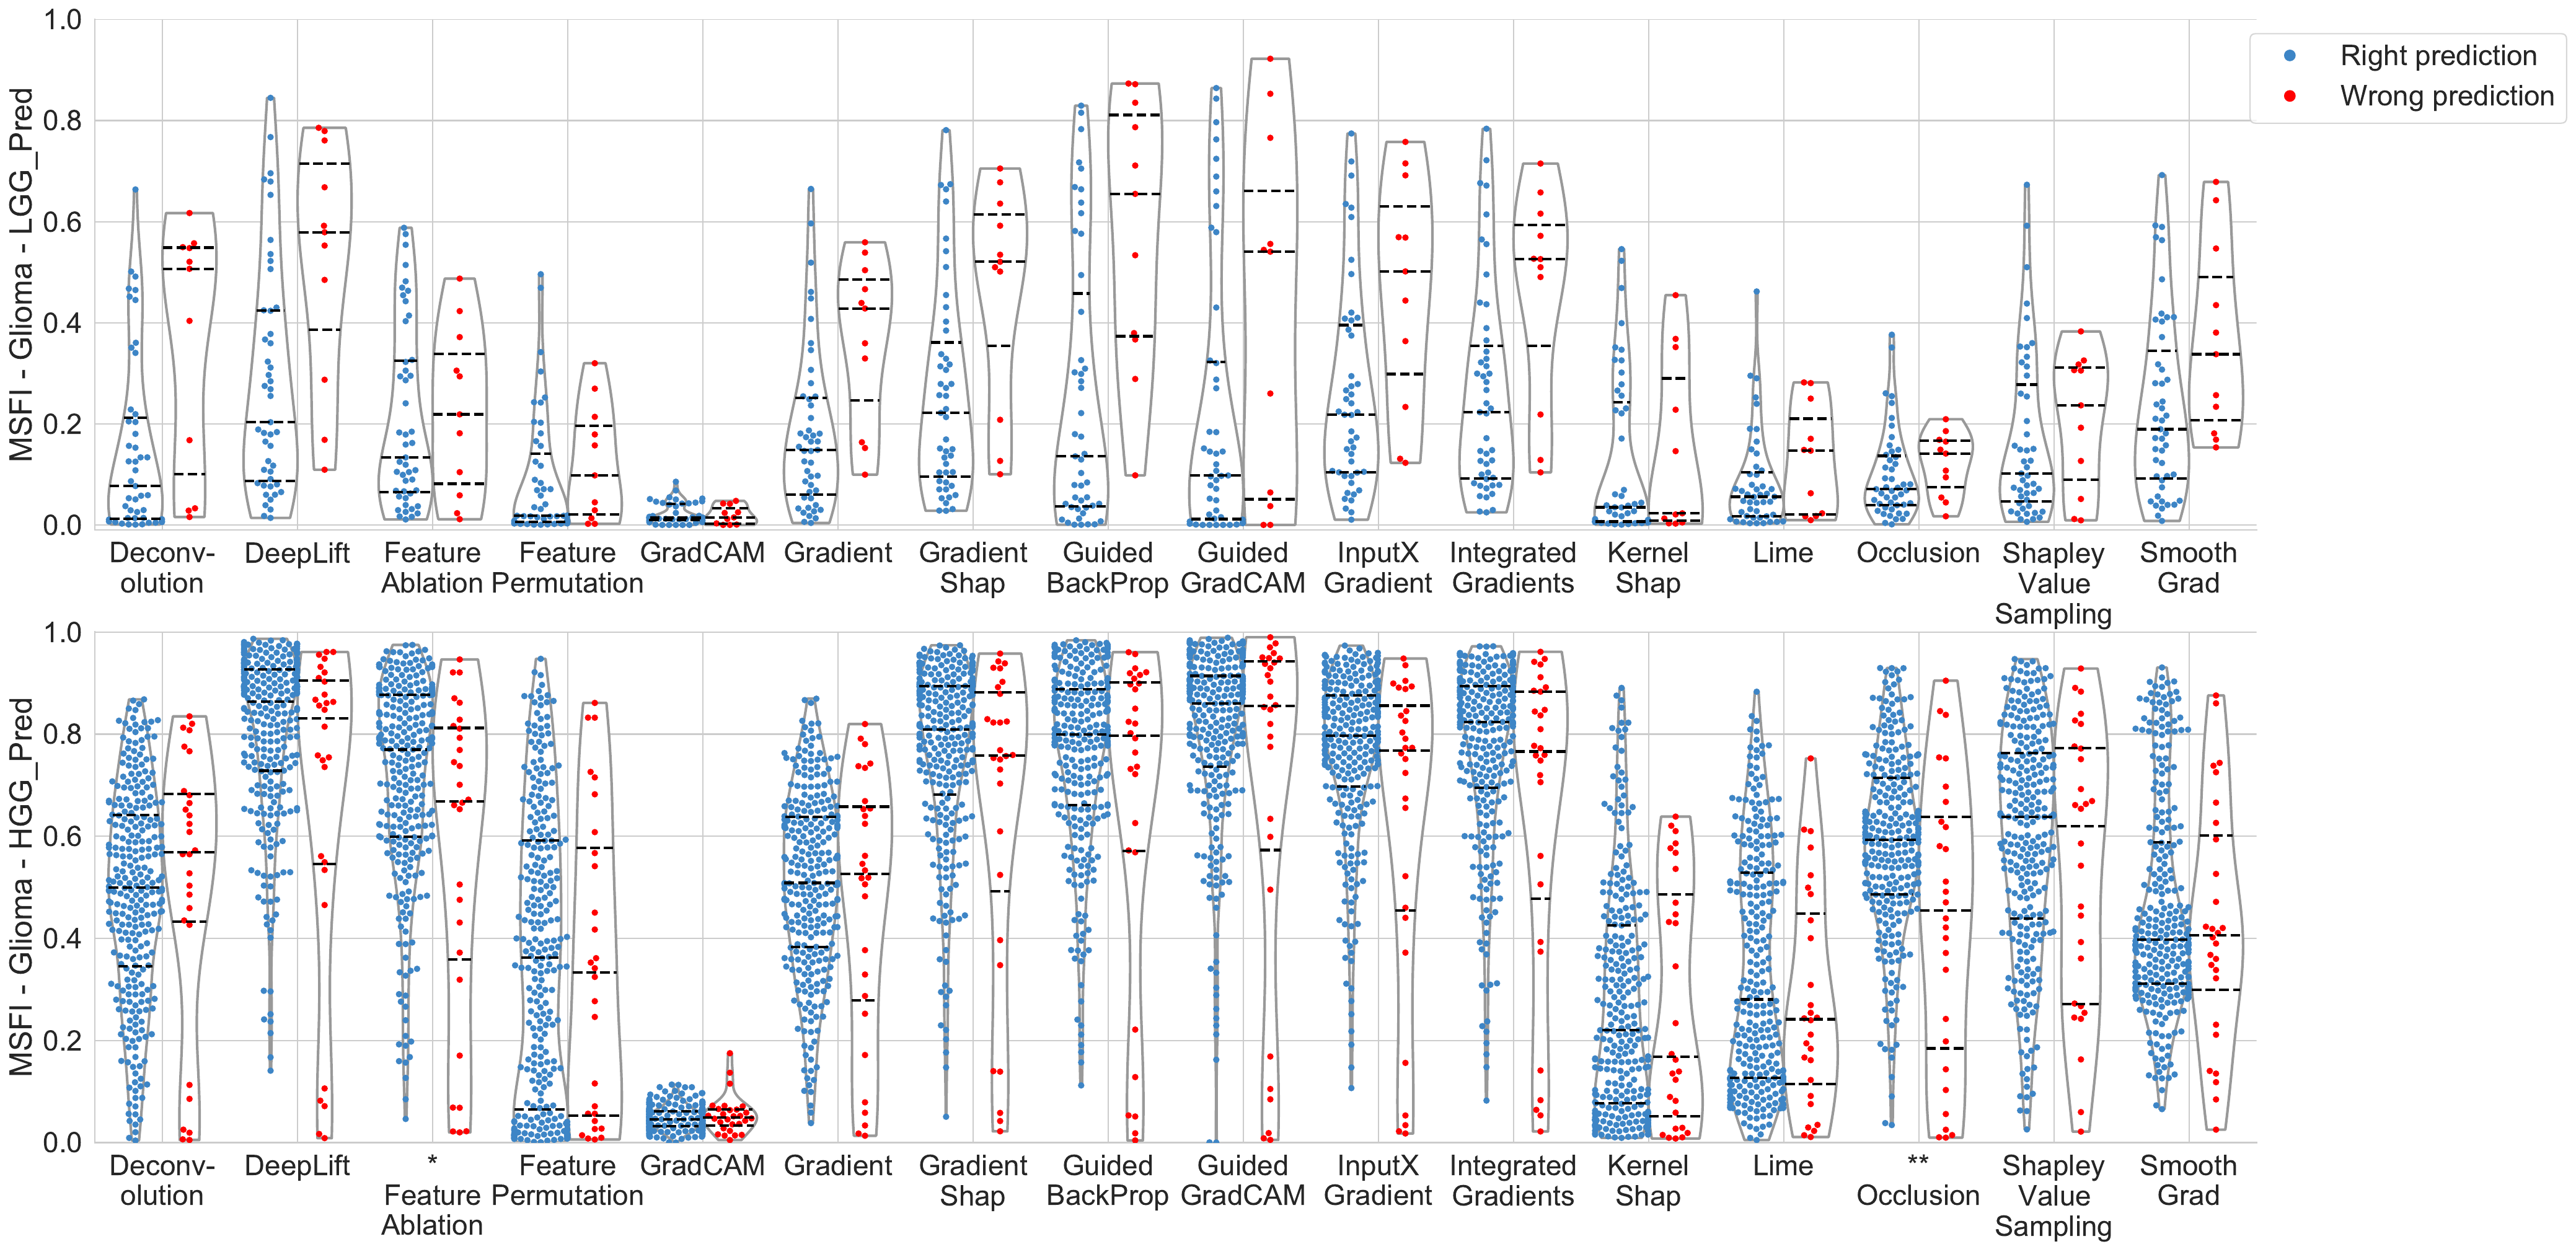}
    \caption{\textbf{MSFI distribution conditioned on the \textit{predicted} labels of LGG and HGG on glioma task.} The swarm and violin plots visualize MSFI distributions of right and wrong predictions conditioned on the predicted labels of LGG (top) and HGG (bottom), respectively.}
    \label{fig:class_conditioned_MSFI_pred}
\end{figure}
\FloatBarrier

\begin{figure}[!h]
    \centering
    \includegraphics[width=\textwidth]{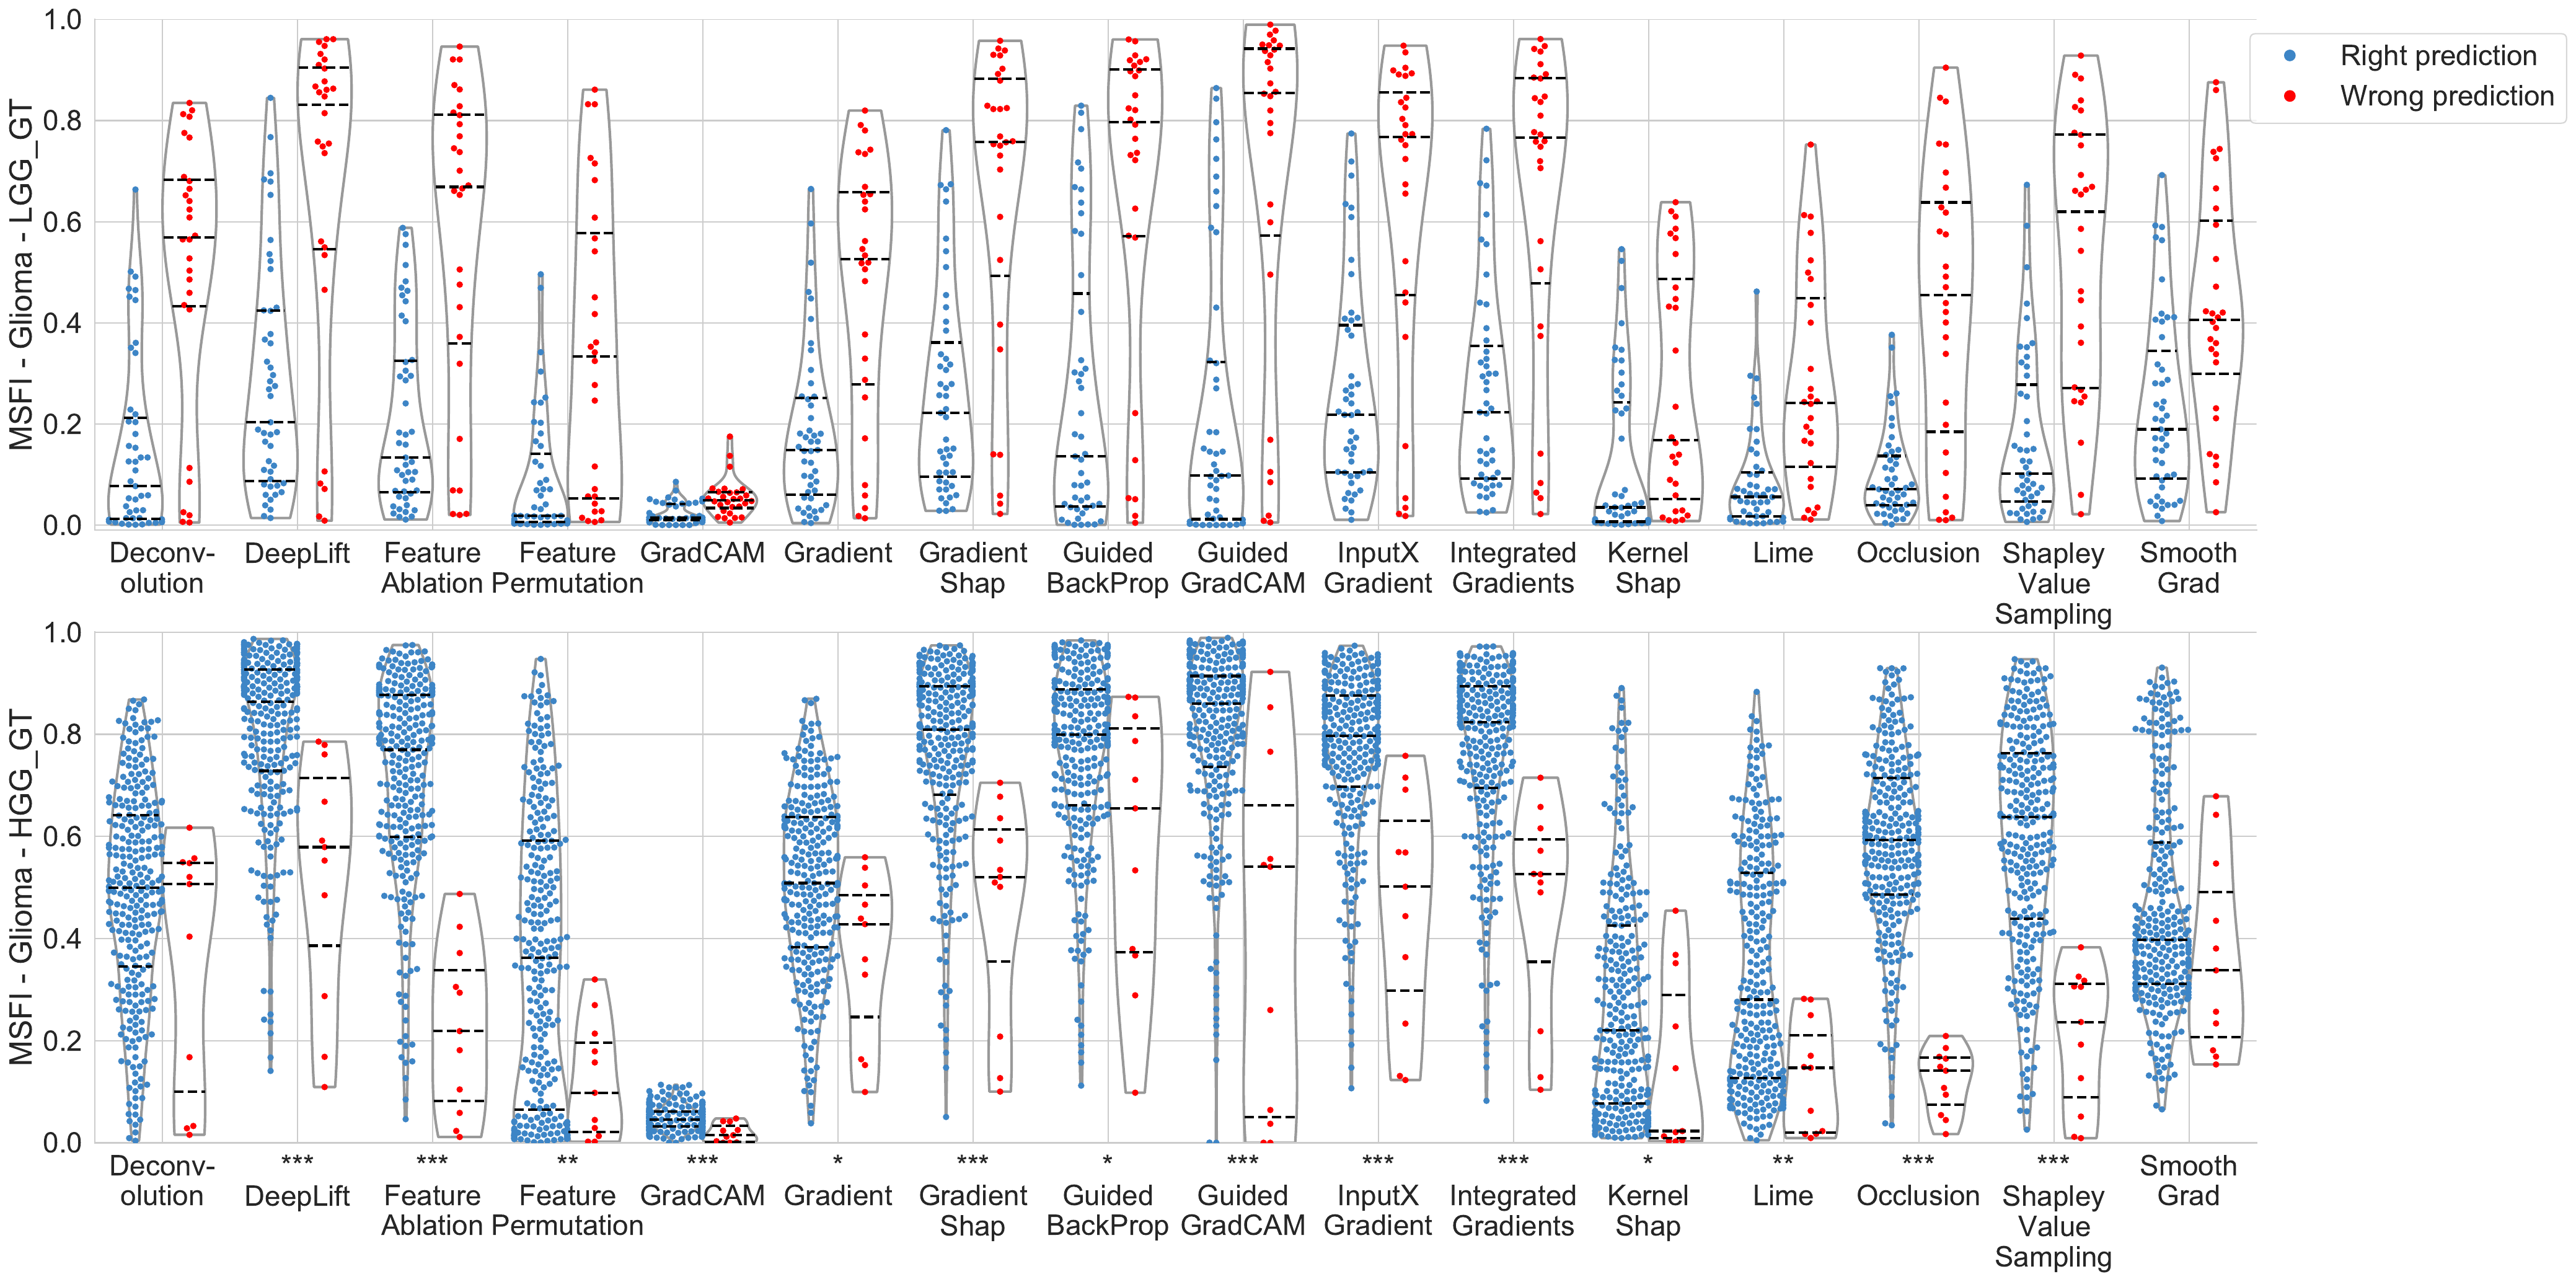}
    \caption{\textbf{MSFI distribution conditioned on the \textit{ground-truth} labels of LGG and HGG on glioma task.} The swarm and violin plots visualize MSFI distributions of right and wrong predictions conditioned on the ground-truth labels of LGG (top) and HGG (bottom), respectively.}
    \label{fig:class_conditioned_MSFI_gt}
\end{figure}
\FloatBarrier

For the knee task, when conditioned on the predicted labels (Fig.~\ref{fig:class_conditioned_MSFI_pred_knee}), all XAI methods did not show significant higher MSFI on correctly predicted data than incorrectly predicted one, for both positive and negative classes. When conditioned on the ground-truth labels (Fig.~\ref{fig:class_conditioned_MSFI_gt_knee}), some XAI methods showed significance, which can be explained by the MSFI distribution difference on different predicted classes.

\begin{figure}[!h]
    \centering
    \includegraphics[width=\textwidth]{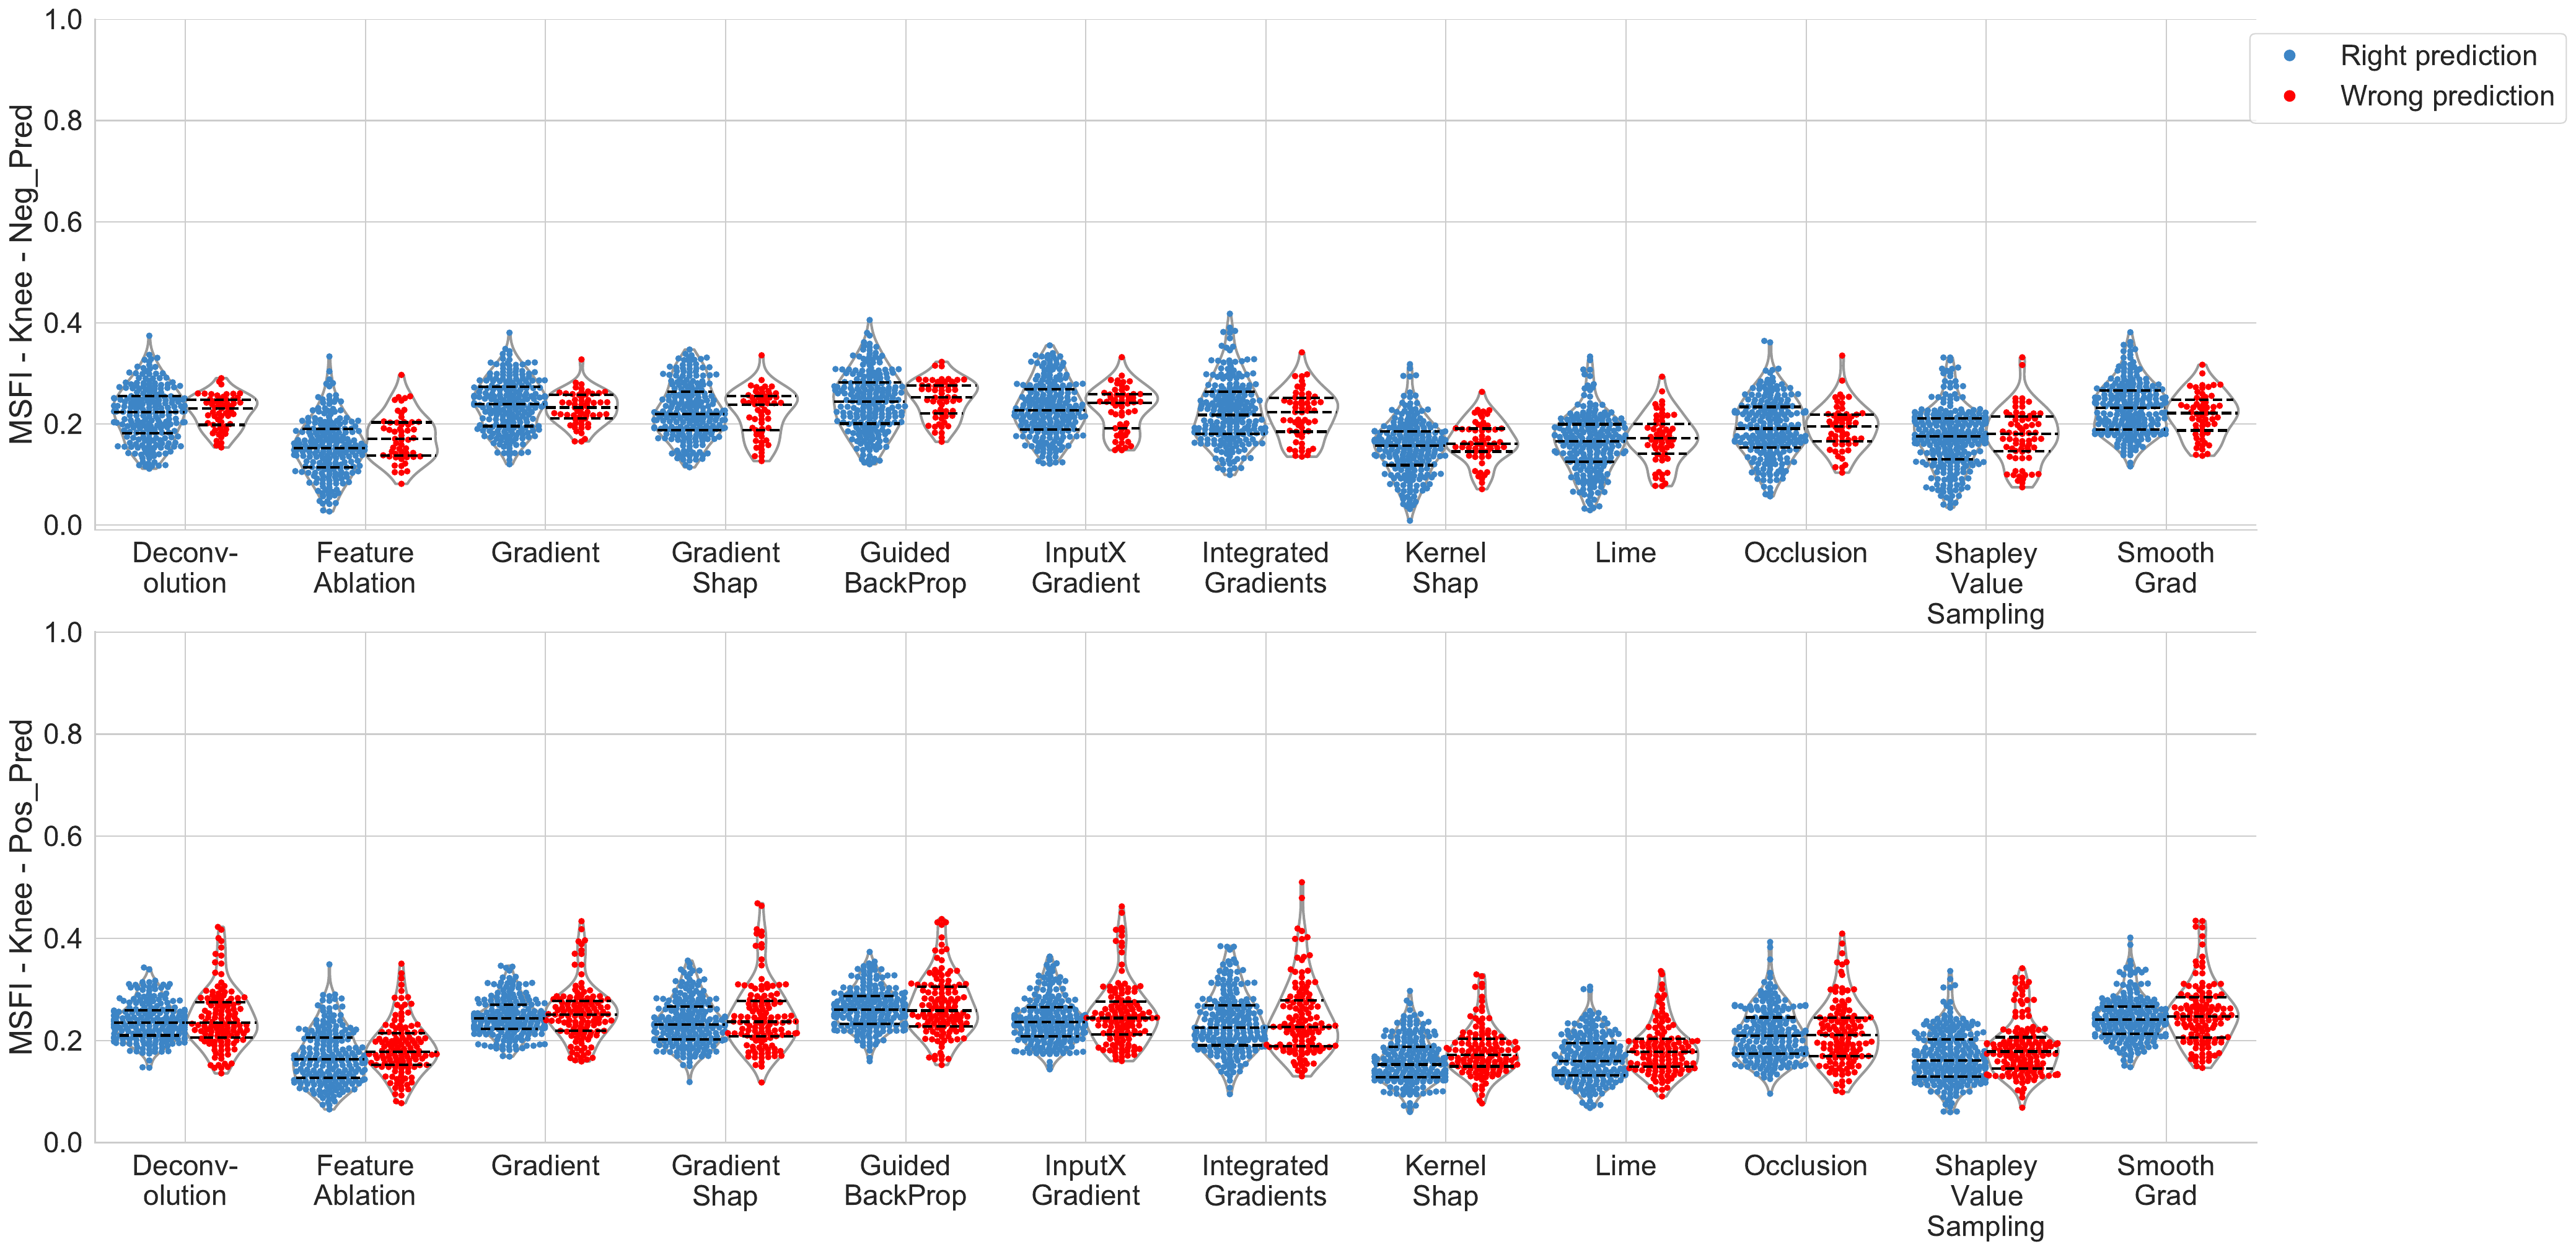}
    \caption{\textbf{MSFI distribution conditioned on the \textit{predicted} labels of negative and positive class on knee task.} The swarm and violin plots visualize MSFI distributions of right and wrong predictions conditioned on the predicted labels of negative (top) and positive class (bottom), respectively.}
    \label{fig:class_conditioned_MSFI_pred_knee}
\end{figure}
\FloatBarrier

\begin{figure}[!h]
    \centering
    \includegraphics[width=\textwidth]{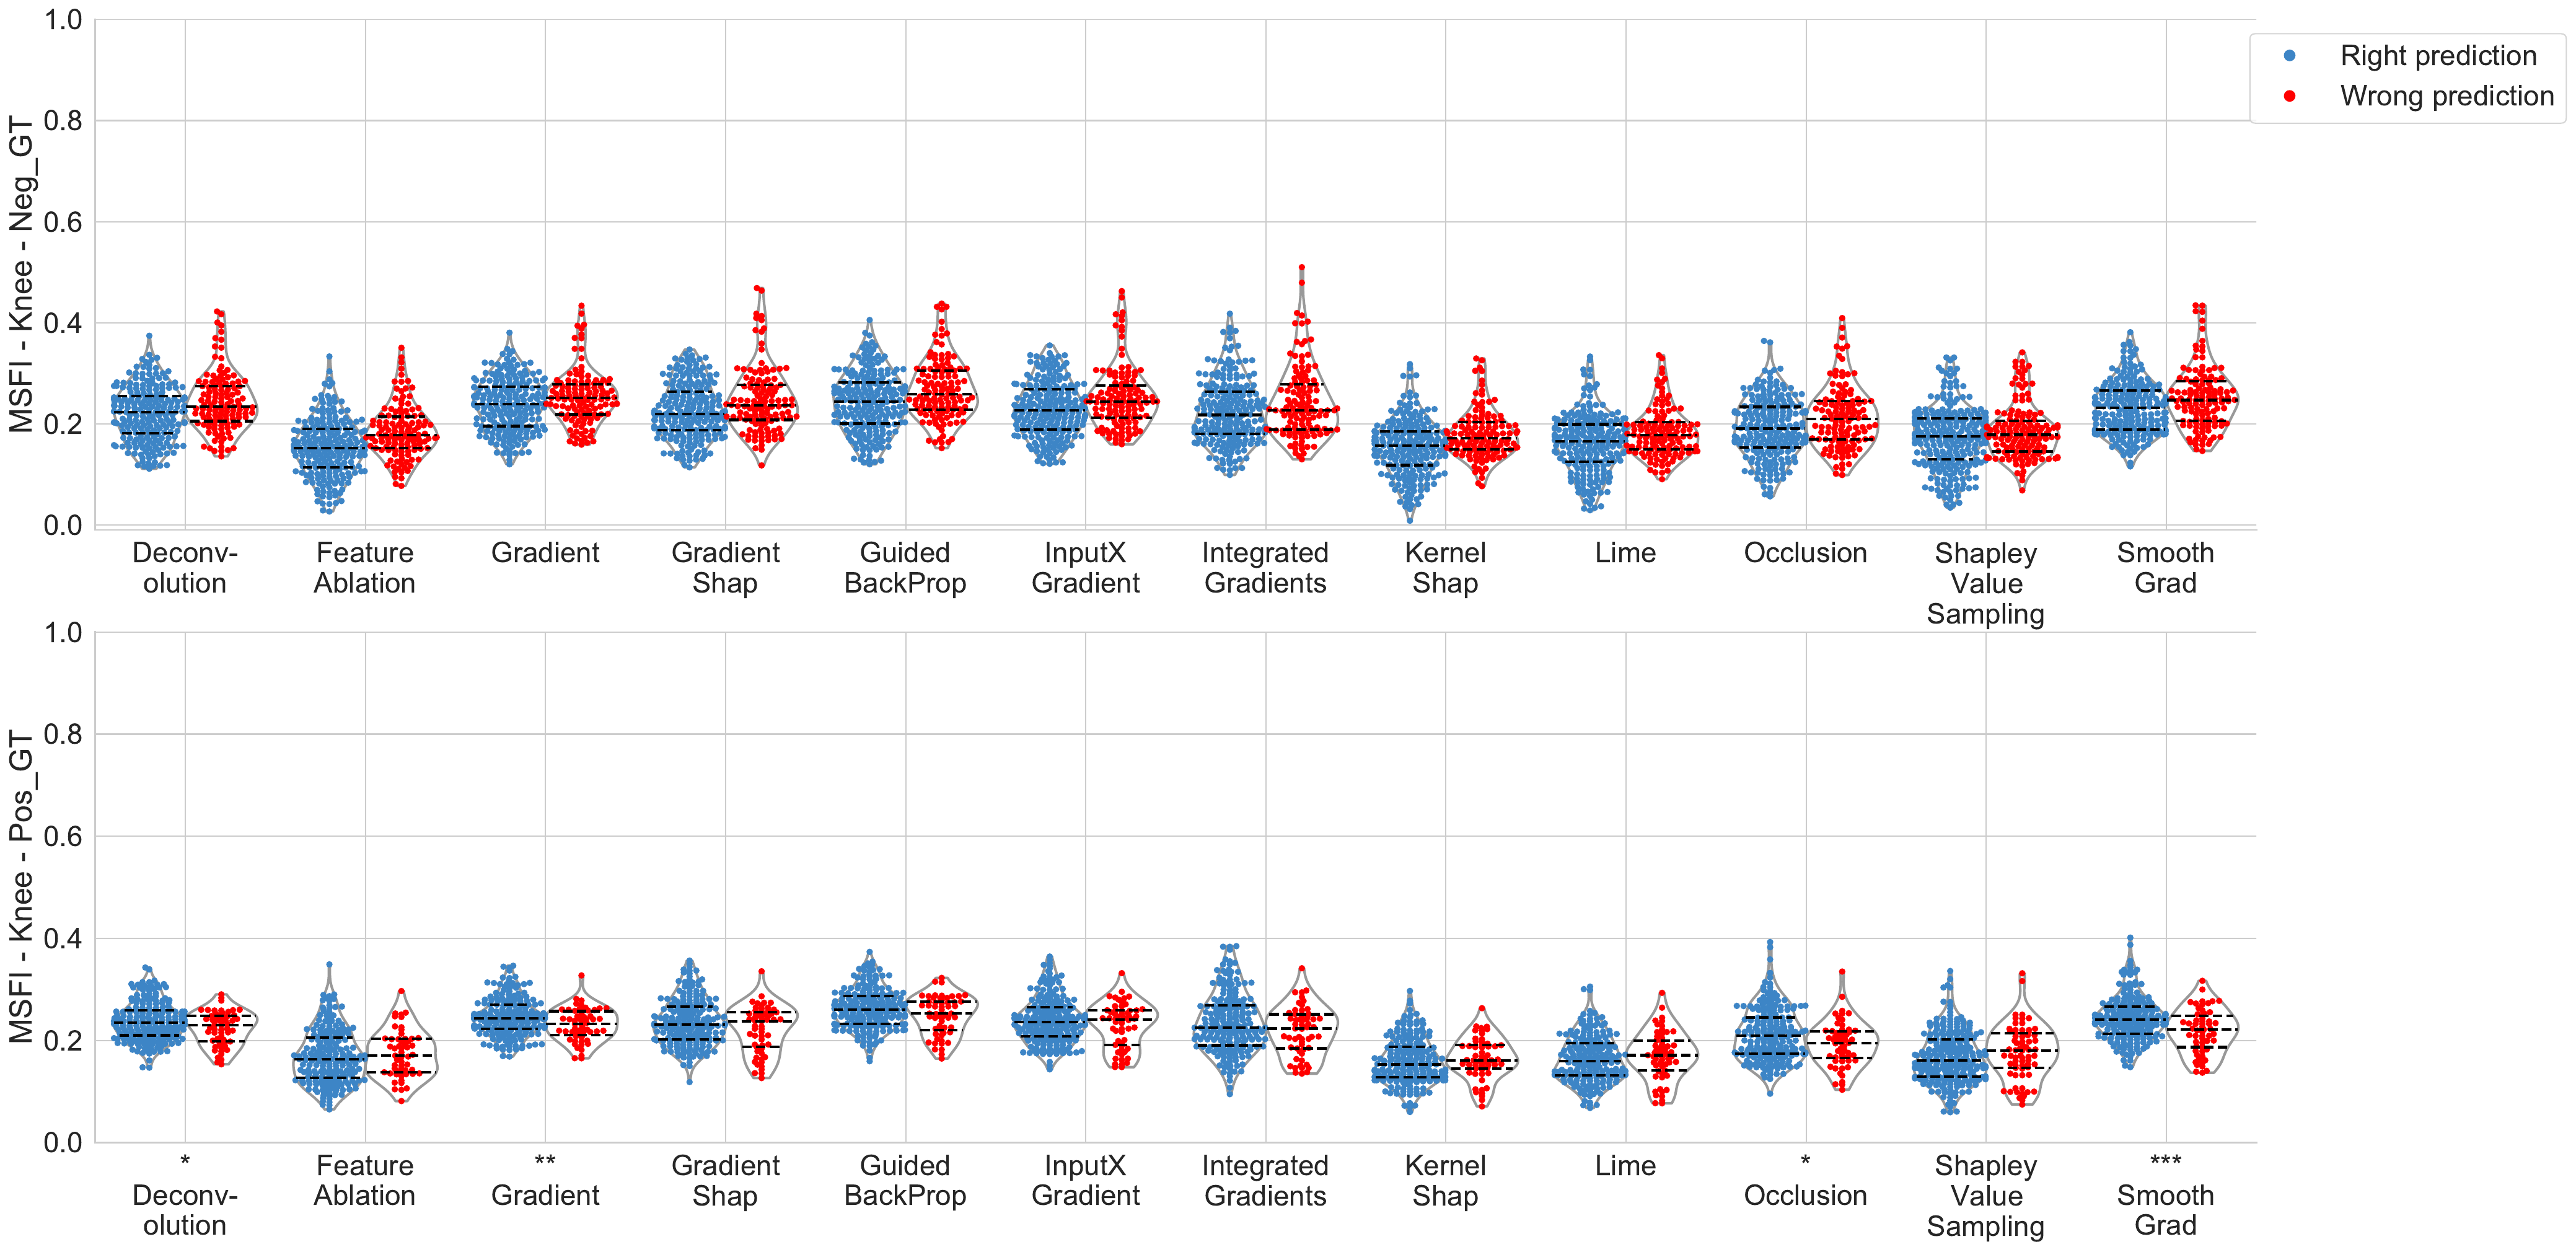}
    \caption{\textbf{MSFI distribution conditioned on the \textit{ground-truth} labels of negative and positive class on knee task.} The swarm and violin plots visualize MSFI distributions of right and wrong predictions conditioned on the ground-truth labels of negative (top) and positive class (bottom), respectively.}
    \label{fig:class_conditioned_MSFI_gt_knee}
\end{figure}
\FloatBarrier

Informative plausibility test conditioned on the predicted labels yielded similar results using FP metric, as shown in Fig.~\ref{fig:class_conditioned_FP_glioma_pred} on glioma, and Fig.~\ref{fig:class_conditioned_FP_knee_pred} on knee task.

\begin{figure}[!h]
    \centering
    \includegraphics[width=\textwidth]{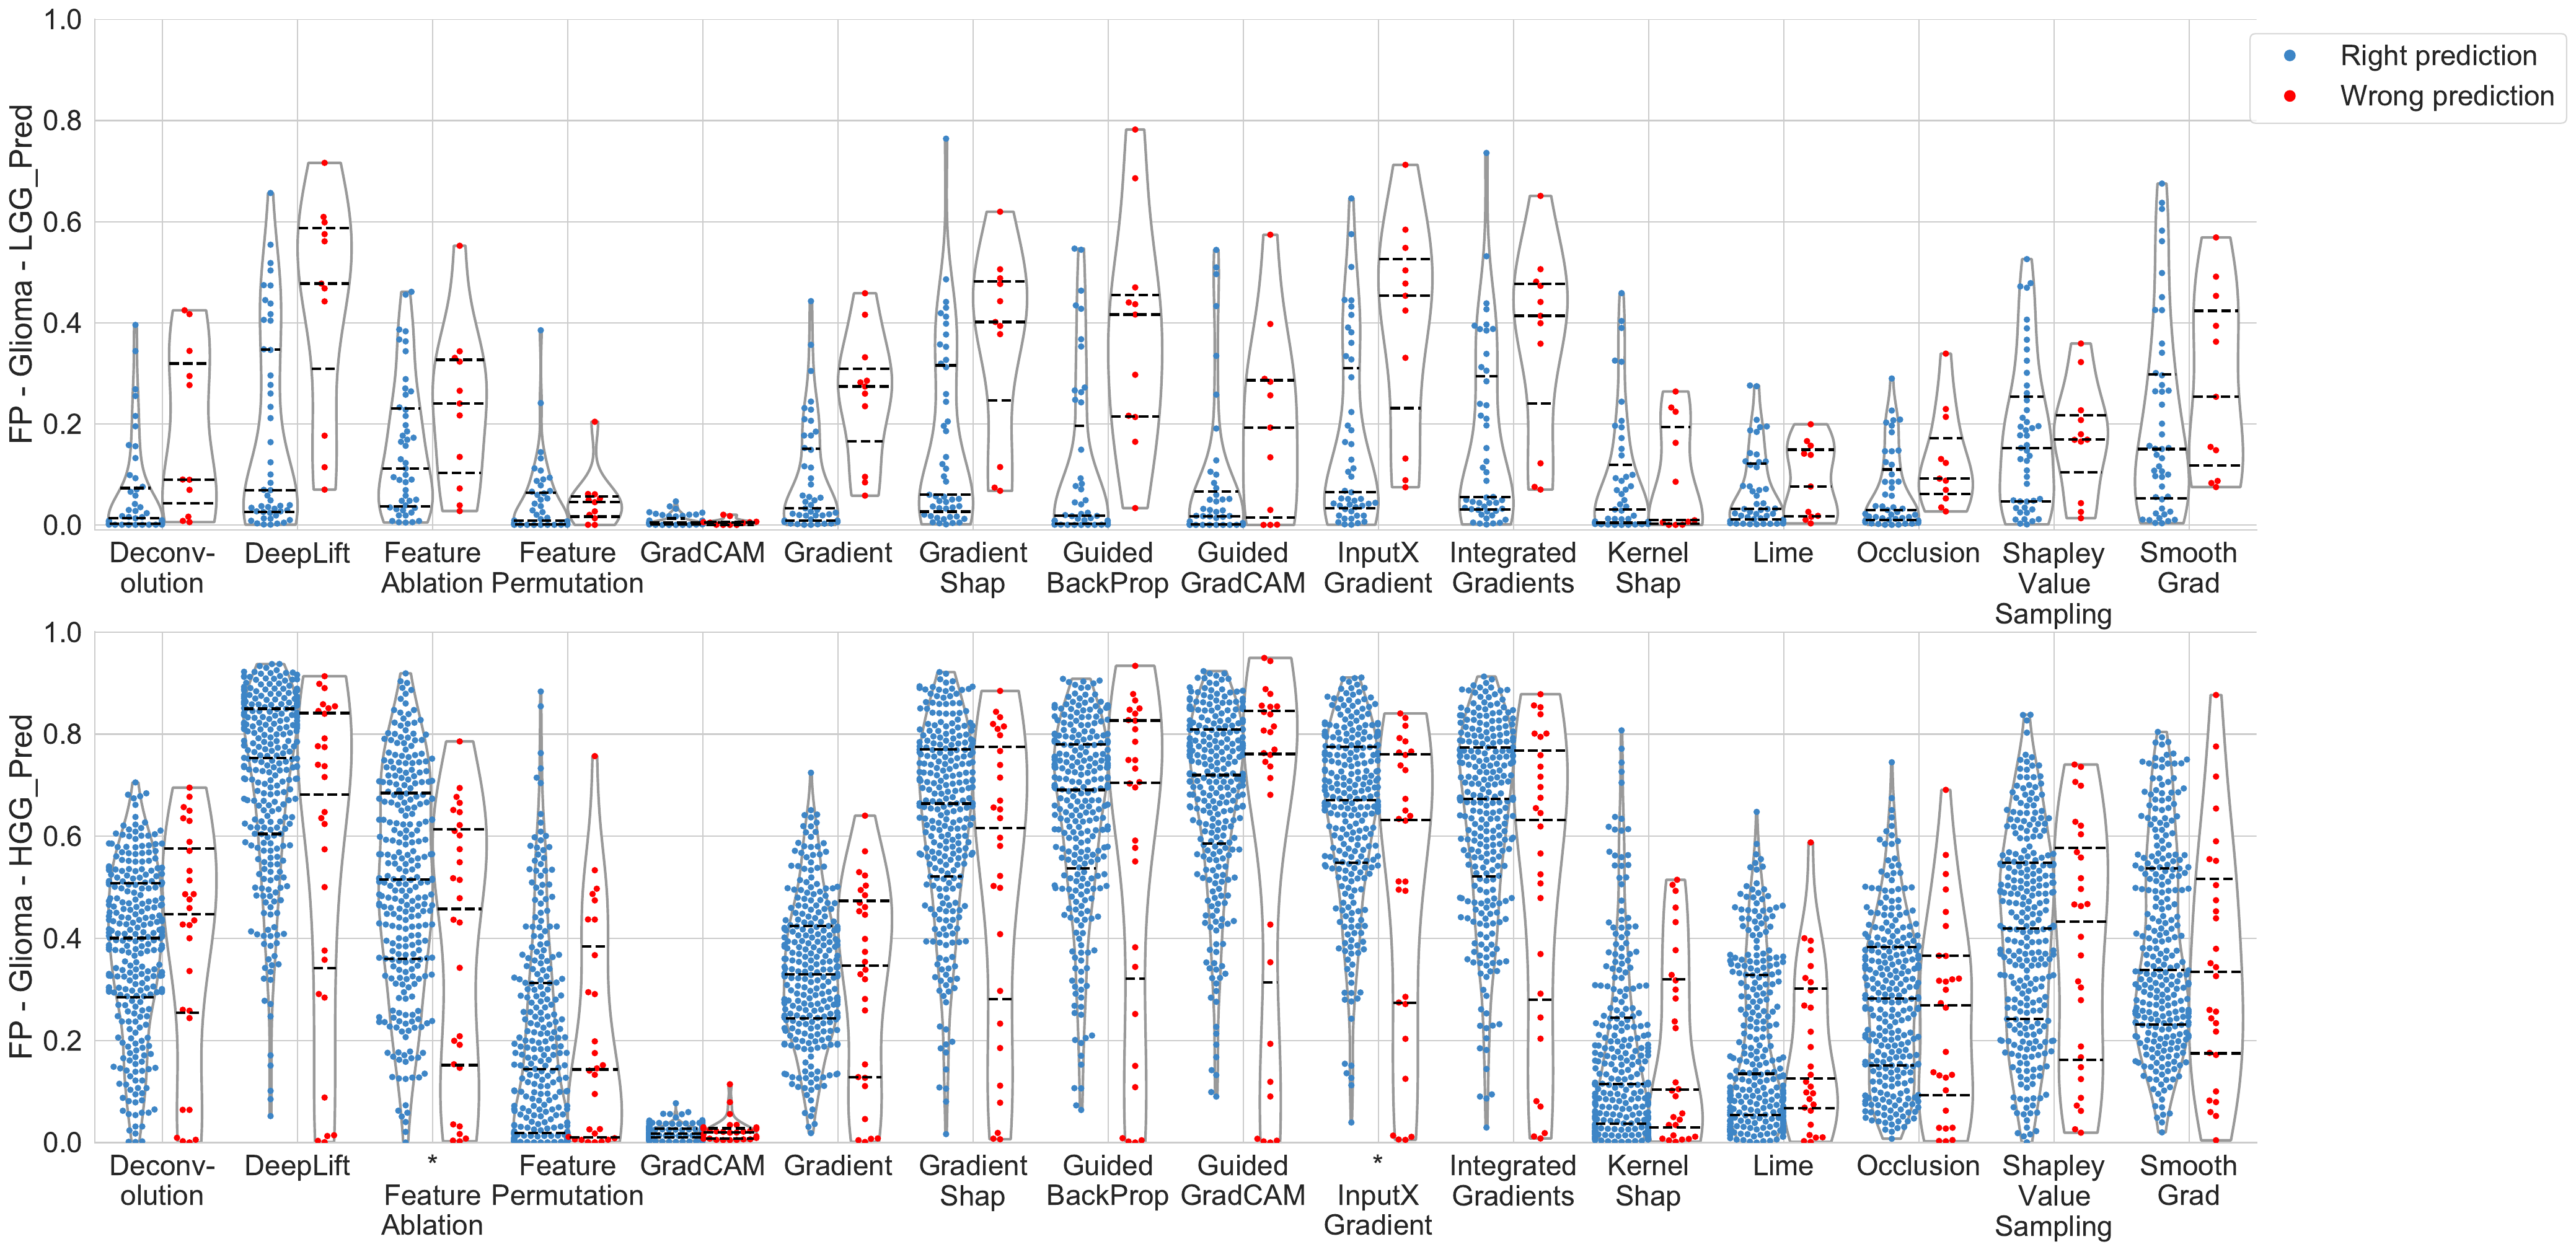}
    \caption{\textbf{FP distribution conditioned on the predicted labels of LGG and HGG on glioma task.} The swarm and violin plots visualize FP distributions of right and wrong predictions conditioned on the predicted labels of LGG (top) and HGG class (bottom), respectively.}
    \label{fig:class_conditioned_FP_glioma_pred}
\end{figure}
\FloatBarrier

\begin{figure}[!h]
    \centering
    \includegraphics[width=\textwidth]{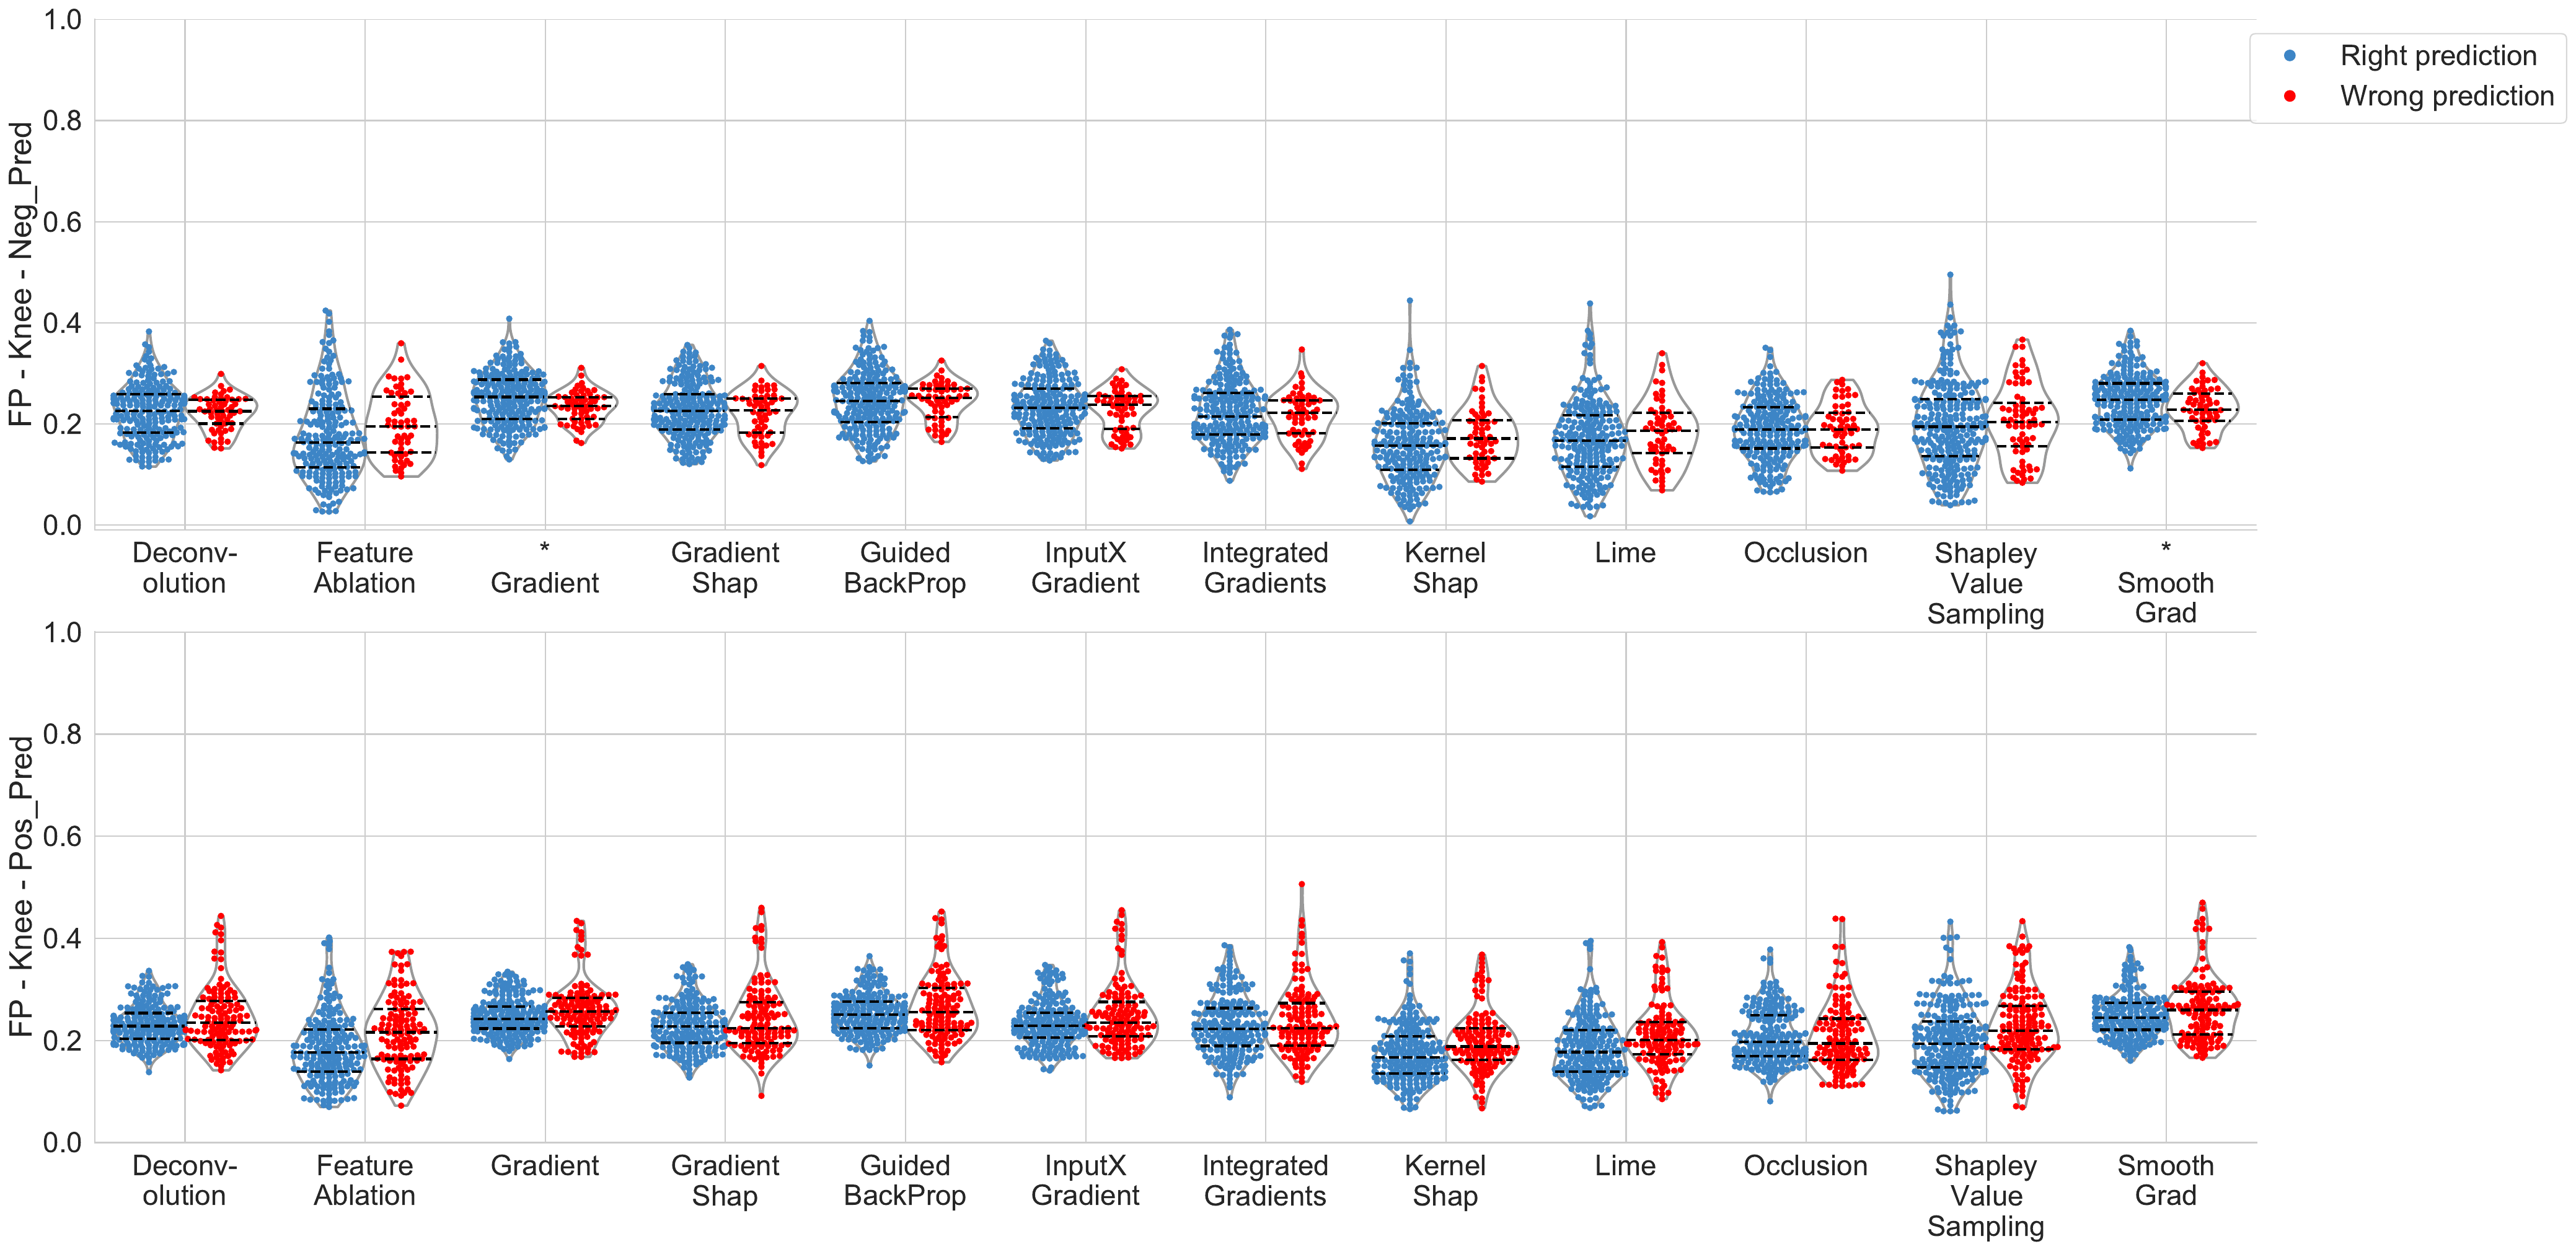}
    \caption{\textbf{FP distribution conditioned on the predicted labels of negative and positive class on knee task.} The swarm and violin plots visualize MSFI distributions of right and wrong predictions conditioned on the predicted labels of negative (top) and positive class (bottom), respectively.}
    \label{fig:class_conditioned_FP_knee_pred}
\end{figure}
\FloatBarrier
\section{Additional Figures}

\begin{figure*}[h]
\addcontentsline{toc}{subsection}{Correlation between Doctor Rating and the Plausibility Metrics}
    \centering
    \includegraphics[width=1
    \textwidth]{fig/dr rating corr.pdf}
    \caption{\textbf{Pearson's correlation between doctor rating and the plausibility metrics}. The scatter plot shows the correlation between doctor rating and MSFI scores (left), and between doctor rating and FP scores (right). Their regression lines are also indicated on the plots. MSFI slope = 0.36, FP slope = 0.25.
    Pearson's correlation between Doctor Rating and MSFI = 0.59, between Doctor Rating and FP = 0.57.}
    \label{fig:dr}
\end{figure*}
\FloatBarrier

\begin{figure*}%
\addcontentsline{toc}{subsection}{Heatmaps on the Glioma Task}
    \centering
    \subfloat[\centering  HGG]{{\includegraphics[width=\textwidth,height=\textheight,keepaspectratio]{fig/BraTS20_Training_070.pdf} }}%
    \qquad
    \subfloat[\centering LGG]{{\includegraphics[width=\textwidth,height=\textheight,keepaspectratio]{fig/BraTS20_Training_277.pdf} }}%
    \caption{\textbf{The evaluated 16 heatmaps on the glioma task.} Tumor feature segmentation map is marked as a green contour, and the modality importance is coded by the intensity of the mask contour. The model predicts correctly for both MRIs. We indicate the doctor rating, MSFI, and FP scores assessed on the 3D heatmaps, and visualize one 2D slice. Heatmaps are in the range of $[-1, 1]$, with redness and blueness representing the degree of feature importance and unimportance.}%
    \label{fig:hgg_lgg}%
\end{figure*}

\begin{figure*}%
\addcontentsline{toc}{subsection}{Heatmaps on the Knee Task}
    \centering
    \subfloat[\centering Meniscus tear]{{\includegraphics[width=\textwidth,height=\textheight,keepaspectratio]{fig/1184_cameraready.pdf} }}%
    \qquad
    \subfloat[\centering Intact]{{\includegraphics[width=\textwidth,height=\textheight,keepaspectratio]{fig/1182_cameraready.pdf} }}%
    \caption{\textbf{The evaluated 13 heatmaps on the knee task.} Meniscus bounding boxes are marked as green contours, and the modality importance is coded by the intensity of the bounding box contour. The model predicts correctly for both MRIs. We indicate MSFI and FP scores assessed on the 3D heatmaps, and visualize one 2D slice. Heatmaps are in the range of $[0, 1]$, with redness representing the degree of feature importance.}%
    \label{fig:example}%
\end{figure*}

\begin{figure*}[h]
\addcontentsline{toc}{subsection}{Synthesized Multi-Modal Glioma MRI}
    \centering
    \includegraphics[width=0.8\linewidth]{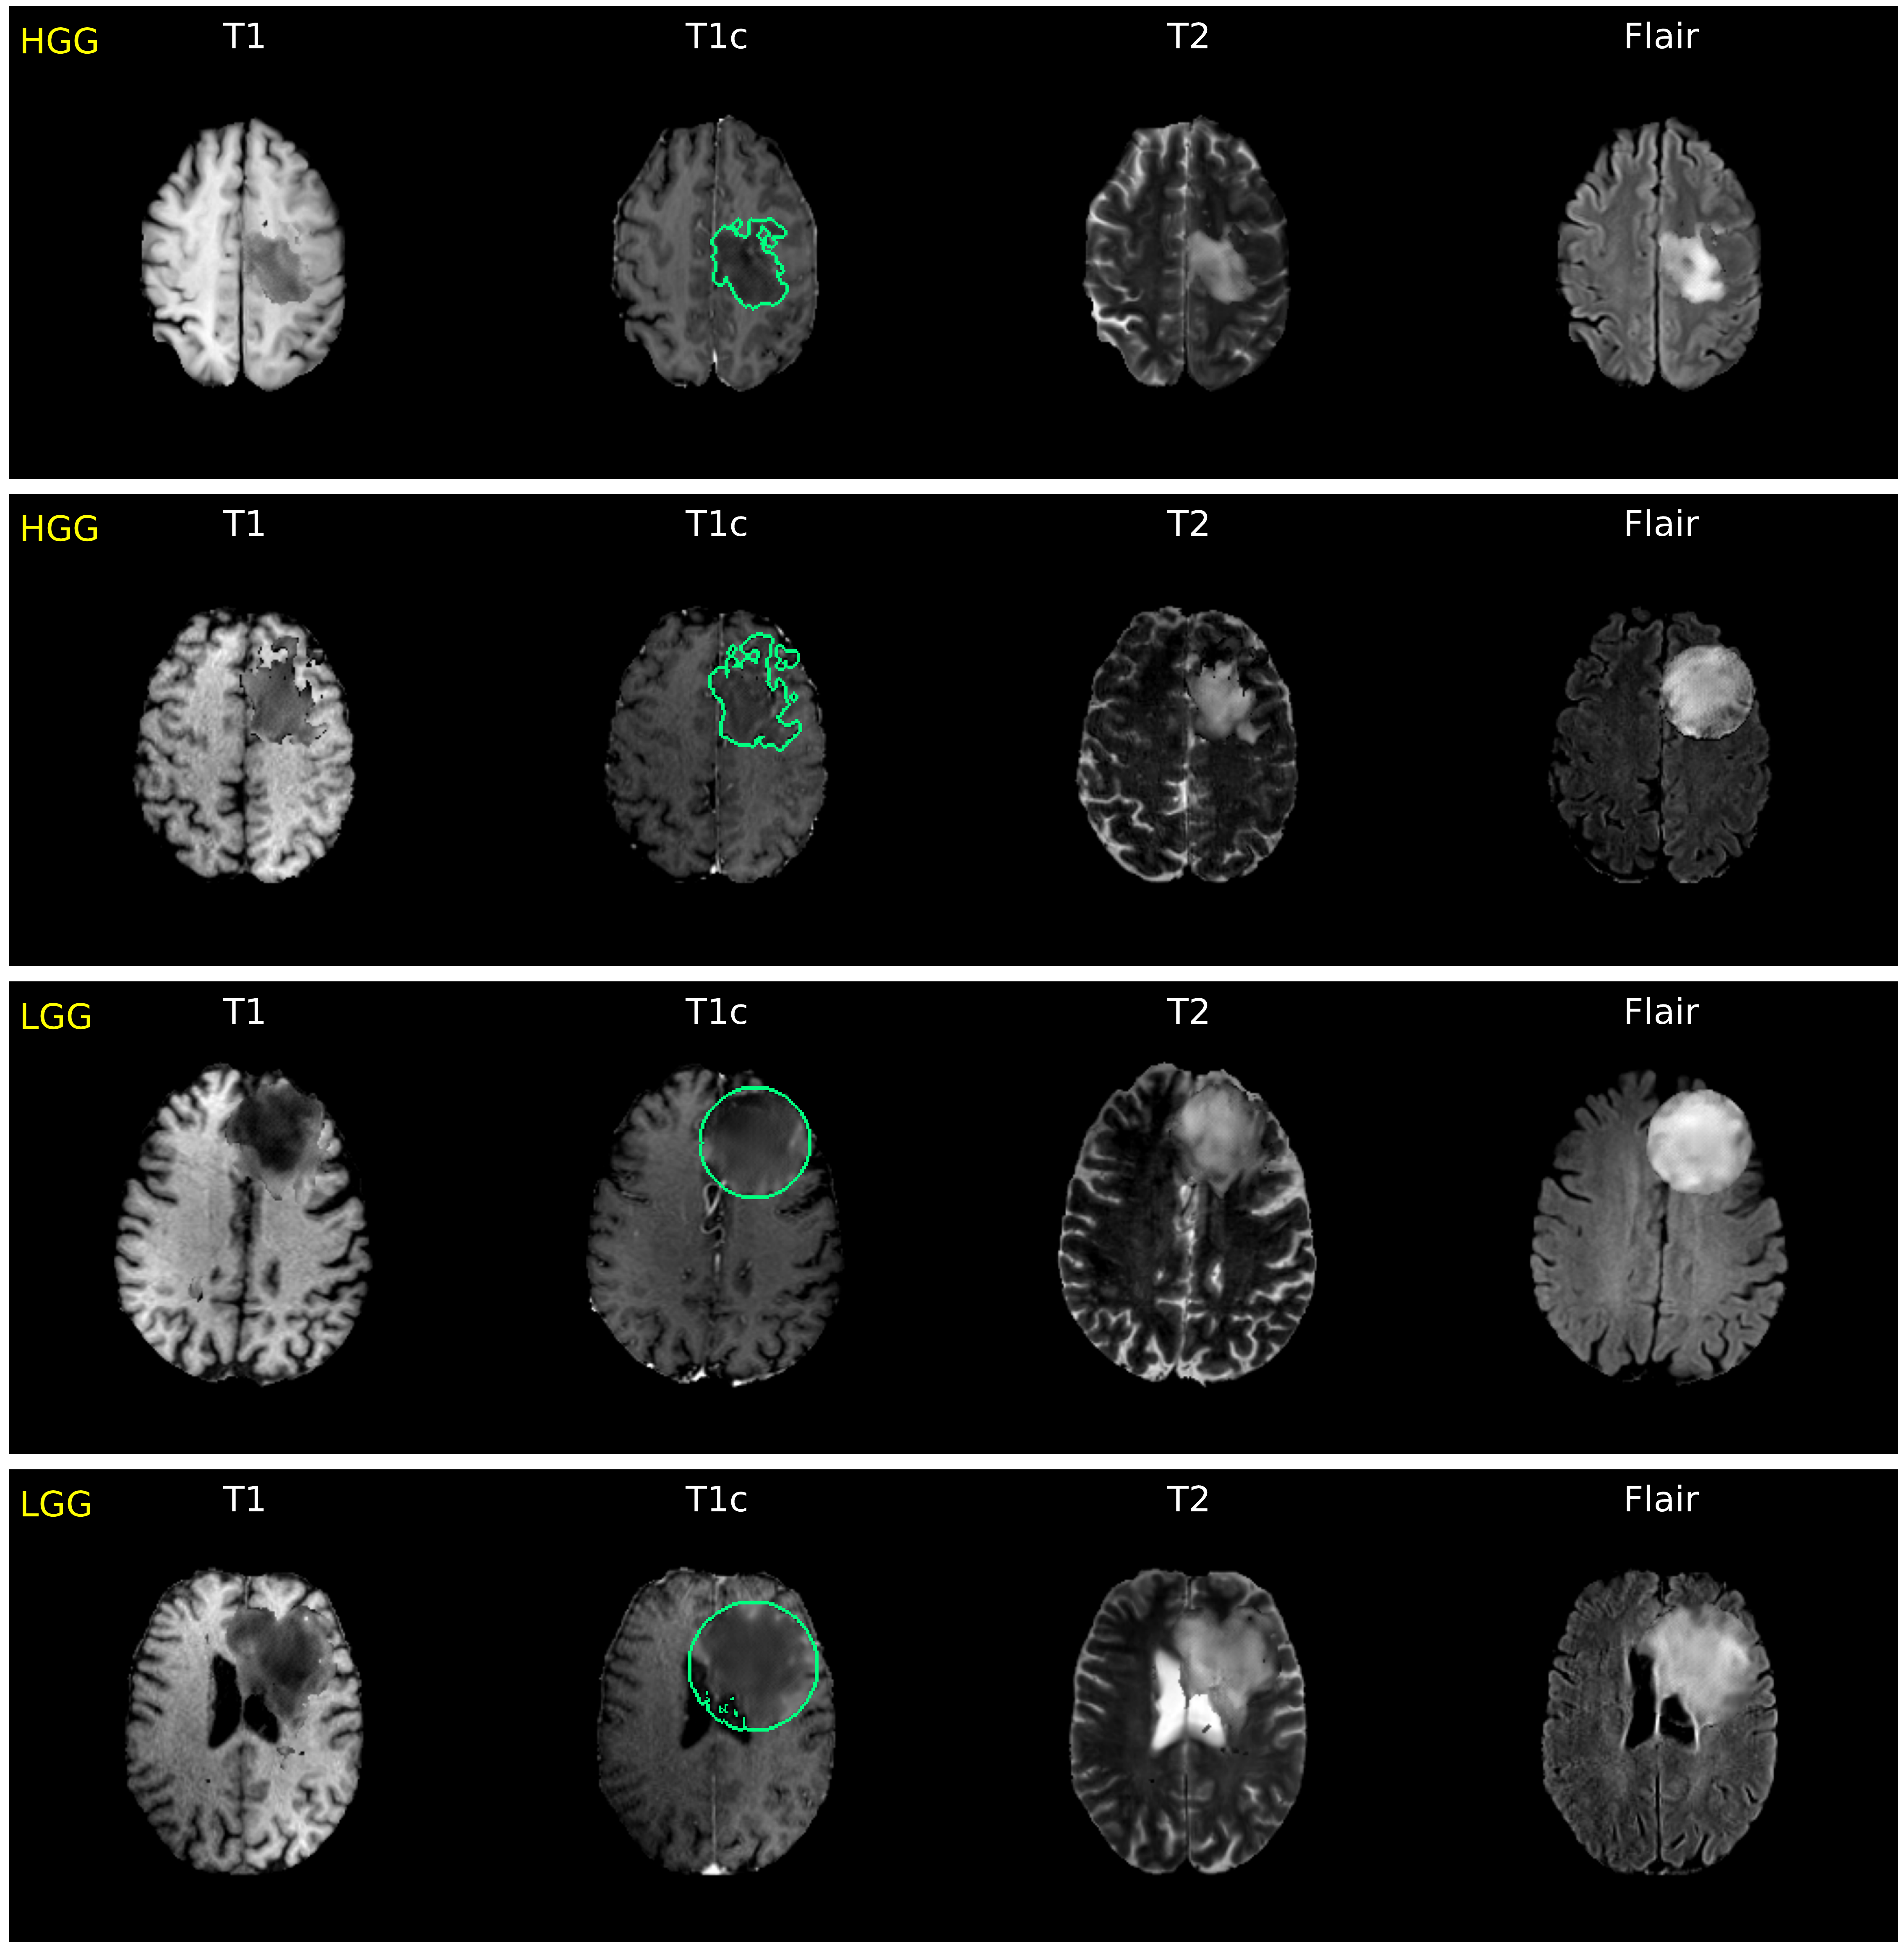}
    \caption{\textbf{The synthesized 2D multi-modal glioma MRI}. The label of HGG and LGG corresponds to tumor shapes on T1C modality, with the tumor shape outlined in the segmentation mask (LGG: round; HGG: irregular). The Flair modality has 70\% alignment with the label, while T1 and T2 modalities are not associated with the tumor grade label.}
    \label{fig:hm}
\end{figure*}

\begin{figure*}%
\addcontentsline{toc}{subsection}{Heatmaps on the Synthetic Glioma Task}
    \centering
    \subfloat[\centering  HGG]{{\includegraphics[width=\textwidth,height=\textheight,keepaspectratio]{fig/58_71.pdf} }}%
    \qquad
    \subfloat[\centering HGG]{{\includegraphics[width=\textwidth,height=\textheight,keepaspectratio]{fig/3_65.pdf} }}%
    \caption{\textbf{The evaluated 16 heatmaps on the synthetic glioma dataset/models.} The heatmaps are in the range of $[0, 1]$, with redness representing the degree of feature importance.}%
    \label{fig:example}%
\end{figure*}

\begin{figure*}[h]%
    \centering
    \subfloat[\centering  LGG]{{\includegraphics[width=\textwidth,height=\textheight,keepaspectratio]{fig/81_50.pdf} }}%
    \qquad
    \subfloat[\centering LGG]{{\includegraphics[width=\textwidth,height=\textheight,keepaspectratio]{fig/105_46.pdf} }}%
    \caption{cont. \textbf{The evaluated 16 heatmaps on the synthetic glioma dataset/models.}}%
    \label{fig:example}%
\end{figure*}

\clearpage

\bibliography{xai_eval,xai_eval_202111}
\bibliographystyle{plain}

\end{document}
